# Supplementary material for: Moniqua: Modulo Quantized Communication in Decentralized SGD
Source: arXiv:2002.11787 source file (2020-06-30)
Supplement: Supplementary file 1 [file lowfre_Sync.tex]

\subsection{Low Frequency on D-PSGD}
From a local view, the update rule of $\eta$ frequency communication can be written as
\begin{displaymath}
	x_{k+1,i} \leftarrow x_{k,i} + \sum\nolimits_{j\in\mathcal{N}_i}\left(q_{k,j} - q_{k,i}\right)\widetilde{W}_{ji} - \alpha \widetilde{g}_{k,i}
\end{displaymath}
which is equivalent to
\begin{equation}
x_{k+1,i} = x_{k,i} +  \sum_{j=1}^{n}\left(x_{k,j} - x_{k,i}\right)\widetilde{W}_{ji} - \alpha \widetilde{g}_{k,i} +  \sum_{j=1}^{n}\left((q_{k,j} - x_{k,j}) - (q_{k,i} - x_{k,i})\right)\widetilde{W}_{ji}
\end{equation}
From a global view, the update rule can be written as
\begin{equation}
{X}_{k+1} = X_k + Q_k(\widetilde{W}-I) - \alpha \widetilde{G}_k= X_k\widetilde{W} - \alpha \widetilde{G}_k + (Q_k-X_k)(\widetilde{W}-I)
\end{equation}
Since change of communication frequency will only change to the terms in the proof of Moniqua that relate to the communication, we can reuse the intermediate result from Moniqua as
\begin{align*}
\frac{1 - \alpha L}{K}\sum_{k=0}^{K-1}\mathbb{E}\left\|\overline{G}_k\right\|^2 + \frac{1}{K}\sum_{k=0}^{K-1}\mathbb{E}\left\|\nabla f(\overline{X}_k)\right\|^2\leq \frac{2(f(0) - f^*)}{\alpha K} + \frac{\alpha L}{n}\sigma^2 + \frac{ L^2}{nK}\sum_{k=0}^{K-1}\sum_{i=1}^{n}\mathbb{E}\left\|\overline{X}_k - x_{k,i}\right\|^2
\end{align*}
And similar to Moniqua, we have
\begin{align*}
&\sum_{k=0}^{K-1}\sum_{i=1}^{n}\mathbb{E}\left\|\overline{X}_k - x_{k,i}\right\|^2\\
\overset{x_{0,i}=0}{=} & \sum_{k=1}^{K-1}\sum_{i=1}^{n}\mathbb{E}\left\|X_k\left(\frac{\mathbbm{1}_n}{n} - e_i\right)\right\|^2\\
= & \sum_{k=1}^{K-1}\sum_{i=1}^{n}\mathbb{E}\left\|\left(X_{k-1}\widetilde{W} - \alpha \widetilde{G}_{k-1} +  \Omega_{k-1}\right)\left(\frac{\mathbbm{1}_n}{n} - e_i\right)\right\|^2\\
= &\sum_{k=1}^{K-1}\sum_{i=1}^{n}\mathbb{E}\left\|\sum_{t=0}^{k-1}\left(-\alpha \widetilde{G}_t +  \Omega_t\right)\left(\frac{\mathbbm{1}_n}{n} - \widetilde{W}^{k-t-1}e_i\right)\right\|^2\\
\leq & 2\alpha^2\sum_{k=1}^{K-1}\sum_{i=1}^{n}\mathbb{E}\left\|\sum_{t=0}^{k-1}\widetilde{G}_t\left(\frac{\mathbbm{1}_n}{n}-\widetilde{W}^{k-t-1}e_i\right)\right\|^2 + 2\sum_{k=1}^{K-1}\sum_{i=1}^{n}\mathbb{E}\left\|\sum_{t=0}^{k-1}\Omega_t\left(\frac{\mathbbm{1}_n}{n} - \widetilde{W}^{k-t-1}e_i\right)\right\|^2\\
= & 2\alpha^2\sum_{k=1}^{K-1}\mathbb{E}\left\|\sum_{t=0}^{k-1}\widetilde{G}_t\left(\frac{\mathbbm{1}_n\mathbbm{1}_n^\top}{n}-\widetilde{W}^{k-t-1}\right)\right\|^2_F + 2\sum_{k=1}^{K-1}\mathbb{E}\left\|\sum_{t=0}^{k-1}\Omega_t\left(\frac{\mathbbm{1}_n\mathbbm{1}_n^\top}{n} - \widetilde{W}^{k-t-1}\right)\right\|^2_F\\
\leq &2\alpha ^2\sum_{k=1}^{K-1}\mathbb{E}\left(\sum_{t=0}^{k-1}\rho ^{\left\lfloor\frac{k-t-1}{\mathcal{T}}\right\rfloor}\left\|\widetilde{G}_t\right\|_F\right)^2 + 2\sum_{k=1}^{K-1}\mathbb{E}\left(\sum_{t=0}^{k-1}\rho ^{\left\lfloor\frac{k-t-1}{\mathcal{T}}\right\rfloor}\left\|\Omega_t\right\|_F\right)^2\\
\leq & \frac{2\alpha ^2\mathcal{T}^2}{(1-\rho )^2}\sum_{k=1}^{K-1}\mathbb{E}\left\|\widetilde{G}_k\right\|^2_F + \frac{2\mathcal{T}^2}{(1-\rho )^2}\sum_{k=1}^{K-1}\mathbb{E}\left\|\Omega_k\right\|^2_F\\
\leq & \frac{2\alpha ^2\mathcal{T}^2}{(1-\rho )^2}\left(n\sigma^2K + 3L^2\sum_{k=0}^{K-1}\sum_{i=1}^{n}\mathbb{E}\left\|\overline{X}_k - x_{k,i}\right\|^2 + 3n\varsigma^2K + 3n\sum_{k=0}^{K-1}\mathbb{E}\left\|\nabla f(\overline{X}_k)\right\|^2\right) + \frac{2\mathcal{T}^2}{(1-\rho )^2}\sum_{k=1}^{K-1}\mathbb{E}\left\|\Omega_k\right\|^2_F
\end{align*}
%\end{displaymath}
Rearrange the terms, we have
%\begin{displaymath}
\begin{align*}
	& \left(1 - \frac{6\alpha^2\mathcal{T}^2L^2}{(1-\rho)^2}\right)\sum_{k=0}^{K-1}\sum_{i=1}^{n}\mathbb{E}\left\|\overline{X}_k - x_{k,i}\right\|^2\\
	\leq & \frac{2\alpha^2\mathcal{T}^2}{(1-\rho)^2}\left(n\sigma^2K + 3n\varsigma^2K + 3n\sum_{k=0}^{K-1}\mathbb{E}\left\|\nabla f(\overline{X}_k)\right\|^2\right) + \frac{2\mathcal{T}^2}{(1-\rho )^2}\sum_{k=1}^{K-1}\mathbb{E}\left\|\Omega_k\right\|^2_F
\end{align*}
%\end{displaymath}
Let $M_1 = 1 - \frac{6\alpha^2\mathcal{T}^2L^2}{(1-\rho)^2}>0$, we have
\begin{displaymath}
	\sum_{k=0}^{K-1}\sum_{i=1}^{n}\mathbb{E}\left\|\overline{X}_k - x_{k,i}\right\|^2\leq \frac{2\alpha^2\mathcal{T}^2}{M_1(1-\rho)^2}\left(n\sigma^2K + 3n\varsigma^2K + 3n\sum_{k=0}^{K-1}\mathbb{E}\left\|\nabla f(\overline{X}_k)\right\|^2\right) + \frac{2\mathcal{T}^2}{M_1(1-\rho )^2}\sum_{k=1}^{K-1}\mathbb{E}\left\|\Omega_k\right\|^2_F
\end{displaymath}
And
\begin{displaymath}
	\frac{L^2}{nK}\sum_{k=0}^{K-1}\sum_{i=1}^{n}\mathbb{E}\left\|\overline{X}_k - x_{k,i}\right\|^2\leq \frac{2\alpha^2\mathcal{T}^2L^2}{M_1(1-\rho)^2}\left(\sigma^2 + 3\varsigma^2 + \frac{3}{K}\sum_{k=0}^{K-1}\mathbb{E}\left\|\nabla f(\overline{X}_k)\right\|^2\right) + \frac{2\mathcal{T}^2L^2}{M_1nK(1-\rho )^2}\sum_{k=1}^{K-1}\mathbb{E}\left\|\Omega_k\right\|^2_F
\end{displaymath}
Pushing it back we obtain
\begin{align*}
&\frac{1 - \alpha L}{K}\sum_{k=0}^{K-1}\mathbb{E}\left\|\overline{G}_k\right\|^2 + \frac{1}{K}\sum_{k=0}^{K-1}\mathbb{E}\left\|\nabla f(\overline{X}_k)\right\|^2\\
\leq & \frac{2(f(0) - f^*)}{\alpha K} + \frac{\alpha L}{n}\sigma^2 + \frac{2\alpha^2\mathcal{T}^2L^2}{M_1(1-\rho)^2}\left(\sigma^2 + 3\varsigma^2 + \frac{3}{K}\sum_{k=0}^{K-1}\mathbb{E}\left\|\nabla f(\overline{X}_k)\right\|^2\right) + \frac{2\mathcal{T}^2L^2}{M_1nK(1-\rho )^2}\sum_{k=1}^{K-1}\mathbb{E}\left\|\Omega_k\right\|^2_F
\end{align*}
where
\begin{displaymath}
M_1 = 1-\frac{6\alpha^2\mathcal{T}^2L^2}{(1-\rho)^2}
\end{displaymath}
Rearrange the terms, we get
%\begin{displaymath}
\begin{align*}
& \frac{1 - \alpha L}{K}\sum_{k=0}^{K-1}\mathbb{E}\left\|\overline{G}_k\right\|^2 + \left(1-\frac{6\alpha^2\mathcal{T}^2L^2}{M_1(1-\rho)^2}\right)\frac{1}{K}\sum_{k=0}^{K-1}\mathbb{E}\left\|\nabla f(\overline{X}_k)\right\|^2\\
\leq & \frac{2(f(0) - f^*)}{\alpha K} + \frac{\alpha L}{n}\sigma^2 +  \frac{2\alpha^2\mathcal{T}^2L^2\left(\sigma^2 + 3\varsigma^2\right)}{M_1(1-\rho)^2} + \frac{2\mathcal{T}^2L^2}{M_1nK(1-\rho )^2}\sum_{k=1}^{K-1}\mathbb{E}\left\|\Omega_k\right\|^2_F
\end{align*}
%\end{displaymath}
Let
\begin{displaymath}
M_2 = 1-\frac{6\alpha^2\mathcal{T}^2L^2}{M_1(1-\rho)^2}
\end{displaymath}
we get
%\begin{displaymath}
\begin{align*}
	& \frac{1 - \alpha L}{K}\sum_{k=0}^{K-1}\mathbb{E}\left\|\overline{G}_k\right\|^2 + \frac{M_2}{K}\sum_{k=0}^{K-1}\mathbb{E}\left\|\nabla f(\overline{X}_k)\right\|^2\\
	\leq & \frac{2(f(0) - f^*)}{\alpha K} + \frac{\alpha L}{n}\sigma^2 +  \frac{2\alpha^2\mathcal{T}^2L^2\left(\sigma^2 + 3\varsigma^2\right)}{M_1(1-\rho)^2} + \frac{2\mathcal{T}^2L^2}{M_1nK(1-\rho )^2}\sum_{k=1}^{K-1}\mathbb{E}\left\|\Omega_k\right\|^2_F
\end{align*}
Since the $\Omega_k$ term is the same as Moniqua, pushing it to the $\Omega_k$, and let $M_1, M_2\geq\frac{1}{2}$ we have
\begin{displaymath}
	\frac{1}{K}\sum_{k=0}^{K-1}\mathbb{E}\left\|\nabla f(\overline{X}_k)\right\|^2\leq \frac{4(f(0) - f^*)}{\alpha K} + \frac{2\alpha L}{n}\sigma^2 +  \frac{8\alpha^2\mathcal{T}^2L^2\left(\sigma^2 + 3\varsigma^2\right)}{(1-\rho)^2} + \frac{8\alpha^2\mathcal{T}^2B^2L^2}{(1-\rho )^2}
\end{displaymath}
By setting $\alpha=\frac{1}{\varsigma^{\frac{2}{3}}K^{\frac{1}{3}}+\sigma\sqrt{\frac{K}{n}}+2L}$, we have
\begin{align*}
& \frac{1}{K}\sum_{k=0}^{K-1}\mathbb{E}\left\|\nabla f(\overline{X}_k)\right\|^2\\
\leq &  \frac{4\sigma(f(0) - f^* + L/2)}{\sqrt{nK}} +  \frac{4\varsigma^{\frac{2}{3}}(f(0)-f^*)}{K^{\frac{2}{3}}}+  \frac{8\mathcal{T}^2L^2n}{(1-\rho)^2K} + \frac{24\mathcal{T}^2L^2\varsigma^{\frac{2}{3}}}{(1-\rho)^2K^{\frac{2}{3}}}+ \frac{8B^2\mathcal{T}^2L^2n}{(1-\rho)^2\sigma^2K}\\
\lesssim & \frac{\sigma}{\sqrt{nK}} + \frac{\varsigma^{\frac{2}{3}}\mathcal{T}^2}{K^{\frac{2}{3}}} + \frac{n\mathcal{T}^2}{K} + \frac{nB^2\mathcal{T}^2}{\sigma^2K}\\
=&\frac{\sigma}{\sqrt{nK}} + \frac{\varsigma^{\frac{2}{3}}}{\eta^2K^{\frac{2}{3}}} + \frac{n}{\eta^2K} + \frac{nB^2}{\eta^2\sigma^2K}
\end{align*}
Now we can see the dependency of asymptotic rate on $eta$.
