# Supplementary material for: Moniqua: Modulo Quantized Communication in Decentralized SGD
Source: arXiv:2002.11787 source file (2020-06-30)
Supplement: Supplementary file 2 [file Moniqua_supplementary_arxiv.pdf]

---

# Supplementary Material

---

## A Overview

This supplementary material contains proof, pseudo code and extra experimental results of Moniqua. It is organized as follows: In Section B, we provide a theoretical explanation of why using shared randomness in communication with stochastic rounding can improve performance (theoretical explanation for technique 1 in Experiment *More aggressive quantization*). Then we demonstrate more experimental results in Section C. In Section D, we illustrate why naively quantizing communication in D-PSGD fails to converge asymptotically, as a proof to Theorem 1. In Section E, we introduce some useful tools of modeling communication as a Markov Chain for the rest of the proof (part of the intuition is illustrated in the paper). We recommend to go through this before getting into Section F to H. Finally we will provide proof to Theorem 2-4 in Section F to H, with corollaries contained in the corresponding sections.

## B Why sharing randomness improves performance (Experiment 6.4)

In this section, we provide a theoretical explanation why using shared randomness in the stochastic rounding is able to improve the performance. With out the loss of generality, in the following analysis, we let the quantization step associated with stochastic rounding quantizer  $\mathcal{Q}$  be  $\delta = 1$ . For any  $z$  quantized using  $\mathcal{Q}$ , let  $z_f = z - \lfloor z \rfloor$ , the variance of quantization error can be expressed as

$$\mathbb{E} \|\mathcal{Q}(z) - z\|^2 = (1 - z_f)(-z_f)^2 + z_f(1 - z_f)^2 = z_f(1 - z_f) \quad (1)$$

Note that in Moniqua, the term associate with quantization error is

$$\begin{aligned} \mathbb{E} \|\Omega_k e_i\|^2 &= \mathbb{E} \left\| \sum_{j=1}^n ((q_{k,j} - x_{k,j}) - (q_{k,i} - x_{k,i})) W_{ji} \right\|^2 \\ &\stackrel{\text{Jensen's Inequality}}{\leq} \sum_{j=1}^n W_{ji} \mathbb{E} \|(q_{k,j} - x_{k,j}) - (q_{k,i} - x_{k,i})\|^2 \end{aligned}$$

and it shows that the key point is to reduce the error bound of

$$\mathbb{E} \|(q_{k,j} - x_{k,j}) - (q_{k,i} - x_{k,i})\|^2$$

We first show for  $\forall x, y \in \mathbb{R}^d$

$$\mathbb{E} \|(\mathcal{Q}(x) - x) - (\mathcal{Q}(y) - y)\|^2 = \mathbb{E} \|\mathcal{Q}(y - x) - (y - x)\|^2$$

With out the loss of generality, let  $x - \lfloor x \rfloor \leq y - \lfloor y \rfloor$ . Let  $x_f = x - \lfloor x \rfloor$  and  $y_f = y - \lfloor y \rfloor$ , then

$$\begin{aligned} \lfloor x + u \rfloor &= \lfloor x \rfloor \quad \text{and} \quad \lfloor y + u \rfloor = \lfloor y \rfloor, \text{ with probability } \lceil y \rceil - y \\ \lfloor x + u \rfloor &= \lceil x \rceil \quad \text{and} \quad \lfloor y + u \rfloor = \lceil y \rceil, \text{ with probability } x - \lfloor x \rfloor \\ \lfloor x + u \rfloor &= \lfloor x \rfloor \quad \text{and} \quad \lfloor y + u \rfloor = \lceil y \rceil, \text{ with probability } (\lceil x \rceil - x) - (\lceil y \rceil - y) \end{aligned}$$

Then we have

$$\mathbb{E} \|(\mathcal{Q}(x) - x) - (\mathcal{Q}(y) - y)\|^2$$

$$\begin{aligned}
&= \mathbb{E} \left\| \left( \delta \left\lfloor \frac{x}{\delta} + u \right\rfloor - x \right) - \left( \delta \left\lfloor \frac{y}{\delta} + u \right\rfloor - y \right) \right\|^2 \\
&= (\lceil y \rceil - y)((\lfloor x \rfloor - x) - (\lfloor y \rfloor - y))^2 + (x - \lfloor x \rfloor)((\lceil x \rceil - x) - (\lceil y \rceil - y))^2 \\
&\quad + ((\lceil x \rceil - x) - (\lceil y \rceil - y))((\lfloor x \rfloor - x) - (\lfloor y \rfloor - y))^2 \\
&= (1 - y_f)(x_f - y_f)^2 + (x_f)(x_f - y_f) + (y_f - x_f)(y_f - x_f - 1)^2 \\
&= (1 - y_f + x_f)(y_f - x_f)^2 + (y_f - x_f)(y_f - x_f - 1)^2 \\
&= (1 - y_f + x_f)(y_f - x_f) \\
&= \mathbb{E} \|\mathcal{Q}(y - x) - (y - x)\|^2
\end{aligned}$$

The last equality holds due to equation 1. Next, let

$$\begin{aligned}
\Delta &= y - x \\
r &= \mathcal{Q}(\Delta) - \Delta
\end{aligned}$$

And let  $r_h$  denote  $h$ -th entry of  $r$ , let  $\Delta_h$  denote  $h$ -th entry of  $\Delta$ . We obtain

$$\begin{aligned}
r_h &= \mathcal{Q}(\Delta_h) - \Delta_h \\
&= \delta \begin{cases} -\frac{\Delta_h}{\delta} + \left\lfloor \frac{\Delta_h}{\delta} \right\rfloor + 1, & p_t \leq \frac{\Delta_h}{\delta} - \left\lfloor \frac{\Delta_h}{\delta} \right\rfloor \\ -\frac{\Delta_h}{\delta} + \left\lfloor \frac{\Delta_h}{\delta} \right\rfloor, & \text{otherwise} \end{cases} \\
&= \delta \begin{cases} -q + 1, & p_t \leq q \\ -q, & \text{otherwise} \end{cases}
\end{aligned}$$

where

$$q = \frac{\Delta_h}{\delta} - \left\lfloor \frac{\Delta_h}{\delta} \right\rfloor, q \in [0, 1]$$

Based on that, we have

$$\begin{aligned}
\mathbb{E} [r_h^2] &\leq \delta^2 ((-q + 1)^2 q + (-q)^2 (1 - q)) \\
&= \delta^2 q (1 - q) \\
&\leq \delta^2 \min\{q, 1 - q\}
\end{aligned}$$

Since  $\min\{q, 1 - q\} \leq \left\lfloor \frac{x_h}{\delta} \right\rfloor$ , we have

$$\mathbb{E} [r_h^2] \leq \delta^2 \left\lfloor \frac{\Delta_h}{\delta} \right\rfloor \leq \delta |\Delta_h|$$

Summing over the index  $h$  yields,

$$\mathbb{E} \|r\|_2^2 \leq \delta \mathbb{E} \|\Delta\|_1 \leq \sqrt{d} \delta \mathbb{E} \|\Delta\|_2$$

Pushing back  $x$  and  $r$ , we have

$$\mathbb{E} \|\mathcal{Q}(y - x) - (y - x)\|^2 \leq \sqrt{d} \delta \mathbb{E} \|y - x\| = \sqrt{d} \delta \mathbb{E} \|x - y\|$$

Putting it back we have

$$\mathbb{E} \|(\mathcal{Q}(x) - x) - (\mathcal{Q}(y) - y)\|^2 \leq \sqrt{d} \delta \mathbb{E} \|x - y\|$$

Now we can see that the error term is bounded by the distance of two quantized tensor, which, in decentralized training, refers to the distance between two models on adjacent workers. In such a way, the error bound can be reduced since the workers are getting close to each other.

## C More Experimental Results

### C.1 Compute Number of Bits

In Experiment 6.4, we calculate the number of bits in the following way: First, we calculate the total number of bits each worker send out, sum them up and divided by number of epochs, and we get the average bandwidth consumption  $\overline{BW}$  of the whole system in each epoch. Then we compute

the number of bits required for each number in the following way (note that every worker has 2 neighbors):

$$\#bits = \frac{\overline{BW}}{\#neighbors \cdot \#workers \cdot \#params \text{ of model}}$$

In our experiments,  $\#neighbors=2$ ,  $\#workers=8$ . For VGG16,  $\#params \text{ of model}=15,245,130$  while for ResNet110,  $\#params \text{ of model}=1,146,842$ . We formalize the results in Table C.1<sup>1</sup>.

Table 1: Bandwidth consumption under different  $\theta$  and  $\delta$  when applying linear quantizer in Moniqua

| MODEL     | MOD PARAM $\theta$ | QUANT STEP | BYTES/EPOCH | AVG BITS |
|-----------|--------------------|------------|-------------|----------|
| VGG16     | NONE               | NONE       | 45594MB     | 32       |
|           | 1.0                | 0.01       | 5206MB      | 3.65     |
|           | 0.08               | 0.01       | 5192MB      | 3.64     |
| RESNET110 | NONE               | NONE       | 3430MB      | 32       |
|           | 2.0                | 0.01       | 609MB       | 5.67     |
|           | 1.3                | 0.01       | 608MB       | 5.67     |

We also show demonstrate the wall clock time comparison of different algorithms in the experiment of Evaluation of Moniqua under different algorithms (Table C.1). Note that the numbers are the wall clock time consumed per epoch in average.

Table 2: Wall Clock Time consumption (Seconds)/Epoch in average under different network in Experiment of Evaluation of Moniqua.

|             | 100MBPS/0.15MS | 20MBPS/0.15MS | 100MBPS/10MS |
|-------------|----------------|---------------|--------------|
| CENTRALIZED | 38.92          | 206.14        | 343.28       |
| D-PSGD      | 36.25          | 189.48        | 310.98       |
| DCD-PSGD    | 32.99          | 105.40        | 202.42       |
| ECD-PSGD    | 31.96          | 105.26        | 202.04       |
| MONIQUA     | 22.42          | 95.08         | 184.86       |

## C.2 Various Quantizers

In this section, we will verify Moniqua is applicable to other quantizers aside from linear quantizer as shown in the paper. We test it on two more quantizers:

### 1. Nearest Rounding (Biased)

$$\mathcal{Q}(x) = \delta \left\lfloor \frac{x}{\delta} + 0.5 \right\rfloor$$

where  $\delta$  is the quantization step as defined in the linear quantizer. In this experiment, we set  $\delta = 0.01$ , the same value as we used in the paper with stochastic rounding.

### 2. Randomized Gossip (Non-linear)

$$\mathcal{Q}(x) = \begin{cases} x, & \text{with probability } p \\ 0, & \text{with probability } 1 - p \end{cases}$$

In this experiment, we set  $p = 0.7$ .

We train ResNet110 on CIFAR10, and plot the results in Figure 1. We can see that the training curves of using three quantizers are all aligned with D-PSGD with full-precision communication. Note that in the paper we show that previous work cannot preserve the aligned curve even with stochastic rounding (unbiased), thus we are not comparing them here.

<sup>1</sup>Note that we only put results that's 'close to the limit of Moniqua' here

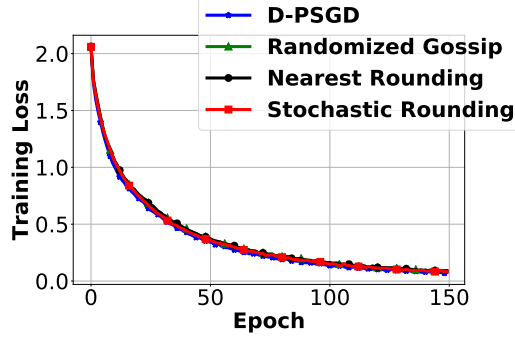

Figure 1: Performance of algorithms under different quantizer

### C.3 More results on different $\theta$

In this experiment, we plot more result of training ResNet110 and VGG16 on CIFAR10 under different  $\delta$  and  $\theta$  in the experiment of aggressive quantization. And we plot the results in Figure 2 and Figure 3.

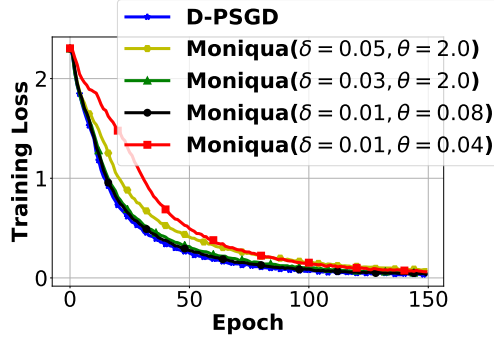

Figure 2: Performance of Moniqua on VGG16 under different  $\theta$  and  $\delta$

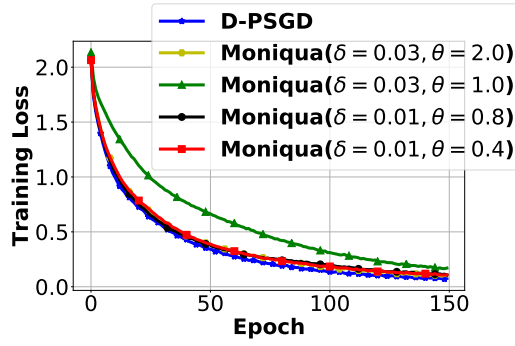

Figure 3: Performance of Moniqua on ResNet110 under different  $\theta$  and  $\delta$

## D Why Naive Quantization Fails in D-PSGD (Proof to Theorem 1)

The update rule of naive quantization on D-PSGD is

$$x_{k+1,i} = x_{k,i}W_{ii} + \sum_{j=1, j \neq i}^n \mathcal{Q}(x_{k,j})W_{ji} - \alpha_k \tilde{g}_{k,i} = x_{k,i} + \sum_{j=1, j \neq i}^n (\mathcal{Q}(x_{k,j}) - x_{k,i})W_{ji} - \alpha_k \tilde{g}_{k,i}$$

where  $\alpha_k$  is allowed to vary with any policy. Let

$$\begin{aligned} X_k &= [x_{k,1}, \dots, x_{k,n}] \in \mathbb{R}^{n \times d} \\ \Omega_k &= \left[ \sum_{j \neq 1} W_{j1} (\mathcal{Q}(x_{k,j}) - x_{k,1}), \dots, \sum_{j \neq n} W_{jn} (\mathcal{Q}(x_{k,j}) - x_{k,n}) \right] \in \mathbb{R}^{n \times d} \\ \tilde{G}_k &= [\tilde{g}_{k,1}, \dots, \tilde{g}_{k,n}] \in \mathbb{R}^{n \times d} \end{aligned}$$

equivalently we have

$$X_{k+1} = X_k + \Omega_k - \alpha_k \tilde{G}_k$$

Let  $Y_k = X_k - x^* \mathbb{1}_n^\top$ , and considering the fact that  $\nabla f(x) = x - \delta/2 = x - x^*$ , we can rewrite the update rule as

$$Y_{k+1} e_i = Y_k e_i + \Omega_k e_i - \alpha_k Y_k e_i + \alpha_k (\tilde{G}_k - G_k) e_i$$

where  $(\tilde{G}_k - G_k)$  denotes variance in the gradient sampling.

Suppose that by using the update rule of naive quantization, worker  $i$  converges to  $x^*$ . Then there must exist a  $K$  such that  $\forall k \geq K$ ,

$$\mathbb{E} \|Y_{k+1} e_i\|^2 \leq \mathbb{E} \|Y_k e_i\|^2 < \frac{\phi^2 \delta^2}{8(1 + \phi^2)} \quad (2)$$

Next we show that this assumption lets us derive a contradiction. Firstly, considering the property of linear quantizer,

$$\frac{\delta^2}{4} \leq \mathbb{E} \|\mathcal{Q}(x_{k,i}) - x^*\|^2 \leq 2\mathbb{E} \|\mathcal{Q}(x_{k,i}) - x_{k,i}\|^2 + 2\mathbb{E} \|x_{k,i} - x^*\|^2$$

As a result

$$\mathbb{E} \|\mathcal{Q}(x_{k,i}) - x_{k,i}\|^2 \geq \frac{\delta^2}{8} - \frac{\phi^2 \delta^2}{8(1 + \phi^2)} = \frac{\delta^2}{8(1 + \phi^2)}$$

Since  $\mathcal{Q}$  is unbiased, that means  $\mathbb{E}[\mathcal{Q}(x) - x] = 0$ , then we have

$$\begin{aligned} & \mathbb{E} \|\Omega_k e_i\|^2 \\ &= \mathbb{E} \left\| \sum_{j \neq i} W_{ji} (\mathcal{Q}(x_{k,j}) - x_{k,i}) \right\|^2 \\ &= \sum_{j \in \mathcal{N}_i} W_{ji}^2 \mathbb{E} \|(\mathcal{Q}(x_{k,j}) - x_{k,i})\|^2 + \sum_{m \neq n \neq i} \mathbb{E} \langle (\mathcal{Q}(x_{k,m}) - x_{k,i}) W_{mi}, (\mathcal{Q}(x_{k,n}) - x_{k,i}) W_{ni} \rangle \\ &\geq \phi^2 \sum_{j \in \mathcal{N}_i} \mathbb{E} \|(\mathcal{Q}(x_{k,j}) - x_{k,i})\|^2 + \sum_{m \neq n \neq i} \mathbb{E} \langle (\mathcal{Q}(x_{k,m}) - x_{k,i}) W_{mi}, (\mathcal{Q}(x_{k,n}) - x_{k,i}) W_{ni} \rangle \\ &\stackrel{\text{unbiased quantizer}}{=} \phi^2 \sum_{j \in \mathcal{N}_i} \mathbb{E} \|\mathcal{Q}(x_{k,j}) - x_{k,i}\|^2 \\ &\geq \frac{\phi^2 \delta^2}{8(1 + \phi^2)} \end{aligned}$$

Putting it back to the update rule, we obtain

$$\begin{aligned} & \mathbb{E} \|Y_{k+1} e_i\|^2 \\ &= \mathbb{E} \left\| (Y_k + \Omega_k - \alpha_k Y_k + \alpha_k (\tilde{G}_k - G_k)) e_i \right\|^2 \\ &\stackrel{(*)}{=} \mathbb{E} \|(1 - \alpha_k) Y_k e_i\|^2 + \mathbb{E} \|\Omega_k e_i\|^2 + \mathbb{E} \left\| \alpha_k (\tilde{G}_k - G_k) e_i \right\|^2 \end{aligned}$$

$$\begin{aligned} &\geq \mathbb{E} \|\Omega_k e_i\|^2 \\ &\geq \frac{\phi^2 \delta^2}{8(1+\phi^2)} \end{aligned}$$

where cross terms in the  $(*)$  step are all 0 due to the unbiased quantizer and unbiased sampling of the gradient. Her we obtain the contradictory that  $\frac{\phi^2 \delta^2}{8(1+\phi^2)} \leq \mathbb{E} \|x_{k+1} - x^*\|^2 < \frac{\phi^2 \delta^2}{8(1+\phi^2)}$ . That being said, for  $\forall k, i$

$$\mathbb{E} \|x_{k,i} - x^*\|^2 \geq \frac{\phi^2 \delta^2}{8(1+\phi^2)}$$

Thus we complete the proof.

## E A Markov Chain Analysis on the Communication

To better understand how the parallel workers reach consensus over a communication matrix, in this section we use theory from the analysis of Markov Chains to obtain some useful lemmas for proof of Moniqua on D-PSGD and AD-PSGD.

Since the communication matrix  $W$  is doubly stochastic (each row and column sum to 1), it has the same structure as the transition matrix of a Markov Chain with  $\frac{\mathbb{1}_n}{n}$  as its the stationary distribution ( $W \frac{\mathbb{1}_n}{n} = \frac{\mathbb{1}_n}{n}$ ). Now let  $t_{\text{mix}}$  and  $d(t)$  denote the mixing time and maximal distance between initial state and stationary distribution as defined in Markov Chain theory.<sup>2</sup>

### E.1 D-PSGD

In D-PSGD, the communication matrix is fixed during the training. That makes it perfectly aligned with the structure of a Markov Chain. As a result, we obtain the following lemma:

**Lemma 1**

$$\left\| W^t \left( I - \frac{\mathbb{1}_n \mathbb{1}_n^\top}{n} \right) \right\|_1 \leq 2 \cdot 2^{-\lfloor \frac{t}{t_{\text{mix}}} \rfloor}$$

**Proof** For  $\forall x \in \mathbb{R}^d$ , let  $u \in \mathbb{R}^d$  be such a vector that every entry of  $u$  is the positive entry of  $x$  and 0 otherwise. Let  $v \in \mathbb{R}^d$  be such a vector that every entry of  $v$  is the absolute value of negative entry of  $x$  and 0 otherwise. The setting above means  $x = u - v$ . For example,

$$\begin{aligned} x &= [2, -1]^\top \\ u &= [2, 0]^\top \\ v &= [0, 1]^\top \end{aligned}$$

And we have

$$\begin{aligned} &\left\| W^t \left( I - \frac{\mathbb{1}_n \mathbb{1}_n^\top}{n} \right) x \right\|_1 \\ &= \left\| W^t \left( I - \frac{\mathbb{1}_n \mathbb{1}_n^\top}{n} \right) (u - v) \right\|_1 \\ &\leq \left\| W^t \left( I - \frac{\mathbb{1}_n \mathbb{1}_n^\top}{n} \right) u \right\|_1 + \left\| W^t \left( I - \frac{\mathbb{1}_n \mathbb{1}_n^\top}{n} \right) v \right\|_1 \\ &= \mathbb{1}_n^\top u \left\| W^t \frac{u}{\mathbb{1}_n^\top u} - \frac{\mathbb{1}_n}{n} \right\|_1 + \mathbb{1}_n^\top v \left\| W^t \frac{v}{\mathbb{1}_n^\top v} - \frac{\mathbb{1}_n}{n} \right\|_1 \\ &\leq 2(\mathbb{1}_n^\top u + \mathbb{1}_n^\top v) d(t) \\ &\leq 2d(t) \|x\|_1 \end{aligned}$$

<sup>2</sup>Here we are using notation from Chapter 4.5 of *Markov Chains and Mixing Times* (Levin 2009), available at <https://pages.uoregon.edu/dlevin/MARKOV/markovmixing.pdf>

Considering the definition of L1-norm, we have

$$\left\| W^t \left( I - \frac{\mathbb{1}_n \mathbb{1}_n^\top}{n} \right) \right\|_1 = \max \frac{\left\| W^t \left( I - \frac{\mathbb{1}_n \mathbb{1}_n^\top}{n} \right) x \right\|_1}{\|x\|_1} \leq 2d(t)$$

According to a well-known results on the theory of Markov Chains,<sup>3</sup>  $d(lt_{\text{mix}}) \leq 2^{-l}$  holds for any non-negative integer  $l$ , so we have

$$\left\| W^t \left( I - \frac{\mathbb{1}_n \mathbb{1}_n^\top}{n} \right) \right\|_1 \leq 2d(t) \leq 2d \left( \frac{t}{t_{\text{mix}}} \cdot t_{\text{mix}} \right) \leq 2d \left( \left\lfloor \frac{t}{t_{\text{mix}}} \right\rfloor t_{\text{mix}} \right) \leq 2 \cdot 2^{-\lfloor \frac{t}{t_{\text{mix}}} \rfloor}$$

That completes the proof.

Additionally, based on standard results in the theory of reversible Markov Chains, we also have<sup>4</sup>

$$t_{\text{mix}} \leq \log \left( \frac{1}{\frac{1}{4} \cdot \frac{1}{n}} \right) \frac{1}{1 - \rho} \leq \frac{\log(4n)}{1 - \rho}.$$

## E.2 AD-PSGD

Note that unlike D-PSGD, here  $W_k$  can be different at each update step and usually each individually have spectral radius  $\rho = 1$ , so we can't expect to get a bound in terms of a bound on the spectral gap as we did in Theorems 1 and 2. Instead, we require the following condition, which is inspired by the literature on Markov chain Monte Carlo methods: for some constant  $t_{\text{mix}}$  (here  $t_{\text{mix}}$  is the same as  $t_{\text{mix}}$  in the paper) and for any  $k$  and any non-negative vector  $\mu \in \mathbb{R}^d$  such that  $\mathbb{1}_n^\top \mu = 1$ , it must hold that

$$\left\| \left( \prod_{i=1}^{t_{\text{mix}}} W_{k+i} \right) \mu - \frac{\mathbb{1}_n}{n} \right\|_1 \leq \frac{1}{2}.$$

We call this constant  $t_{\text{mix}}$  because it is effectively the *mixing time* of the time-inhomogeneous Markov chain with transition probability matrix  $W_k$  at time  $k$ . Note that this condition is more general than those used in previous work on AD-PSGD because it does not require that the  $W_k$  are sampled independently or in an unbiased manner. Based on the above analysis, we can prove the following lemma, which is analogous to the lemma used in the synchronous case.

**Lemma 2** *For any  $k \geq 0$  and for any  $b \geq a \geq 0$ , there exists  $t_{\text{mix}}$  such that*

$$\left\| \prod_{q=a}^b W_q \left( I - \frac{\mathbb{1}_n \mathbb{1}_n^\top}{n} \right) \right\|_1 \leq 2 \cdot 2^{-\lfloor \frac{b-a+1}{t_{\text{mix}}} \rfloor}$$

**Proof** Note that for any  $x \in \mathbb{R}^d$ , and let  $u$  and  $v$  be two vectors having same definition as in Lemma 1 with respect to  $x$ , then we have for any  $k$

$$\begin{aligned} & \left\| \prod_{q=1}^{t_{\text{mix}}} W_{q+k} \left( I - \frac{\mathbb{1}_n \mathbb{1}_n^\top}{n} \right) x \right\|_1 \\ &= \left\| \prod_{q=1}^{t_{\text{mix}}} W_{q+k} \left( I - \frac{\mathbb{1}_n \mathbb{1}_n^\top}{n} \right) (u - v) \right\|_1 \\ &\leq \left\| \prod_{q=1}^{t_{\text{mix}}} W_{q+k} \left( I - \frac{\mathbb{1}_n \mathbb{1}_n^\top}{n} \right) u \right\|_1 + \left\| \prod_{q=1}^{t_{\text{mix}}} W_{q+k} \left( I - \frac{\mathbb{1}_n \mathbb{1}_n^\top}{n} \right) v \right\|_1 \\ &= \mathbb{1}_n^\top u \left\| \prod_{q=1}^{t_{\text{mix}}} W_{q+k} \frac{u}{\mathbb{1}_n^\top u} - \frac{\mathbb{1}_n}{n} \right\|_1 + \mathbb{1}_n^\top v \left\| \prod_{q=1}^{t_{\text{mix}}} W_{q+k} \frac{v}{\mathbb{1}_n^\top v} - \frac{\mathbb{1}_n}{n} \right\|_1 \\ &\leq \frac{1}{2} (\mathbb{1}_n^\top u + \mathbb{1}_n^\top v) \end{aligned}$$

<sup>3</sup>Again, see *Markov Chains and Mixing Times* for more details.

<sup>4</sup>Detailed analysis and proofs of this result can be found in chapter 12.2 of *Markov Chains and Mixing Times*.

$$\leq \frac{1}{2} \|x\|_1$$

Considering the definition of the induced  $\ell_1$  operator norm, we have

$$\left\| \prod_{q=1}^{t_{\text{mix}}} W_{q+k} \left( I - \frac{\mathbb{1}_n \mathbb{1}_n^\top}{n} \right) \right\|_1 = \max_x \frac{\left\| \prod_{q=1}^{t_{\text{mix}}} W_{q+k} \left( I - \frac{\mathbb{1}_n \mathbb{1}_n^\top}{n} \right) x \right\|_1}{\|x\|_1} \leq \frac{1}{2}$$

As a result, from the submultiplicativity of the matrix induced norm, we obtain

$$\begin{aligned} & \left\| \prod_{q=a}^b W_q \left( I - \frac{\mathbb{1}_n \mathbb{1}_n^\top}{n} \right) \right\|_1 \\ & \leq \left\| \prod_{q=1}^{t_{\text{mix}}} W_{a-1+q} \left( I - \frac{\mathbb{1}_n \mathbb{1}_n^\top}{n} \right) \right\|_1 \cdots \left\| \prod_{q=1}^{t_{\text{mix}}} W_{\dots+q} \left( I - \frac{\mathbb{1}_n \mathbb{1}_n^\top}{n} \right) \right\|_1 \cdot \left\| \prod_{q=1}^{t_r} W_{\dots+q} \left( I - \frac{\mathbb{1}_n \mathbb{1}_n^\top}{n} \right) \right\|_1 \\ & \leq 2^{-\lfloor \frac{b-a+1}{t_{\text{mix}}} \rfloor} \left\| \prod_{q=1}^{t_r} W_{\dots+q} \left( I - \frac{\mathbb{1}_n \mathbb{1}_n^\top}{n} \right) \right\|_1 \end{aligned}$$

where  $t_r = (b - a + 1) \bmod t_{\text{mix}}$ . Note that

$$\left\| \prod_{q=1}^{t_r} W_q \left( I - \frac{\mathbb{1}_n \mathbb{1}_n^\top}{n} \right) \right\|_1 \leq 1 - \frac{1}{n} + (n-1) \frac{1}{n} = 2 - \frac{2}{n} \leq 2$$

Putting it back we obtain

$$\left\| \prod_{q=a}^b W_{\dots+q} \left( I - \frac{\mathbb{1}_n \mathbb{1}_n^\top}{n} \right) \right\|_1 \leq 2 \cdot 2^{-\lfloor \frac{b-a+1}{t_{\text{mix}}} \rfloor}$$

That completes the proof.

Note that in the analysis of Moniqua on AD-PSGD (Section H), we will use this lemma as an assumption.

## F Moniqua on D-PSGD (Proof to Theorem 2)

### F.1 Algorithm and Assumptions

---

**Algorithm 1** General pseudo-code of Decentralized SGD on worker  $i$

---

**Input:** initial point  $x_{0,i} = x_0$ , step size  $\alpha$ , communication matrix  $W$ , number of iterations  $K$ , quantization function  $\mathcal{Q}$ , neighbor list  $\mathcal{N}_i$

- 1: **for**  $k = 0, 1, 2, \dots, K-1$  **do**
- 2:     Make some exchanged information  $q_{k,i}$  available to all the neighbors
- 3:     Compute a local stochastic gradient based on data sample  $\xi_{k,i}$  and current weight  $x_{k,i}$ :  $\tilde{g}_{k,i}$
- 4:     **for**  $j \in \mathcal{N}_i$  **do**
- 5:         Fetch  $q_{k,j}$  from neighbor  $j$  and subtract a bias term  $b_{k,i}$  proportionally:

$$x_{k+\frac{1}{2},i} \leftarrow x_{k,i} + q_{k,j} W_{ji} - b_{k,i} W_{ji}$$

- 6:     **end for**
- 7:     Update the local weight with local gradient:  $x_{k+1,i} \leftarrow x_{k+\frac{1}{2},i} - \alpha \tilde{g}_{k,i}$
- 8: **end for**

**Output:** Averaged model  $\bar{X}_K = \frac{1}{n} \sum_{i=1}^n x_{K,i}$

---

Assumptions:

1. **Lipschitzian Gradient:** All the function  $f_i$  have  $L$ -Lipschitzian gradients.
2. **Spectral Gap:** Communication matrix  $W$  is a symmetric doubly stochastic matrix and for  $\rho \triangleq \max\{|\lambda_2(W)|, |\lambda_n(W)|\}$ ,  $\rho < 1$ , where  $\lambda_i(W)$  denotes  $i$ -th eigenvalue of  $W$ .
3. **Bounded Variance:** There exists  $\sigma$  and  $\varsigma$  such that

$$\mathbb{E}_{\xi_i \sim \mathcal{D}_i} \left\| \nabla \tilde{f}_i(x; \xi_i) - \nabla f_i(x) \right\|^2 \leq \sigma^2, \quad \mathbb{E}_{i \sim \mathcal{U}([n])} \left\| \nabla f_i(x) - \nabla f(x) \right\|^2 \leq \varsigma^2, \forall i$$

where  $\nabla \tilde{f}_i(x; \xi_i)$  denotes gradient sample on worker  $i$  computed via data sample  $\xi_i$ .

4. **Initialization:** All the models are initialized by the same parameters:  $x_{0,i} = x_0, \forall i$  and with out the loss of generality  $x_0 = 0$ .
5. **Gradient magnitude:** The norm of a sampled gradient is bounded by  $\|\tilde{g}_{k,i}\| \leq B$  for some constant  $B$ .

## F.2 Theorems

We highlight all the theorems there:

**Theorem 1** *If we apply a quantizer  $\mathcal{Q}_\omega$  to the communication, making the exchanged information  $q_{k,i} = b_{k,i} = \theta \cdot \mathcal{Q}_\omega\left(\frac{x_{k,i}}{\theta} \bmod 1\right)$ , and we set the hyperparameters to*

$$\theta = \frac{16 \log(4n) \alpha B}{1 - \rho}, \quad \omega = \frac{1 - \rho}{32 \log(4n)}, \quad \text{and} \quad \alpha = \frac{1}{\varsigma^{\frac{2}{3}} K^{\frac{1}{3}} + \sigma \sqrt{\frac{K}{n}} + 2L},$$

*then the output of Algorithm 1 converges at the asymptotic rate*

$$\frac{1}{K} \sum_{k=0}^{K-1} \mathbb{E} \left\| \nabla f(\bar{X}_k) \right\|^2 \lesssim \frac{1}{K} + \frac{\sigma}{\sqrt{nK}} + \frac{\varsigma^{\frac{2}{3}}}{K^{\frac{2}{3}}} + \frac{\sigma^2 n}{\sigma^2 K + n} + \frac{B^2 n}{\sigma^2 K + n}.$$

**Corollary 1** *If we use a linear quantizer with quantization step  $\delta$  as  $\mathcal{Q}_\omega$  in Theorem 1, the number of bits  $\mathcal{B}$  required per dimension per iteration is upper bounded by  $\mathcal{B} \leq \log \left( \frac{32 \log(4n) \sqrt{d}}{1 - \rho} \right)$ .*

**Corollary 2** *Let Algorithm 1 communicate at constant frequency  $\eta$ , that is, run lines 5-7 only when  $k \bmod \eta^{-1} = 0$ . If we use the same quantizer as Corollary 1, the number of bits required per dimension per iteration is upper bounded by  $\mathcal{B} \leq \eta \log \left( \frac{32 \log(4n) \sqrt{d}}{\eta(1 - \rho)} \right)$  and the algorithm converges at the same  $O(1/\sqrt{nK})$  asymptotic rate.*

**Why not using Mod directly?** Here we briefly explain why using  $\theta \cdot \mathcal{Q}_\omega\left(\frac{x}{\theta} \bmod 1\right)$  instead of  $\mathcal{Q}_\omega(x \bmod \theta)$  for theoretical analysis. Note that the quantizers we analyze in the paper holds either one of the property mentioned in Section 3 in the paper.

Note that for Property 1, with a given  $x \leq \theta$ :

$$\left\| \theta \cdot \mathcal{Q}_\omega\left(\frac{x}{\theta} \bmod 1\right) - x \right\| = \theta \left\| \mathcal{Q}_\omega\left(\frac{x}{\theta} \bmod 1\right) - \left(\frac{x}{\theta} \bmod 1\right) \right\| \leq \theta \delta \sqrt{d} = \theta \omega$$

And for Property 2, with a given  $x \leq \theta$ :

$$\left\| \theta \cdot \mathcal{Q}_\omega\left(\frac{x}{\theta} \bmod 1\right) - x \right\| = \theta \left\| \mathcal{Q}_\omega\left(\frac{x}{\theta} \bmod 1\right) - \left(\frac{x}{\theta} \bmod 1\right) \right\| \leq \theta \omega \cdot 1 = \theta \omega$$

As a result, we can use the same bound  $\theta \omega$  for quantizers with either one of the properties, which we will show in the rest of the proof.

## F.3 Proof to Theorem 1

**Proof** *From a local view, applying Moniqua on Algorithm 1 on worker  $i$  at iteration  $k$  can be written as*

$$x_{k+1,i} \leftarrow x_{k,i} + \sum_{j \in \mathcal{N}_i} (q_{k,j} - q_{k,i}) W_{ji} - \alpha \tilde{g}_{k,i}$$

which is equivalent to

$$x_{k+1,i} = x_{k,i} + \sum_{j=1}^n (x_{k,j} - x_{k,i}) W_{ji} - \alpha \tilde{g}_{k,i} + \sum_{j=1}^n ((q_{k,j} - x_{k,j}) - (q_{k,i} - x_{k,i})) W_{ji} \quad (3)$$

From a global view, the update rule can be written as

$$X_{k+1} = X_k + Q_k(W - I) - \alpha \tilde{G}_k = X_k W - \alpha \tilde{G}_k + (Q_k - X_k)(W - I) \quad (4)$$

where

$$\begin{aligned} X_k &= [x_{k,1}, \dots, x_{k,n}] \\ Q_k &= [q_{k,1}, \dots, q_{k,n}] \\ \tilde{G}_k &= [\tilde{g}_{k,1}, \dots, \tilde{g}_{k,n}] \end{aligned}$$

Besides, for convenience, we also have the following notation

$$\begin{aligned} G_k &= [g_{k,1}, \dots, g_{k,n}] \\ \bar{X} &= X \frac{\mathbb{1}_n}{n}, \forall X \in \mathbb{R}^{d \times n} \\ \Omega_k &= (Q_k - X_k)(W - I) \end{aligned}$$

where  $g_{k,i}$  denotes gradient computed via the whole dataset  $\mathcal{D}_i$  and  $x_{k,i}$

We first<sup>5</sup> use mathematical induction to prove  $\|X_k(e_i - e_j)\|_2 \leq \theta = \frac{16 \log(4n)\alpha B}{1-\rho}, \forall i, j \in [n], k \geq 0$ .

I. Firstly, when  $k = 0$ ,  $\|X_0(e_i - e_j)\|_2 = 0 \leq \theta, \forall i, j$

II. Now, suppose for  $\|X_k(e_i - e_j)\|_2 \leq \theta, k \geq 0, \forall i, j$ . We now derive  $\|X_{k+1}(e_i - e_j)\|_2 \leq \theta$ . Note that for  $\forall i, j$ , we have

$$\begin{aligned} & \|X_{k+1}(e_i - e_j)\|_2 \\ & \leq \left\| X_{k+1} \left( \frac{\mathbb{1}_n}{n} - e_i \right) \right\|_2 + \left\| X_{k+1} \left( \frac{\mathbb{1}_n}{n} - e_j \right) \right\|_2 \\ & \leq \left\| X_{k+1} \left( I - \frac{\mathbb{1}_n \mathbb{1}_n^\top}{n} \right) \right\|_{2 \leftarrow 1} \|e_i\|_1 + \left\| X_{k+1} \left( I - \frac{\mathbb{1}_n \mathbb{1}_n^\top}{n} \right) \right\|_{2 \leftarrow 1} \|e_j\|_1 \\ & = 2 \left\| X_{k+1} \left( I - \frac{\mathbb{1}_n \mathbb{1}_n^\top}{n} \right) \right\|_{2 \leftarrow 1} \\ & = 2 \left\| \left( X_k W - \alpha \tilde{G}_k + \Omega_k \right) \left( I - \frac{\mathbb{1}_n \mathbb{1}_n^\top}{n} \right) \right\|_{2 \leftarrow 1} \\ & \stackrel{X_0=0}{=} 2 \left\| \sum_{t=0}^k \left( -\alpha \tilde{G}_t + \Omega_t \right) W^{k-t} \left( I - \frac{\mathbb{1}_n \mathbb{1}_n^\top}{n} \right) \right\|_{2 \leftarrow 1} \\ & \leq 2 \sum_{t=0}^k \left\| \left( -\alpha \tilde{G}_t + \Omega_t \right) W^{k-t} \left( I - \frac{\mathbb{1}_n \mathbb{1}_n^\top}{n} \right) \right\|_{2 \leftarrow 1} \\ & \leq 2 \sum_{t=0}^k \left\| -\alpha \tilde{G}_t + \Omega_t \right\|_{2 \leftarrow 1} \left\| W^{k-t} - \frac{\mathbb{1}_n \mathbb{1}_n^\top}{n} \right\|_1 \\ & \leq 2\alpha \sum_{t=0}^k \left\| \tilde{G}_t \right\|_{2 \leftarrow 1} \left\| W^{k-t} - \frac{\mathbb{1}_n \mathbb{1}_n^\top}{n} \right\|_1 + 2 \sum_{t=0}^k \left\| \Omega_t \right\|_{2 \leftarrow 1} \left\| W^{k-t} - \frac{\mathbb{1}_n \mathbb{1}_n^\top}{n} \right\|_1 \end{aligned}$$

---

<sup>5</sup>Since  $\|X_k(e_i - e_j)\|_\infty \leq \|X_k(e_i - e_j)\|_2$  and  $\|X_k(e_i - e_j)\|_2$  is easier to analyze, so we prove  $\|X_k(e_i - e_j)\|_2 \leq \theta$  that will automatically hold for  $\|X_k(e_i - e_j)\|_\infty \leq \theta$ .

where  $(2 \leftarrow 1)$ -norm denotes a matrix's L2-norm induced by L1-norm, specifically matrix  $A$ 's  $(2 \leftarrow 1)$ -norm can be computed by  $\|A\|_{2 \leftarrow 1} = \max \frac{\|A\|_2}{\|x\|_1}$ . Now since we have the assumption on  $\|X_k(e_i - e_j)\|_2 \leq \theta, k \geq 0, \forall i, j$ , it means  $\forall t \leq k$  and  $\forall i$

$$\begin{aligned}
& \|\Omega_t e_i\| \\
& \leq \left\| \sum_{j=1}^n ((q_{t,j} - x_{t,j}) - (q_{t,i} - x_{t,i})) W_{ji} \right\| \\
& \leq \sum_{j=1}^n W_{ji} \|(q_{t,j} - x_{t,j}) - (q_{t,i} - x_{t,i})\| \\
& \leq \sum_{j=1}^n W_{ji} \left\| \theta \mathcal{Q} \left( \frac{x_{t,j}}{\theta} \mod 1 \right) - \theta \mathcal{Q} \left( \frac{x_{t,i}}{\theta} \mod 1 \right) - (x_{t,j} - x_{t,i}) \right\| \\
& \leq \sum_{j=1}^n W_{ji} \left\| \theta \mathcal{Q} \left( \frac{x_{t,j}}{\theta} \mod 1 \right) - \theta \mathcal{Q} \left( \frac{x_{t,j}}{\theta} \mod 1 \right) - \theta \left( \frac{x_{t,j} - x_{t,i}}{\theta} \mod 1 \right) \right\| \\
& \leq \sum_{j=1}^n W_{ji} \left\| \theta \mathcal{Q} \left( \frac{x_{t,j}}{\theta} \mod 1 \right) - \theta \left( \frac{x_{t,j}}{\theta} \mod 1 \right) - \left( \theta \mathcal{Q} \left( \frac{x_{t,i}}{\theta} \mod 1 \right) - \theta \left( \frac{x_{t,i}}{\theta} \mod 1 \right) \right) \right\| \\
& \leq \sum_{j=1}^n W_{ji} \left\| \theta \mathcal{Q} \left( \frac{x_{t,j}}{\theta} \mod 1 \right) - \theta \left( \frac{x_{t,j}}{\theta} \mod 1 \right) \right\| \\
& + \sum_{j=1}^n W_{ji} \left\| \theta \mathcal{Q} \left( \frac{x_{t,i}}{\theta} \mod 1 \right) - \theta \left( \frac{x_{t,i}}{\theta} \mod 1 \right) \right\| \\
& \leq 2\omega\theta
\end{aligned}$$

Now putting this result and the fact that  $\|\tilde{g}_{k,i}\| \leq B, \forall k, i$

$$\begin{aligned}
& \|X_{k+1}(e_i - e_j)\|_2 \\
& \leq 2\alpha \sum_{t=0}^k \|\tilde{G}_t\|_{2 \leftarrow 1} \left\| W^{k-t} - \frac{\mathbb{1}_n \mathbb{1}_n^\top}{n} \right\|_1 + 2 \sum_{t=0}^k \|\Omega_t\|_{2 \leftarrow 1} \left\| W^{k-t} - \frac{\mathbb{1}_n \mathbb{1}_n^\top}{n} \right\|_1 \\
& \leq 4(\alpha B + 2\omega\theta) \sum_{t=0}^k 2^{-\lfloor (k-t)/t_{\text{mix}} \rfloor} \\
& \leq 4(\alpha B + 2\omega\theta) \sum_{t=0}^{t_{\text{mix}}-1} \sum_{r=0}^{\infty} 2^{-r} \\
& \leq 8(\alpha B + 2\omega\theta) t_{\text{mix}} \\
& \leq 8(\alpha B + 2\omega\theta) \frac{\log(4n)}{1-\rho}
\end{aligned}$$

Derivation of the last four steps and definition of  $t_{\text{mix}}$  are further illustrated in Section E.

Since  $\omega = \frac{1-\rho}{32 \log(4n)}$ , we have

$$\|X_{k+1}(e_i - e_j)\|_2 \leq 8(\alpha B + 2\omega\theta) \frac{\log(4n)}{1-\rho} \leq \frac{16 \log(4n)}{1-\rho} \alpha B = \theta$$

and the completes the proof of  $\|X_k(e_i - e_j)\|_2 \leq \theta, \forall i, j, k$

Next we analyze the quantization error term  $\Omega_k$ .

$$\sum_{k=0}^{K-1} \mathbb{E} \|\Omega_k\|_F^2$$

$$\begin{aligned}
&= \sum_{k=0}^{K-1} \sum_{i=1}^n \mathbb{E} \|\Omega_k e_i\|^2 \\
&\leq \sum_{k=0}^{K-1} \sum_{i=1}^n \mathbb{E} \left\| \sum_{j=1}^n ((q_{k,j} - x_{k,j}) - (q_{k,i} - x_{k,i})) W_{ji} \right\|^2 \\
&\stackrel{Jensen}{\leq} \sum_{k=0}^{K-1} \sum_{i=1}^n \sum_{j=1}^n W_{ji} \mathbb{E} \|((q_{k,j} - x_{k,j}) - (q_{k,i} - x_{k,i}))\|^2 \\
&= \sum_{k=0}^{K-1} \sum_{i=1}^n \sum_{j=1}^n W_{ji} \left( \mathbb{E} \left\| \theta \mathcal{Q} \left( \frac{x_{k,j}}{\theta} \mod 1 \right) - \theta \mathcal{Q} \left( \frac{x_{k,i}}{\theta} \mod 1 \right) - (x_{k,j} - x_{k,i}) \right\|^2 \right) \\
&\leq \sum_{k=0}^{K-1} \sum_{i=1}^n \sum_{j=1}^n W_{ji} \\
&\quad \left( \mathbb{E} \left\| \theta \mathcal{Q} \left( \frac{x_{k,j}}{\theta} \mod 1 \right) - \theta \mathcal{Q} \left( \frac{x_{k,i}}{\theta} \mod 1 \right) - \theta \left( \frac{x_{k,j} - x_{k,i}}{\theta} \mod 1 \right) \right\|^2 \right) \\
&\leq \sum_{k=0}^{K-1} \sum_{i=1}^n \sum_{j=1}^n W_{ji} \\
&\quad \left( \mathbb{E} \left\| \theta \mathcal{Q} \left( \frac{x_{k,j}}{\theta} \mod 1 \right) - \theta \left( \frac{x_{k,j}}{\theta} \mod 1 \right) - \left( \theta \mathcal{Q} \left( \frac{x_{k,i}}{\theta} \mod 1 \right) - \theta \left( \frac{x_{k,i}}{\theta} \mod 1 \right) \right) \right\|^2 \right) \\
&\leq 2 \sum_{k=0}^{K-1} \sum_{i=1}^n \sum_{j=1}^n W_{ji} \mathbb{E} \left\| \theta \mathcal{Q} \left( \frac{x_{k,j}}{\theta} \mod 1 \right) - \theta \left( \frac{x_{k,j}}{\theta} \mod 1 \right) \right\|^2 \\
&\quad + 2 \sum_{k=0}^{K-1} \sum_{i=1}^n \sum_{j=1}^n W_{ji} \mathbb{E} \left\| \theta \mathcal{Q} \left( \frac{x_{k,i}}{\theta} \mod 1 \right) - \theta \left( \frac{x_{k,i}}{\theta} \mod 1 \right) \right\|^2 \\
&\leq 4 \sum_{k=0}^{K-1} \sum_{i=1}^n \mathbb{E} \left\| \theta \mathcal{Q} \left( \frac{x_{k,i}}{\theta} \mod 1 \right) - \theta \left( \frac{x_{k,i}}{\theta} \mod 1 \right) \right\|^2 \\
&\leq 4 \sum_{k=0}^{K-1} \sum_{i=1}^n \omega^2 \theta^2 \\
&\leq \alpha^2 B^2 n K
\end{aligned}$$

The last step holds because  $\omega\theta = \frac{1}{2}\alpha B$ . Until now we have proved

$$\begin{aligned}
&\|X_k(e_i - e_j)\|^2 \leq \theta, \forall i, j, k \\
&\sum_{k=0}^{K-1} \mathbb{E} \|\Omega_k\|_F^2 \leq \alpha^2 B^2 n K
\end{aligned}$$

Next we start to prove the convergence of Moniqua:

From Lemma 3 (Definition of constant  $M_1$  and  $M_2$  can be found in Lemma 3) we have

$$\begin{aligned}
&\frac{1 - \alpha L}{K} \sum_{k=0}^{K-1} \mathbb{E} \|\bar{G}_k\|^2 + \frac{M_2}{K} \sum_{k=0}^{K-1} \mathbb{E} \|\nabla f(\bar{X}_k)\|^2 \\
&\leq \frac{2(f(0) - f^*)}{\alpha K} + \frac{\alpha L}{n} \sigma^2 + \frac{2\alpha^2 L^2 (\sigma^2 + 3\varsigma^2)}{M_1(1 - \rho)^2} + \frac{2L^2}{M_1 n K (1 - \rho)^2} \sum_{k=1}^{K-1} \mathbb{E} \|\Omega_k\|_F^2
\end{aligned}$$

Pushing it to the  $\Omega_k$ , and let  $M_1, M_2 \geq \frac{1}{2}$  we have

$$\frac{1}{K} \sum_{k=0}^{K-1} \mathbb{E} \|\nabla f(\bar{X}_k)\|^2 \leq \frac{4(f(0) - f^*)}{\alpha K} + \frac{2\alpha L}{n} \sigma^2 + \frac{8\alpha^2 L^2 (\sigma^2 + 3\varsigma^2)}{(1 - \rho)^2} + \frac{8\alpha^2 B^2 L^2}{(1 - \rho)^2}$$

By setting  $\alpha = \frac{1}{\varsigma^{\frac{2}{3}} K^{\frac{1}{3}} + \sigma \sqrt{\frac{K}{n}} + 2L}$ , we have

$$\begin{aligned} \frac{1}{K} \sum_{k=0}^{K-1} \mathbb{E} \|\nabla f(\bar{X}_k)\|^2 &\leq \frac{8(f(0) - f^*)L}{K} + \frac{4\sigma(f(0) - f^* + L/2)}{\sqrt{nK}} + \frac{4\varsigma^{\frac{2}{3}}(f(0) - f^*)}{K^{\frac{2}{3}}} \\ &\quad + \frac{8L^2\sigma^2n}{(1-\rho)^2(\sigma^2K + 4nL^2)} + \frac{24L^2\varsigma^{\frac{2}{3}}}{(1-\rho)^2K^{\frac{2}{3}}} + \frac{8L^2B^2n}{(1-\rho)^2(\sigma^2K + 4nL^2)} \\ &\lesssim \frac{1}{K} + \frac{\sigma}{\sqrt{nK}} + \frac{\varsigma^{\frac{2}{3}}}{K^{\frac{2}{3}}} + \frac{\sigma^2n}{\sigma^2K + n} + \frac{B^2n}{\sigma^2K + n} \end{aligned}$$

That completes the proof of Theorem 1.

#### F.4 Proof to Corollary

##### Proof to Corollary 1

**Proof** The number of bits used in the communication per iteration per dimension can be written as  $\log(\frac{1}{\delta})$ , note that for linear quantizer,  $\omega = \delta\sqrt{d}$ , so we have number of bits is upper bounded by  $\log(\frac{1}{\delta}) = \log\left(\frac{\sqrt{d}}{\omega}\right) = \log\left(\frac{32\log(4n)\sqrt{d}}{1-\rho}\right)$

**Proof to Corollary 2** Note that for low frequency communication, we can rewrite the communication matrix  $\widetilde{W}$  as

$$\widetilde{W} = \begin{cases} W, & k \bmod \frac{1}{\eta} = 0 \\ I, & \text{otherwise} \end{cases}$$

Now we derive the  $\theta$

$$\begin{aligned} &\|X_k(e_i - e_j)\|_2 \\ &\leq \left\|X_k\left(\frac{\mathbb{1}_n}{n} - e_i\right)\right\|_2 + \left\|X_k\left(\frac{\mathbb{1}_n}{n} - e_j\right)\right\|_2 \\ &\leq \left\|X_k\left(I - \frac{\mathbb{1}_n\mathbb{1}_n^\top}{n}\right)\right\|_{2\leftarrow 1} \|e_i\|_1 + \left\|X_k\left(I - \frac{\mathbb{1}_n\mathbb{1}_n^\top}{n}\right)\right\|_{2\leftarrow 1} \|e_j\|_1 \\ &= 2 \left\|X_k\left(I - \frac{\mathbb{1}_n\mathbb{1}_n^\top}{n}\right)\right\|_{2\leftarrow 1} \\ &\leq 2 \left\|\left(X_{k-1}\widetilde{W} - \alpha\widetilde{G}_{k-1} + \Omega_{k-1}\right)\left(I - \frac{\mathbb{1}_n\mathbb{1}_n^\top}{n}\right)\right\|_{2\leftarrow 1} \\ &= 2 \left\|\sum_{t=0}^{k-1} \left(-\alpha\widetilde{G}_t + \Omega_t\right)\widetilde{W}^{k-t-1}\left(I - \frac{\mathbb{1}_n\mathbb{1}_n^\top}{n}\right)\right\|_{2\leftarrow 1} \\ &\leq 2 \sum_{t=0}^{k-1} \left\|\left(-\alpha\widetilde{G}_t + \Omega_t\right)\widetilde{W}^{k-t-1}\left(I - \frac{\mathbb{1}_n\mathbb{1}_n^\top}{n}\right)\right\|_{2\leftarrow 1} \\ &\leq 2 \sum_{t=0}^{k-1} \left\|-\alpha\widetilde{G}_t + \Omega_t\right\|_{2\leftarrow 1} \left\|W^{\lfloor\eta(k-t-1)\rfloor} - \frac{\mathbb{1}_n\mathbb{1}_n^\top}{n}\right\|_1 \\ &\leq 4(\alpha B + 2\omega\theta) \sum_{t=0}^{k-1} 2^{-\lfloor\lfloor\eta(k-t-1)\rfloor/t_{\text{mix}}\rfloor} \\ &\leq 4(\alpha B + 2\omega\theta) \sum_{s=0}^{t_{\text{mix}}-1} \sum_{t=0}^{\frac{1}{\eta}-1} \sum_{r=0}^{\infty} 2^{-r} \\ &\leq 8(\alpha B + 2\omega\theta) \frac{t_{\text{mix}}}{\eta} \end{aligned}$$

$$\leq 8(\alpha B + 2\omega\theta) \frac{\log(4n)}{\eta(1-\rho)}$$

Let the last term be  $\theta$ , we get

$$\theta = \frac{8 \log(4n)}{\eta(1-\rho) - 16\omega \log(4n)} \alpha B$$

Set  $\omega = \frac{\eta(1-\rho)}{32 \log(4n)}$ , we have

$$\theta = \frac{16 \log(4n)}{\eta(1-\rho)} \alpha B$$

Similar to Corollary 1, considering the communication happens at the frequency of  $\eta$ , we have number of bits is upper bounded by  $\eta \log\left(\frac{1}{\delta}\right) = \eta \log\left(\frac{\sqrt{d}}{\omega}\right) = \eta \log\left(\frac{32 \log(4n) \sqrt{d}}{\eta(1-\rho)}\right)$ .

Next, we discuss the dependency of asymptotic rate on the frequency  $\eta$ . Now for convenience, we let  $\mathcal{T} = \eta^{-1}$ . From a local view, the update rule of  $\eta$  frequency communication can be written as

$$x_{k+1,i} \leftarrow x_{k,i} + \sum_{j \in \mathcal{N}_i} (q_{k,j} - q_{k,i}) \widetilde{W}_{ji} - \alpha \widetilde{g}_{k,i}$$

which is equivalent to

$$x_{k+1,i} = x_{k,i} + \sum_{j=1}^n (x_{k,j} - x_{k,i}) \widetilde{W}_{ji} - \alpha \widetilde{g}_{k,i} + \sum_{j=1}^n ((q_{k,j} - x_{k,j}) - (q_{k,i} - x_{k,i})) \widetilde{W}_{ji} \quad (5)$$

From a global view, the update rule can be written as

$$X_{k+1} = X_k + Q_k(\widetilde{W} - I) - \alpha \widetilde{G}_k = X_k \widetilde{W} - \alpha \widetilde{G}_k + (Q_k - X_k)(\widetilde{W} - I) \quad (6)$$

Since change of communication frequency will only change to the terms in the proof of Moniqua that relate to the communication, we can reuse the intermediate result from Moniqua as

$$\frac{1-\alpha L}{K} \sum_{k=0}^{K-1} \mathbb{E} \|\overline{G}_k\|^2 + \frac{1}{K} \sum_{k=0}^{K-1} \mathbb{E} \|\nabla f(\overline{X}_k)\|^2 \leq \frac{2(f(0) - f^*)}{\alpha K} + \frac{\alpha L}{n} \sigma^2 + \frac{L^2}{nK} \sum_{k=0}^{K-1} \sum_{i=1}^n \mathbb{E} \|\overline{X}_k - x_{k,i}\|^2$$

And similar to Moniqua, we have

$$\begin{aligned} & \sum_{k=0}^{K-1} \sum_{i=1}^n \mathbb{E} \|\overline{X}_k - x_{k,i}\|^2 \\ \stackrel{x_{0,i}=0}{=} & \sum_{k=1}^{K-1} \sum_{i=1}^n \mathbb{E} \left\| X_k \left( \frac{\mathbb{1}_n}{n} - e_i \right) \right\|^2 \\ = & \sum_{k=1}^{K-1} \sum_{i=1}^n \mathbb{E} \left\| \left( X_{k-1} \widetilde{W} - \alpha \widetilde{G}_{k-1} + \Omega_{k-1} \right) \left( \frac{\mathbb{1}_n}{n} - e_i \right) \right\|^2 \\ = & \sum_{k=1}^{K-1} \sum_{i=1}^n \mathbb{E} \left\| \sum_{t=0}^{k-1} \left( -\alpha \widetilde{G}_t + \Omega_t \right) \left( \frac{\mathbb{1}_n}{n} - \widetilde{W}^{k-t-1} e_i \right) \right\|^2 \\ \leq & 2\alpha^2 \sum_{k=1}^{K-1} \sum_{i=1}^n \mathbb{E} \left\| \sum_{t=0}^{k-1} \widetilde{G}_t \left( \frac{\mathbb{1}_n}{n} - \widetilde{W}^{k-t-1} e_i \right) \right\|^2 + 2 \sum_{k=1}^{K-1} \sum_{i=1}^n \mathbb{E} \left\| \sum_{t=0}^{k-1} \Omega_t \left( \frac{\mathbb{1}_n}{n} - \widetilde{W}^{k-t-1} e_i \right) \right\|^2 \\ = & 2\alpha^2 \sum_{k=1}^{K-1} \mathbb{E} \left\| \sum_{t=0}^{k-1} \widetilde{G}_t \left( \frac{\mathbb{1}_n \mathbb{1}_n^\top}{n} - \widetilde{W}^{k-t-1} \right) \right\|_F^2 + 2 \sum_{k=1}^{K-1} \mathbb{E} \left\| \sum_{t=0}^{k-1} \Omega_t \left( \frac{\mathbb{1}_n \mathbb{1}_n^\top}{n} - \widetilde{W}^{k-t-1} \right) \right\|_F^2 \\ \leq & 2\alpha^2 \sum_{k=1}^{K-1} \mathbb{E} \left( \sum_{t=0}^{k-1} \rho^{\lfloor \frac{k-t-1}{\mathcal{T}} \rfloor} \left\| \widetilde{G}_t \right\|_F \right)^2 + 2 \sum_{k=1}^{K-1} \mathbb{E} \left( \sum_{t=0}^{k-1} \rho^{\lfloor \frac{k-t-1}{\mathcal{T}} \rfloor} \left\| \Omega_t \right\|_F \right)^2 \\ \leq & \frac{2\alpha^2 \mathcal{T}^2}{(1-\rho)^2} \sum_{k=1}^{K-1} \mathbb{E} \left\| \widetilde{G}_k \right\|_F^2 + \frac{2\mathcal{T}^2}{(1-\rho)^2} \sum_{k=1}^{K-1} \mathbb{E} \left\| \Omega_k \right\|_F^2 \end{aligned}$$

$$\leq \frac{2\alpha^2\mathcal{T}^2}{(1-\rho)^2} \left( n\sigma^2K + 3L^2 \sum_{k=0}^{K-1} \sum_{i=1}^n \mathbb{E} \|\bar{X}_k - x_{k,i}\|^2 + 3n\varsigma^2K + 3n \sum_{k=0}^{K-1} \mathbb{E} \|\nabla f(\bar{X}_k)\|^2 \right) + \frac{2\mathcal{T}^2}{(1-\rho)^2} \sum_{k=1}^{K-1} \mathbb{E} \|\Omega_k\|_F^2$$

Rearrange the terms, we have

$$\begin{aligned} & \left( 1 - \frac{6\alpha^2\mathcal{T}^2L^2}{(1-\rho)^2} \right) \sum_{k=0}^{K-1} \sum_{i=1}^n \mathbb{E} \|\bar{X}_k - x_{k,i}\|^2 \\ & \leq \frac{2\alpha^2\mathcal{T}^2}{(1-\rho)^2} \left( n\sigma^2K + 3n\varsigma^2K + 3n \sum_{k=0}^{K-1} \mathbb{E} \|\nabla f(\bar{X}_k)\|^2 \right) + \frac{2\mathcal{T}^2}{(1-\rho)^2} \sum_{k=1}^{K-1} \mathbb{E} \|\Omega_k\|_F^2 \end{aligned}$$

Let  $M_1 = 1 - \frac{6\alpha^2\mathcal{T}^2L^2}{(1-\rho)^2} > 0$ , we have

$$\sum_{k=0}^{K-1} \sum_{i=1}^n \mathbb{E} \|\bar{X}_k - x_{k,i}\|^2 \leq \frac{2\alpha^2\mathcal{T}^2}{M_1(1-\rho)^2} \left( n\sigma^2K + 3n\varsigma^2K + 3n \sum_{k=0}^{K-1} \mathbb{E} \|\nabla f(\bar{X}_k)\|^2 \right) + \frac{2\mathcal{T}^2}{M_1(1-\rho)^2} \sum_{k=1}^{K-1} \mathbb{E} \|\Omega_k\|_F^2$$

And

$$\frac{L^2}{nK} \sum_{k=0}^{K-1} \sum_{i=1}^n \mathbb{E} \|\bar{X}_k - x_{k,i}\|^2 \leq \frac{2\alpha^2\mathcal{T}^2L^2}{M_1(1-\rho)^2} \left( \sigma^2 + 3\varsigma^2 + \frac{3}{K} \sum_{k=0}^{K-1} \mathbb{E} \|\nabla f(\bar{X}_k)\|^2 \right) + \frac{2\mathcal{T}^2L^2}{M_1nK(1-\rho)^2} \sum_{k=1}^{K-1} \mathbb{E} \|\Omega_k\|_F^2$$

Pushing it back we obtain

$$\begin{aligned} & \frac{1-\alpha L}{K} \sum_{k=0}^{K-1} \mathbb{E} \|\bar{G}_k\|^2 + \frac{1}{K} \sum_{k=0}^{K-1} \mathbb{E} \|\nabla f(\bar{X}_k)\|^2 \\ & \leq \frac{2(f(0) - f^*)}{\alpha K} + \frac{\alpha L}{n} \sigma^2 + \frac{2\alpha^2\mathcal{T}^2L^2}{M_1(1-\rho)^2} \left( \sigma^2 + 3\varsigma^2 + \frac{3}{K} \sum_{k=0}^{K-1} \mathbb{E} \|\nabla f(\bar{X}_k)\|^2 \right) + \frac{2\mathcal{T}^2L^2}{M_1nK(1-\rho)^2} \sum_{k=1}^{K-1} \mathbb{E} \|\Omega_k\|_F^2 \end{aligned}$$

where

$$M_1 = 1 - \frac{6\alpha^2\mathcal{T}^2L^2}{(1-\rho)^2}$$

Rearrange the terms, we get

$$\begin{aligned} & \frac{1-\alpha L}{K} \sum_{k=0}^{K-1} \mathbb{E} \|\bar{G}_k\|^2 + \left( 1 - \frac{6\alpha^2\mathcal{T}^2L^2}{M_1(1-\rho)^2} \right) \frac{1}{K} \sum_{k=0}^{K-1} \mathbb{E} \|\nabla f(\bar{X}_k)\|^2 \\ & \leq \frac{2(f(0) - f^*)}{\alpha K} + \frac{\alpha L}{n} \sigma^2 + \frac{2\alpha^2\mathcal{T}^2L^2(\sigma^2 + 3\varsigma^2)}{M_1(1-\rho)^2} + \frac{2\mathcal{T}^2L^2}{M_1nK(1-\rho)^2} \sum_{k=1}^{K-1} \mathbb{E} \|\Omega_k\|_F^2 \end{aligned}$$

Let

$$M_2 = 1 - \frac{6\alpha^2\mathcal{T}^2L^2}{M_1(1-\rho)^2}$$

we get

$$\begin{aligned} & \frac{1-\alpha L}{K} \sum_{k=0}^{K-1} \mathbb{E} \|\bar{G}_k\|^2 + \frac{M_2}{K} \sum_{k=0}^{K-1} \mathbb{E} \|\nabla f(\bar{X}_k)\|^2 \\ & \leq \frac{2(f(0) - f^*)}{\alpha K} + \frac{\alpha L}{n} \sigma^2 + \frac{2\alpha^2\mathcal{T}^2L^2(\sigma^2 + 3\varsigma^2)}{M_1(1-\rho)^2} + \frac{2\mathcal{T}^2L^2}{M_1nK(1-\rho)^2} \sum_{k=1}^{K-1} \mathbb{E} \|\Omega_k\|_F^2 \end{aligned}$$

Since the  $\Omega_k$  term is the same as Moniqua because the  $\eta$  in  $\theta$  and  $\omega$  will compensate with each other.

Pushing it to the  $\Omega_k$ , and let  $M_1, M_2 \geq \frac{1}{2}$  we have

$$\frac{1}{K} \sum_{k=0}^{K-1} \mathbb{E} \|\nabla f(\bar{X}_k)\|^2 \leq \frac{4(f(0) - f^*)}{\alpha K} + \frac{2\alpha L}{n} \sigma^2 + \frac{8\alpha^2\mathcal{T}^2L^2(\sigma^2 + 3\varsigma^2)}{(1-\rho)^2} + \frac{8\alpha^2\mathcal{T}^2B^2L^2}{(1-\rho)^2}$$

By setting  $\alpha = \frac{1}{\varsigma^{\frac{2}{3}} K^{\frac{1}{3}} + \sigma \sqrt{\frac{K}{n}} + 2L}$ , we have

$$\begin{aligned}
\frac{1}{K} \sum_{k=0}^{K-1} \mathbb{E} \|\nabla f(\bar{X}_k)\|^2 &\leq \frac{8(f(0) - f^*)L}{K} + \frac{4\sigma(f(0) - f^* + L/2)}{\sqrt{nK}} + \frac{4\varsigma^{\frac{2}{3}}(f(0) - f^*)}{K^{\frac{2}{3}}} \\
&\quad + \frac{8\mathcal{T}^2 L^2 \sigma^2 n}{(1-\rho)^2(\sigma^2 K + 4nL^2)} + \frac{24\mathcal{T}^2 L^2 \varsigma^{\frac{2}{3}}}{(1-\rho)^2 K^{\frac{2}{3}}} + \frac{8\mathcal{T}^2 L^2 B^2 n}{(1-\rho)^2(\sigma^2 K + 4nL^2)} \\
&\lesssim \frac{1}{K} + \frac{\sigma}{\sqrt{nK}} + \frac{\mathcal{T}^2 \varsigma^{\frac{2}{3}}}{K^{\frac{2}{3}}} + \frac{\mathcal{T}^2 \sigma^2 n}{\sigma^2 K + n} + \frac{\mathcal{T}^2 B^2 n}{\sigma^2 K + n} \\
&= \frac{1}{K} + \frac{\sigma}{\sqrt{nK}} + \frac{\varsigma^{\frac{2}{3}}}{\eta^2 K^{\frac{2}{3}}} + \frac{\sigma^2 n}{\eta^2(\sigma^2 K + n)} + \frac{B^2 n}{\eta^2(\sigma^2 K + n)}
\end{aligned}$$

Now we can see the dependency of asymptotic rate on  $\eta$ .

### F.5 Lemma for D-PSGD

**Lemma 3** *The output of Algorithm 1 has the following bound:*

$$\begin{aligned}
&\frac{1 - \alpha L}{K} \sum_{k=0}^{K-1} \mathbb{E} \|\bar{G}_k\|^2 + \frac{M_2}{K} \sum_{k=0}^{K-1} \mathbb{E} \|\nabla f(\bar{X}_k)\|^2 \\
&\leq \frac{2(f(0) - f^*)}{\alpha K} + \frac{\alpha L}{n} \sigma^2 + \frac{2\alpha^2 L^2 (\sigma^2 + 3\varsigma^2)}{M_1(1-\rho)^2} + \frac{2L^2}{M_1 n K (1-\rho)^2} \sum_{k=1}^{K-1} \mathbb{E} \|\Omega_k\|_F^2
\end{aligned}$$

where

$$M_1 = 1 - \frac{6\alpha^2 L^2}{(1-\rho)^2}, M_2 = 1 - \frac{6\alpha^2 L^2}{M_1(1-\rho)^2}$$

and

$$\Omega_k e_i = \sum_{j=1}^n ((q_{k,j} - x_{k,j}) - (q_{k,i} - x_{k,i})) W_{ji}, \bar{G}_k = \frac{1}{n} \sum_{i=1}^n g_{k,i}$$

**Proof** From Lemma 6, we have

$$\begin{aligned}
&\frac{1 - \alpha L}{K} \sum_{k=0}^{K-1} \mathbb{E} \|\bar{G}_k\|^2 + \frac{1}{K} \sum_{k=0}^{K-1} \mathbb{E} \|\nabla f(\bar{X}_k)\|^2 \\
&\leq \frac{2(f(0) - f^*)}{\alpha K} + \frac{\alpha L}{n} \sigma^2 + \frac{L^2}{nK} \sum_{k=0}^{K-1} \sum_{i=1}^n \mathbb{E} \|\bar{X}_k - x_{k,i}\|^2 \\
&\stackrel{\text{Lemma 4}}{\leq} \frac{2(f(0) - f^*)}{\alpha K} + \frac{\alpha L}{n} \sigma^2 + \frac{2\alpha^2 L^2}{M_1(1-\rho)^2} \left( \sigma^2 + 3\varsigma^2 + \frac{3}{K} \sum_{k=0}^{K-1} \mathbb{E} \|\nabla f(\bar{X}_k)\|^2 \right) \\
&\quad + \frac{2L^2}{M_1 n K (1-\rho)^2} \sum_{k=1}^{K-1} \mathbb{E} \|\Omega_k\|_F^2
\end{aligned}$$

where

$$M_1 = 1 - \frac{6\alpha^2 L^2}{(1-\rho)^2}$$

Rearrange the terms, we get

$$\begin{aligned}
&\frac{1 - \alpha L}{K} \sum_{k=0}^{K-1} \mathbb{E} \|\bar{G}_k\|^2 + \left( 1 - \frac{6\alpha^2 L^2}{M_1(1-\rho)^2} \right) \frac{1}{K} \sum_{k=0}^{K-1} \mathbb{E} \|\nabla f(\bar{X}_k)\|^2 \\
&\leq \frac{2(f(0) - f^*)}{\alpha K} + \frac{\alpha L}{n} \sigma^2 + \frac{2\alpha^2 L^2 (\sigma^2 + 3\varsigma^2)}{M_1(1-\rho)^2} + \frac{2L^2}{M_1 n K (1-\rho)^2} \sum_{k=1}^{K-1} \mathbb{E} \|\Omega_k\|_F^2
\end{aligned}$$

Let

$$M_2 = 1 - \frac{6\alpha^2 L^2}{M_1(1-\rho)^2}$$

we get

$$\begin{aligned} & \frac{1-\alpha L}{K} \sum_{k=0}^{K-1} \mathbb{E} \|\bar{G}_k\|^2 + \frac{M_2}{K} \sum_{k=0}^{K-1} \mathbb{E} \|\nabla f(\bar{X}_k)\|^2 \\ & \leq \frac{2(f(0) - f^*)}{\alpha K} + \frac{\alpha L}{n} \sigma^2 + \frac{2\alpha^2 L^2 (\sigma^2 + 3\varsigma^2)}{M_1(1-\rho)^2} + \frac{2L^2}{M_1 n K (1-\rho)^2} \sum_{k=1}^{K-1} \mathbb{E} \|\Omega_k\|_F^2 \end{aligned}$$

and that completes the proof

**Lemma 4**

$$\frac{L^2}{nK} \sum_{k=0}^{K-1} \sum_{i=1}^n \mathbb{E} \|\bar{X}_k - x_{k,i}\|^2 \leq \frac{2\alpha^2 L^2}{M_1(1-\rho)^2} \left( \sigma^2 + 3\varsigma^2 + \frac{3}{K} \sum_{k=0}^{K-1} \mathbb{E} \|\nabla f(\bar{X}_k)\|^2 \right) + \frac{2L^2}{M_1 n K (1-\rho)^2} \sum_{k=1}^{K-1} \mathbb{E} \|\Omega_k\|_F^2$$

**Proof**

$$\begin{aligned} & \sum_{k=0}^{K-1} \sum_{i=1}^n \mathbb{E} \|\bar{X}_k - x_{k,i}\|^2 \\ & = \sum_{k=1}^{K-1} \sum_{i=1}^n \mathbb{E} \left\| X_k \left( \frac{\mathbb{1}_n}{n} - e_i \right) \right\|^2 \\ & = \sum_{k=1}^{K-1} \sum_{i=1}^n \mathbb{E} \left\| \left( X_{k-1} W - \alpha \tilde{G}_{k-1} + \Omega_{k-1} \right) \left( \frac{\mathbb{1}_n}{n} - e_i \right) \right\|^2 \\ & \stackrel{x_{0,i}=0}{=} \sum_{k=1}^{K-1} \sum_{i=1}^n \mathbb{E} \left\| \sum_{t=0}^{k-1} \left( -\alpha \tilde{G}_t + \Omega_t \right) \left( \frac{\mathbb{1}_n}{n} - W^{k-t-1} e_i \right) \right\|^2 \\ & \leq 2\alpha^2 \sum_{k=1}^{K-1} \sum_{i=1}^n \mathbb{E} \left\| \sum_{t=0}^{k-1} \tilde{G}_t \left( \frac{\mathbb{1}_n}{n} - W^{k-t-1} e_i \right) \right\|^2 + 2 \sum_{k=1}^{K-1} \sum_{i=1}^n \mathbb{E} \left\| \sum_{t=0}^{k-1} \Omega_t \left( \frac{\mathbb{1}_n}{n} - W^{k-t-1} e_i \right) \right\|^2 \\ & = 2\alpha^2 \sum_{k=1}^{K-1} \mathbb{E} \left\| \sum_{t=0}^{k-1} \tilde{G}_t \left( \frac{\mathbb{1}_n \mathbb{1}_n^\top}{n} - W^{k-t-1} \right) \right\|_F^2 + 2 \sum_{k=1}^{K-1} \mathbb{E} \left\| \sum_{t=0}^{k-1} \Omega_t \left( \frac{\mathbb{1}_n \mathbb{1}_n^\top}{n} - W^{k-t-1} \right) \right\|_F^2 \\ & \stackrel{\text{Lemma 8}}{\leq} 2\alpha^2 \sum_{k=1}^{K-1} \mathbb{E} \left( \sum_{t=0}^{k-1} \rho^{k-t-1} \|\tilde{G}_t\|_F \right)^2 + 2 \sum_{k=1}^{K-1} \mathbb{E} \left( \sum_{t=0}^{k-1} \rho^{k-t-1} \|\Omega_t\|_F \right)^2 \\ & \stackrel{\text{Lemma 7}}{\leq} \frac{2\alpha^2}{(1-\rho)^2} \sum_{k=1}^{K-1} \mathbb{E} \|\tilde{G}_k\|_F^2 + \frac{2}{(1-\rho)^2} \sum_{k=1}^{K-1} \mathbb{E} \|\Omega_k\|_F^2 \\ & \stackrel{\text{Lemma 5}}{\leq} \frac{2\alpha^2}{(1-\rho)^2} \left( n\sigma^2 K + 3L^2 \sum_{k=0}^{K-1} \sum_{i=1}^n \mathbb{E} \|\bar{X}_k - x_{k,i}\|^2 + 3n\varsigma^2 K + 3n \sum_{k=0}^{K-1} \mathbb{E} \|\nabla f(\bar{X}_k)\|^2 \right) + \frac{2}{(1-\rho)^2} \sum_{k=1}^{K-1} \mathbb{E} \|\Omega_k\|_F^2 \end{aligned}$$

Rearrange the terms, we have

$$\begin{aligned} & \left( 1 - \frac{6\alpha^2 L^2}{(1-\rho)^2} \right) \sum_{k=0}^{K-1} \sum_{i=1}^n \mathbb{E} \|\bar{X}_k - x_{k,i}\|^2 \\ & \leq \frac{2\alpha^2}{(1-\rho)^2} \left( n\sigma^2 K + 3n\varsigma^2 K + 3n \sum_{k=0}^{K-1} \mathbb{E} \|\nabla f(\bar{X}_k)\|^2 \right) + \frac{2}{(1-\rho)^2} \sum_{k=1}^{K-1} \mathbb{E} \|\Omega_k\|_F^2 \end{aligned}$$

Let  $M_1 = 1 - \frac{6\alpha^2 L^2}{(1-\rho)^2} > 0$ , we have

$$\sum_{k=0}^{K-1} \sum_{i=1}^n \mathbb{E} \|\bar{X}_k - x_{k,i}\|^2 \leq \frac{2\alpha^2}{M_1(1-\rho)^2} \left( n\sigma^2 K + 3n\varsigma^2 K + 3n \sum_{k=0}^{K-1} \mathbb{E} \|\nabla f(\bar{X}_k)\|^2 \right) + \frac{2}{M_1(1-\rho)^2} \sum_{k=1}^{K-1} \mathbb{E} \|\Omega_k\|_F^2$$

And

$$\frac{L^2}{nK} \sum_{k=0}^{K-1} \sum_{i=1}^n \mathbb{E} \|\bar{X}_k - x_{k,i}\|^2 \leq \frac{2\alpha^2 L^2}{M_1(1-\rho)^2} \left( \sigma^2 + 3\varsigma^2 + \frac{3}{K} \sum_{k=0}^{K-1} \mathbb{E} \|\nabla f(\bar{X}_k)\|^2 \right) + \frac{2L^2}{M_1 n K (1-\rho)^2} \sum_{k=1}^{K-1} \mathbb{E} \|\Omega_k\|_F^2$$

**Lemma 5**

$$\sum_{k=0}^{K-1} \mathbb{E} \|\tilde{G}_k\|_F^2 \leq n\sigma^2 K + 3L^2 \sum_{k=0}^{K-1} \sum_{i=1}^n \mathbb{E} \|\bar{X}_k - x_{k,i}\|^2 + 3n\varsigma^2 K + 3n \sum_{k=0}^{K-1} \mathbb{E} \|\nabla f(\bar{X}_k)\|^2$$

**Proof** From the property of Frobenius norm, we have

$$\mathbb{E} \|\tilde{G}_k\|_F^2 = \sum_{i=1}^n \mathbb{E} \|\tilde{g}_{k,i}\|^2$$

Next, we derive the upper bound of  $\mathbb{E} \|\tilde{g}_{k,i}\|^2$

$$\begin{aligned} & \mathbb{E} \|\tilde{g}_{k,i}\|^2 \\ &= \mathbb{E} \|\tilde{g}_{k,i} - g_{k,i} + g_{k,i}\|^2 \\ &= \mathbb{E} \|\tilde{g}_{k,i} - g_{k,i}\|^2 + \mathbb{E} \|g_{k,i}\|^2 + 2\mathbb{E} \langle \tilde{g}_{k,i} - g_{k,i}, g_{k,i} \rangle \\ &= \mathbb{E} \|\tilde{g}_{k,i} - g_{k,i}\|^2 + \mathbb{E} \|g_{k,i}\|^2 \\ &\leq \sigma^2 + 3\mathbb{E} \|g_{k,i} - \nabla f_i(\bar{X}_k)\|^2 + 3\mathbb{E} \|\nabla f_i(\bar{X}_k) - \nabla f(\bar{X}_k)\|^2 + 3\mathbb{E} \|\nabla f(\bar{X}_k)\|^2 \\ &\leq \sigma^2 + 3L^2 \mathbb{E} \|\bar{X}_k - x_{k,i}\|^2 + 3\varsigma^2 + 3\mathbb{E} \|\nabla f(\bar{X}_k)\|^2 \end{aligned}$$

Summing from  $k = 0$  to  $K - 1$ , we obtain

$$\begin{aligned} & \sum_{k=0}^{K-1} \mathbb{E} \|\tilde{G}_k\|_F^2 \\ &= \sum_{k=0}^{K-1} \sum_{i=1}^n \mathbb{E} \|\tilde{g}_{k,i}\|^2 \\ &\leq \sum_{k=0}^{K-1} \sum_{i=1}^n \sigma^2 + 3L^2 \sum_{k=0}^{K-1} \sum_{i=1}^n \mathbb{E} \|\bar{X}_k - x_{k,i}\|^2 + 3 \sum_{k=0}^{K-1} \sum_{i=1}^n \varsigma^2 + 3 \sum_{k=0}^{K-1} \sum_{i=1}^n \mathbb{E} \|\nabla f(\bar{X}_k)\|^2 \\ &= n\sigma^2 K + 3L^2 \sum_{k=0}^{K-1} \sum_{i=1}^n \mathbb{E} \|\bar{X}_k - x_{k,i}\|^2 + 3n\varsigma^2 K + 3n \sum_{k=0}^{K-1} \mathbb{E} \|\nabla f(\bar{X}_k)\|^2 \end{aligned}$$

That completes the proof

**Lemma 6**

$$\frac{1-\alpha L}{K} \sum_{k=0}^{K-1} \mathbb{E} \|\bar{G}_k\|^2 + \frac{1}{K} \sum_{k=0}^{K-1} \mathbb{E} \|\nabla f(\bar{X}_k)\|^2 \leq \frac{2(f(0) - f^*)}{\alpha K} + \frac{\alpha L}{n} \sigma^2 + \frac{L^2}{nK} \sum_{k=0}^{K-1} \sum_{i=1}^n \mathbb{E} \|\bar{X}_k - x_{k,i}\|^2$$

**Proof** Let  $\mathbb{1}_n$  denote a  $n$ -dimensional vector with all the entries be 1. And we have

$$\bar{X}_{k+1} = (X_k W - \alpha \tilde{G}_k + \Omega_k) \frac{\mathbb{1}_n}{n} = \bar{X}_k - \alpha \bar{\tilde{G}}_k + (Q_k - X_k)(W - I) \frac{\mathbb{1}_n}{n} = \bar{X}_k - \alpha \bar{\tilde{G}}_k$$

And by Taylor Expansion, we have

$$\begin{aligned} \mathbb{E} f(\bar{X}_{k+1}) &= \mathbb{E} f \left( \frac{(X_k W - \alpha \tilde{G}_k + \Omega_k) \mathbb{1}_n}{n} \right) \\ &= \mathbb{E} f \left( \bar{X}_k - \alpha \bar{\tilde{G}}_k \right) \\ &\leq \mathbb{E} f(\bar{X}_k) - \alpha \mathbb{E} \langle \nabla f(\bar{X}_k), \bar{\tilde{G}}_k \rangle + \frac{\alpha^2 L}{2} \mathbb{E} \|\bar{\tilde{G}}_k\|^2 \end{aligned}$$

And for the last term, we have

$$\begin{aligned}
\mathbb{E} \left\| \bar{G}_k \right\|^2 &= \mathbb{E} \left\| \frac{\sum_{i=1}^n \tilde{g}_{k,i}}{n} \right\|^2 \\
&= \mathbb{E} \left\| \frac{\sum_{i=1}^n \tilde{g}_{k,i} - \sum_{i=1}^n g_{k,i}}{n} + \frac{\sum_{i=1}^n g_{k,i}}{n} \right\|^2 \\
&= \mathbb{E} \left\| \frac{\sum_{i=1}^n \tilde{g}_{k,i} - \sum_{i=1}^n g_{k,i}}{n} \right\|^2 + \mathbb{E} \left\| \frac{\sum_{i=1}^n g_{k,i}}{n} \right\|^2 \\
&\quad + \mathbb{E} \left\langle \frac{\sum_{i=1}^n \tilde{g}_{k,i} - \sum_{i=1}^n g_{k,i}}{n} + \frac{\sum_{i=1}^n g_{k,i}}{n} \right\rangle \\
&= \mathbb{E} \left\| \frac{\sum_{i=1}^n \tilde{g}_{k,i} - \sum_{i=1}^n g_{k,i}}{n} \right\|^2 + \mathbb{E} \left\| \frac{\sum_{i=1}^n g_{k,i}}{n} \right\|^2 \\
&\stackrel{\text{Assumption 3}}{=} \frac{1}{n^2} \sum_{i=1}^n \mathbb{E} \|\tilde{g}_{k,i} - g_{k,i}\|^2 + \mathbb{E} \left\| \frac{\sum_{i=1}^n g_{k,i}}{n} \right\|^2 \\
&\stackrel{\text{Assumption 3}}{\leq} \frac{\sigma^2}{n} + \mathbb{E} \left\| \frac{\sum_{i=1}^n g_{k,i}}{n} \right\|^2
\end{aligned}$$

Putting it back, we obtain

$$\begin{aligned}
\mathbb{E} f(\bar{X}_{k+1}) &\leq \mathbb{E} f(\bar{X}_k) - \alpha \mathbb{E} \langle \nabla f(\bar{X}_k), \bar{G}_k \rangle + \frac{\alpha^2 L}{2n} \sigma^2 + \frac{\alpha^2 L}{2} \mathbb{E} \left\| \frac{\sum_{i=1}^n g_{k,i}}{n} \right\|^2 \\
&= \mathbb{E} f(\bar{X}_k) - \frac{\alpha - \alpha^2 L}{2} \mathbb{E} \|\bar{G}_k\|^2 - \frac{\alpha}{2} \mathbb{E} \|\nabla f(\bar{X}_k)\|^2 + \frac{\alpha^2 L}{2n} \sigma^2 \\
&\quad + \frac{\alpha}{2} \mathbb{E} \|\nabla f(\bar{X}_k) - \bar{G}_k\|^2
\end{aligned}$$

where the last step comes from  $2\langle a, b \rangle = \|a\|^2 + \|b\|^2 = \|a - b\|^2$  And

$$\begin{aligned}
\mathbb{E} \|\nabla f(\bar{X}_k) - \bar{G}_k\|^2 &\leq \frac{1}{n} \sum_{i=1}^n \mathbb{E} \left\| \nabla f_i \left( \frac{\sum_{i'=1}^n x_{k,i'}}{n} \right) - \nabla f_i(x_{k,i}) \right\|^2 \\
&\stackrel{\text{Assumption 1}}{\leq} \frac{L^2}{n} \sum_{i=1}^n \mathbb{E} \left\| \frac{\sum_{i'=1}^n x_{k,i'}}{n} - x_{k,i} \right\|^2 \\
&= \frac{L^2}{n} \sum_{i=1}^n \mathbb{E} \|\bar{X}_k - x_{k,i}\|^2
\end{aligned}$$

putting it back, we have

$$\frac{\alpha - \alpha^2 L}{2} \mathbb{E} \|\bar{G}_k\|^2 + \frac{\alpha}{2} \mathbb{E} \|\nabla f(\bar{X}_k)\|^2 \leq \mathbb{E} f(\bar{X}_k) - \mathbb{E} f(\bar{X}_{k+1}) + \frac{\alpha^2 L}{2n} \sigma^2 + \frac{\alpha L^2}{2n} \sum_{i=1}^n \mathbb{E} \|\bar{X}_k - x_{k,i}\|^2$$

summing over from  $k = 0$  to  $K - 1$  on both sides, we have

$$\frac{1 - \alpha L}{K} \sum_{k=0}^{K-1} \mathbb{E} \|\bar{G}_k\|^2 + \frac{1}{K} \sum_{k=0}^{K-1} \mathbb{E} \|\nabla f(\bar{X}_k)\|^2 \leq \frac{2(f(0) - f^*)}{\alpha K} + \frac{\alpha L}{n} \sigma^2 + \frac{L^2}{nK} \sum_{k=0}^{K-1} \sum_{i=1}^n \mathbb{E} \|\bar{X}_k - x_{k,i}\|^2$$

That completes the proof.

**Lemma 7** Given two non-negative sequences  $\{a_t\}_{t=1}^\infty$  and  $\{b_t\}_{t=1}^\infty$  that satisfying

$$a_t = \sum_{s=1}^t \rho^{t-s} b_s$$

with  $0 \leq \rho < 1$ , we have

$$S_k = \sum_{t=1}^k a_t \leq \frac{1}{1 - \rho} \sum_{s=1}^k b_s$$

$$D_k = \sum_{t=1}^k a_t^2 \leq \frac{1}{(1-\rho)^2} \sum_{s=1}^k b_s^2$$

**Proof**

$$\begin{aligned} S_k &= \sum_{t=1}^k a_t = \sum_{t=1}^k \sum_{s=1}^t \rho^{t-s} b_s = \sum_{s=1}^k \sum_{t=s}^k \rho^{t-s} b_s = \sum_{s=1}^k \sum_{t=0}^{k-s} \rho^t b_s \leq \frac{1}{1-\rho} \sum_{s=1}^k b_s \\ D_k &= \sum_{t=1}^k a_t = \sum_{t=1}^k \sum_{s=1}^t \rho^{t-s} b_s \sum_{r=1}^t \rho^{t-r} b_r = \sum_{s=1}^k \sum_{t=s}^k \rho^{t-s} b_s = \sum_{t=1}^k \sum_{s=1}^t \sum_{r=1}^t \rho^{2t-s-r} b_s b_r \\ &\leq \sum_{t=1}^k \sum_{s=1}^t \sum_{r=1}^t \rho^{2t-s-r} \frac{b_s^2 + b_r^2}{2} = \sum_{t=1}^k \sum_{s=1}^t \sum_{r=1}^t \rho^{2t-s-r} b_s^2 \\ &\leq \frac{1}{1-\rho} \sum_{t=1}^k \sum_{s=1}^t \rho^{t-s} b_s^2 \leq \frac{1}{(1-\rho)^2} \sum_{s=1}^k b_s^2 \end{aligned}$$

**Lemma 8** For any  $X_t \in \mathbb{R}^{d \times n}$ , we have

$$\left\| \sum_{t=0}^{k-1} X_t \left( \frac{\mathbb{1}_n \mathbb{1}_n^\top}{n} - W^{k-t-1} \right) \right\|_F^2 \leq \left( \sum_{t=0}^{k-1} \rho^{k-t-1} \|X_t\|_F \right)^2$$

**Proof**

$$\begin{aligned} &\left\| \sum_{t=0}^{k-1} X_t \left( \frac{\mathbb{1}_n \mathbb{1}_n^\top}{n} - W^{k-t-1} \right) \right\|_F^2 \\ &= \left( \left\| \sum_{t=0}^{k-1} X_t \left( \frac{\mathbb{1}_n \mathbb{1}_n^\top}{n} - W^{k-t-1} \right) \right\|_F \right)^2 \\ &\leq \left( \sum_{t=0}^{k-1} \left\| X_t \left( \frac{\mathbb{1}_n \mathbb{1}_n^\top}{n} - W^{k-t-1} \right) \right\|_F \right)^2 \\ &\leq \left( \sum_{t=0}^{k-1} \|X_t\|_F \left\| \frac{\mathbb{1}_n \mathbb{1}_n^\top}{n} - W^{k-t-1} \right\| \right)^2 \\ &\leq \left( \sum_{t=0}^{k-1} \rho^{k-t-1} \|X_t\|_F \right)^2 \end{aligned}$$

That completes the proof.

## G Moniqua on $D^2$ (Proof to Theorem 3)

### G.1 Algorithm and Assumptions

---

**Algorithm 2** Moniqua with Variance Reduction on worker  $i$

---

**Input:** initial point  $x_{0,i} = x_0$ , step size  $\alpha$ , communication matrix  $W$ , number of iterations  $K$ , neighbor list of worker  $i$ :  $\mathcal{N}_i$

- 1: **for**  $k = 0, 1, 2, \dots, K - 1$  **do**
- 2:   Randomly sample data  $\xi_{k,i}$  from local memory
- 3:   Compute a local stochastic gradient based on  $\xi_{k,i}$  and current weight  $x_{k,i}$ :  $\tilde{g}_{k,i}$
- 4:   **if**  $k = 0$  **then**
- 5:     Update local weight:
 
$$x_{k+\frac{1}{2},i} \leftarrow x_{k,i} - \alpha \tilde{g}_{k,i}$$
- 6:   **else**
- 7:     Update local weight:
 
$$x_{k+\frac{1}{2},i} \leftarrow 2x_{k,i} - x_{k-1,i} - \alpha \tilde{g}_{k,i} + \alpha \tilde{g}_{k-1,i}$$
- 8:   **end if**
- 9:   Make the exchanged information  $q_{k,i}$  available to all the neighbors.
- 10:   **for**  $j \in \mathcal{N}_i$  **do**
- 11:     Fetch  $q_{k,j}$  from neighbor  $j$  and subtract the biased term  $q_{k,i}$  proportionally:
 
$$x_{k+1,i} \leftarrow x_{k+\frac{1}{2},i} + q_{k,j}W_{ji} - q_{k,i}W_{ji}$$
- 12:   **end for**
- 13: **end for**

**Output:**  $\bar{X}_K = \frac{1}{n} \sum_{i=1}^n x_{K,i}$

---

$D^2$  makes the following assumptions (1-4), and we add the additional assumption (5):

1. **Lipschitzian Gradient:** All the function  $f_i$  have L-Lipschitzian gradients.
2. **Communication Matrix:** Communication matrix  $W$  is a symmetric doubly stochastic matrix. Let the eigenvalues of  $W \in \mathbb{R}^{n \times n}$  be  $\lambda_1 \geq \dots \geq \lambda_n$ . We assume  $\lambda_2 < 1$ ,  $\lambda_n > -\frac{1}{3}$ .
3. **Bounded Variance:**

$$\mathbb{E}_{\xi \sim \mathcal{D}_i} \left\| \nabla \tilde{f}_i(x_i; \xi_i) - \nabla f_i(x) \right\|^2 \leq \sigma^2, \forall i$$

where  $\nabla \tilde{f}_i(x; \xi_i)$  denotes gradient sample on worker  $i$  computed via data sample  $\xi_i$ .
4. **Initialization:** All the models are initialized by the same parameters:  $x_{0,i} = x_0, \forall i$  and with out the loss of generality  $x_0 = 0$ .
5. **Gradient magnitude:** The norm of a sampled gradient is bounded by  $\|\tilde{g}_{k,i}\| \leq B$  for some constant  $B$ .

### G.2 Theorems

We highlight all the theorems there:

**Theorem 2** If we apply quantizer  $\mathcal{Q}_\omega$  to the communication as described in Theorem 2, by setting hyperparameters to

$$\theta = (12nC_5 + 4)\alpha B, \quad \omega = \frac{1}{4nC_6}, \quad \text{and} \quad \alpha = \frac{1}{\sigma\sqrt{K/n + 2L}},$$

where definitions of  $C_5$  and  $C_6$  can be found in Lemma 9, applying Moniqua to  $D^2$  gives the following asymptotic convergence rate:

$$\frac{1}{K} \sum_{k=0}^{K-1} \mathbb{E} \left\| \nabla f(\bar{X}_k) \right\|^2 \lesssim \frac{1}{K} + \frac{\sigma}{\sqrt{nK}} + \frac{\sigma^2 n}{\sigma^2 K + n} + \frac{B^2 n}{\sigma^2 K + n}.$$

**Corollary 3** *If we use a linear quantizer with quantization step  $\delta$  as  $\mathcal{Q}_\omega$ , the number of bits  $\mathcal{B}$  required per dimension per iteration is upper bounded by  $\mathcal{B} \leq \log(4nC_6\sqrt{d})$ .*

### G.3 Proof to Theorem 2

**Proof** *From a local view, define  $x_{-1} = \tilde{g}_{-1} = 0$ , the update rule of Moniqua on  $D^2$  on worker  $i$  in iteration  $k$  can be written as*

$$\begin{aligned} x_{k+\frac{1}{2},i} &= 2x_{k,i} - x_{k-1,i} - \alpha\tilde{g}_{k,i} + \alpha\tilde{g}_{k-1,i} \\ x_{k+1,i} &= \sum_{j=1}^n x_{k+\frac{1}{2},j} W_{ji} + \sum_{j=1}^n \left( (q_{k,j} - x_{k+\frac{1}{2},j}) - (q_{k,i} - x_{k+\frac{1}{2},i}) \right) W_{ji} \end{aligned}$$

*From a global view, the update rule can be written as*

$$\begin{aligned} X_{k+\frac{1}{2}} &= 2X_k - X_{k-1} - \alpha\tilde{G}_k + \alpha\tilde{G}_{k-1} \\ X_{k+1} &= X_{k+\frac{1}{2}}W + (Q_k - X_{k+\frac{1}{2}})(W - I) \end{aligned}$$

*Define*

$$\Omega_k = (Q_k - X_{k+\frac{1}{2}})(W - I)$$

*Since  $W$  is symmetric, it can be diagonalized as  $W = P\Lambda P^\top$ , where the  $i$ -th column of  $P$  and  $\Lambda$  are  $W$ 's  $i$ -th eigenvector and eigenvalue, respectively. And we obtain*

$$X_{k+1} = 2X_k P\Lambda P^\top - X_{k-1} P\Lambda P^\top - \alpha\tilde{G}_k P\Lambda P^\top + \alpha\tilde{G}_{k-1} P\Lambda P^\top + \Omega_k$$

*and*

$$X_{k+1}P = 2X_k P\Lambda - X_{k-1} P\Lambda - \alpha\tilde{G}_k P\Lambda + \alpha\tilde{G}_{k-1} P\Lambda + \Omega_k P$$

*Denote  $Y_k = X_k P$ ,  $H(X_k; \xi_k) = \tilde{G}_k P$ , and denote  $y_{k,i}$ ,  $h_{k,i}$  and  $r_{k,i}$  as the  $i$ -th column of  $Y_k$ ,  $H_k$  and  $\Omega_k P$ , respectively. Then we have*

$$y_{k+1,i} = \lambda_i(2y_{k,i} - y_{k-1,i} - \alpha h_{k,i} + \alpha h_{k-1,i}) + r_{k,i}$$

*From Lemma 13 (Constants  $C_1$  to  $C_6$  are defined in the Lemma 9 and Lemma 13) we get*

$$\begin{aligned} &\left(1 - \frac{3C_1\alpha^2 L^2}{C_4}\right) \mathbb{E} \|\nabla f(0)\| + \left(1 - \alpha L - 3\frac{C_2}{C_4}\alpha^4 L^4\right) \frac{1}{K} \sum_{k=1}^{K-1} \mathbb{E} \|\bar{G}_k\|^2 + \frac{1}{K} \sum_{k=0}^{K-1} \mathbb{E} \|\nabla f(\bar{X}_k)\|^2 \\ &\leq \frac{2(f(0) - f^*)}{\alpha K} + \frac{\alpha L}{n} \sigma^2 + \frac{3C_1\alpha^2 L^2(\sigma^2 + \varsigma_0^2)}{C_4 K} + 6\frac{C_2}{C_4}\alpha^2 \sigma^2 L^2 + 3\frac{C_2}{nC_4}\alpha^4 \sigma^2 L^4 + \frac{C_3 L^2}{C_4} \left(\frac{12C_5 + 4}{2C_6}\right)^2 \alpha^2 B^2 \end{aligned}$$

*Let  $\alpha = \frac{1}{\sigma\sqrt{K/n+2L}}$ , we have*

$$\begin{aligned} &\frac{1}{K} \sum_{k=0}^{K-1} \mathbb{E} \|\nabla f(\bar{X}_k)\|^2 \\ &\leq \frac{2(f(0) - f^*)}{\alpha K} + \frac{\alpha L}{n} \sigma^2 + \frac{3C_1\alpha^2 L^2(\sigma^2 + \varsigma_0^2)}{C_4 K} + 6\frac{C_2}{C_4}\alpha^2 \sigma^2 L^2 + 3\frac{C_2}{nC_4}\alpha^4 \sigma^2 L^4 + \left(\frac{12C_5 + 4}{2C_6}\right)^2 \frac{C_3 L^2}{C_4} B^2 \alpha^2 \\ &\leq \frac{4(f(0) - f^*)L}{K} + \frac{2\sigma(f(0) - f^* + L/2)}{\sqrt{nK}} + \frac{3C_1 L^2(\sigma^2 + \varsigma_0^2)n}{C_4(\sigma^2 K^2 + 4nL^2 K)} + \frac{6C_2 L^2 \sigma^2 n}{C_4(\sigma^2 K + 4nL^2)} \\ &\quad + \frac{3C_2 n \sigma^2 L^2}{C_4(\sigma^4 K^2 + 16n^2 L^4)} + \left(\frac{12C_5 + 4}{2C_6}\right)^2 \frac{C_3 B^2 L^2 n}{C_4(\sigma^2 K + 4nL^2)} \\ &\lesssim \frac{1}{K} + \frac{\sigma}{\sqrt{nK}} + \frac{(\sigma^2 + \varsigma_0^2)n}{\sigma^2 K^2 + nK} + \frac{\sigma^2 n}{\sigma^2 K + n} + \frac{\sigma^2 n}{\sigma^4 K^2 + n^2} + \frac{B^2 n}{\sigma^2 K + n} \\ &\lesssim \frac{1}{K} + \frac{\sigma}{\sqrt{nK}} + \frac{\sigma^2 n}{\sigma^2 K + n} + \frac{B^2 n}{\sigma^2 K + n} \end{aligned}$$

#### G.4 Proof to Corollary

##### Proof to Corollary 3

**Proof** The number of bits used in the communication per iteration per dimension can be written as  $\log\left(\frac{1}{\delta}\right)$ , note that for linear quantizer,  $\omega = \delta\sqrt{d}$ , so we have number of bits is upper bounded by  $\log\left(\frac{1}{\delta}\right) = \log\left(\frac{\sqrt{d}}{\omega}\right) = \log\left(4nC_6\sqrt{d}\right)$

#### G.5 Lemma for $D^2$

**Lemma 9** Define

$$C_5 = \max \left\{ |v_n| + \frac{2|\lambda_n|}{1-|v_n|}, \sqrt{\frac{\lambda_2}{1-\lambda_2}} + \frac{2\lambda_2}{1-\lambda_2} \right\}$$

$$C_6 = \max \left\{ \frac{2}{1-|v_n|}, \frac{2}{\sqrt{1-\lambda_2}} \right\}$$

Let  $\omega = \frac{1}{4nC_6}$ , and we have <sup>6</sup> for  $\forall i, j$

$$\left\| x_{k+\frac{1}{2}}(e_i - e_j) \right\| \leq (12nC_5 + 4)\alpha B$$

We now use mathematical induction to prove this inequality.

**Proof** First, when  $k = 0$ ,

$$\left\| X_{0+\frac{1}{2}}(e_i - e_j) \right\| = \left\| -\alpha \tilde{G}_0(e_i - e_j) \right\| \leq \alpha \left\| \tilde{G}_0 \right\|_{2 \leftarrow 1} \|e_i - e_j\|_1 \leq 2\alpha B \leq (12nC_5 + 4)\alpha B$$

Next, suppose we know for some  $k \geq 0$ ,  $\forall t \leq k$ , we have  $\left\| X_{t+\frac{1}{2}}(e_i - e_j) \right\| \leq (12nC_5 + 4)\alpha B$ , now we prove  $\left\| X_{(k+1)+\frac{1}{2}}(e_i - e_j) \right\| \leq (12nC_5 + 4)\alpha B$

Now, for  $\forall i, j$

$$\begin{aligned} & \left\| X_{k+1}(e_i - e_j) \right\| \\ & \leq \left\| X_{k+1} \left( \frac{\mathbb{1}_n}{n} - e_i \right) \right\| + \left\| X_{k+1} \left( \frac{\mathbb{1}_n}{n} - e_j \right) \right\| \\ & \leq 2 \left\| X_{k+1} \left( \frac{\mathbb{1}_n \mathbb{1}_n^\top}{n} - I \right) \right\| \\ & \leq 2 \left\| X_{k+1} \left( \frac{\mathbb{1}_n \mathbb{1}_n^\top}{n} - I \right) \right\|_F \\ & = 2 \left\| X_{k+1} P P^\top - X_{k+1} v_1 v_1^\top \right\|_F \\ & \stackrel{\text{Lemma 12}}{=} 2 \left\| X_{k+1} P \begin{bmatrix} 0 & 0 & 0 & \dots & 0 \\ 0 & 1 & 0 & \dots & 0 \\ 0 & 0 & 1 & \dots & 0 \\ \vdots & \vdots & \vdots & \ddots & \vdots \\ 0 & 0 & 0 & \dots & 1 \end{bmatrix} \right\|_F \\ & \leq 2 \sum_{i=2}^n \|y_{k+1,i}\| \end{aligned}$$

From the update rule, we have

$$y_{k+1,i} = \lambda_i(2y_{k,i} - y_{k-1,i} - \alpha h_{k,i} + \alpha h_{k-1,i}) + r_{k,i} = \lambda_i(2y_{k,i} - y_{k-1,i}) + \lambda_i \beta_{k,i} + r_{k,i}$$

<sup>6</sup>Since  $\left\| X_{k+\frac{1}{2}}(e_i - e_j) \right\|_\infty \leq \left\| X_{k+\frac{1}{2}}(e_i - e_j) \right\|_2$  and  $\left\| X_{k+\frac{1}{2}}(e_i - e_j) \right\|_2$  is easier to analyze, so we prove  $\left\| X_{k+\frac{1}{2}}(e_i - e_j) \right\|_2 \leq \theta$  that will automatically hold for  $\left\| X_{k+\frac{1}{2}}(e_i - e_j) \right\|_\infty \leq \theta$ .

where  $\beta_{k,i} = -\alpha h_{k,i} + \alpha h_{k-1,i}$ , for all  $y_i$  with  $-\frac{1}{3} < \lambda_i < 0$ , from Lemma 11 we have

$$y_{k+1,i} = y_{1,i} \left( \frac{u_i^{k+1} - v_i^{k+1}}{u_i - v_i} \right) + \sum_{s=1}^k (\lambda_i \beta_{s,i} + r_{s,i}) \frac{u_i^{k-s+1} - v_i^{k-s+1}}{u_i - v_i}$$

where  $u_i = \lambda_i + \sqrt{\lambda_i^2 - \lambda_i}$  and  $v_i = \lambda_i - \sqrt{\lambda_i^2 - \lambda_i}$ , we obtain

$$\|y_{k+1,i}\| \leq \|y_{1,i}\| \left| \frac{u_i^{k+1} - v_i^{k+1}}{u_i - v_i} \right| + |\lambda_i| \sum_{s=1}^k \|\beta_{s,i}\| \left| \frac{u_i^{k-s+1} - v_i^{k-s+1}}{u_i - v_i} \right| + \sum_{s=1}^k \|r_{s,i}\| \left| \frac{u_i^{k-s+1} - v_i^{k-s+1}}{u_i - v_i} \right|$$

Since

$$\left| \frac{u_i^{n+1} - v_i^{n+1}}{u_i - v_i} \right| \leq |v_i|^n \left| \frac{u_i \left( \frac{u_i}{v_i} \right)^n - v_i}{u_i - v_i} \right| \leq |v_i|^n$$

We obtain

$$\|y_{k+1,i}\| \leq \|y_{1,i}\| |v_i|^k + |\lambda_i| \sum_{s=1}^k \|\beta_{s,i}\| |v_i|^{k-s} + \sum_{s=1}^k \|r_{s,i}\| |v_i|^{k-s}$$

For  $\beta_{k,i}$ , we have

$$\begin{aligned} & \sum_{i=2}^n \|\beta_{k,i}\| \\ &= \sum_{i=2}^n \|-\alpha h_{k,i} + \alpha h_{k-1,i}\| \\ &\stackrel{\text{Lemma 12}}{\leq} \alpha \sqrt{n} (\|G_k\|_F + \|G_{k-1}\|_F) \\ &\leq 2\alpha n B \end{aligned}$$

Similarly, we have

$$\sum_{i=2}^n \|r_{k,i}\| \leq \sum_{i=2}^n \|\Omega_k P e_i\| \stackrel{\text{Lemma 12}}{\leq} \sqrt{n} \|\Omega_k\|_F \leq 2n\omega\theta$$

The last step is because: for  $\forall i$

$$\begin{aligned} & \|\Omega_k e_i\| \\ &\leq \left\| \sum_{j=1}^n ((q_{k,j} - x_{k,j}) - (q_{k,i} - x_{k,i})) W_{ji} \right\| \\ &\leq \sum_{j=1}^n W_{ji} \|(q_{k,j} - x_{k,j}) - (q_{k,i} - x_{k,i})\| \\ &\leq \sum_{j=1}^n W_{ji} \left\| \theta \mathcal{Q} \left( \frac{x_{k,j}}{\theta} \mod 1 \right) - \theta \mathcal{Q} \left( \frac{x_{k,i}}{\theta} \mod 1 \right) - (x_{k,j} - x_{k,i}) \right\| \\ &\leq \sum_{j=1}^n W_{ji} \left\| \theta \mathcal{Q} \left( \frac{x_{k,j}}{\theta} \mod 1 \right) - \theta \mathcal{Q} \left( \frac{x_{k,j}}{\theta} \mod 1 \right) - \theta \left( \frac{x_{k,j} - x_{k,i}}{\theta} \mod 1 \right) \right\| \\ &\leq \sum_{j=1}^n W_{ji} \left\| \theta \mathcal{Q} \left( \frac{x_{k,j}}{\theta} \mod 1 \right) - \theta \left( \frac{x_{k,j}}{\theta} \mod 1 \right) - \left( \theta \mathcal{Q} \left( \frac{x_{k,i}}{\theta} \mod 1 \right) - \theta \left( \frac{x_{k,i}}{\theta} \mod 1 \right) \right) \right\| \\ &\leq 2\omega\theta \end{aligned}$$

when  $\lambda_i < 0$ , we have

$$\sum_{i=2}^n \|y_{k+1,i}\| \leq \sum_{i=2}^n \|y_{1,i}\| |v_i|^k + \sum_{i=2}^n |\lambda_i| \sum_{s=1}^k \|\beta_{s,i}\| |v_i|^{k-s} + \sum_{i=2}^n \sum_{s=1}^k \|r_{s,i}\| |v_i|^{k-s}$$

$$\begin{aligned}
&\leq \sum_{i=2}^n \|y_{1,i}\| |v_n|^k + \sum_{i=2}^n |\lambda_n| \sum_{s=1}^k \|\beta_{s,i}\| |v_n|^{k-s} + \sum_{i=2}^n \sum_{s=1}^k \|r_{s,i}\| |v_n|^{k-s} \\
&\leq \alpha n B |v_n|^k + 2\alpha n B |\lambda_n| \sum_{s=1}^{\infty} |v_n|^{k-s} + 2n\omega\theta \sum_{s=1}^{\infty} |v_n|^{k-s} \\
&\leq \alpha n B |v_n|^k + \frac{2\alpha n B |\lambda_n|}{1 - |v_n|} + \frac{2n\omega\theta}{1 - |v_n|}
\end{aligned}$$

where  $v_n = \lambda_n - \sqrt{\lambda_n^2 - \lambda_n}$ .

On the other hand, when  $0 \leq \lambda_i < 1$ , from Lemma 11 we have

$$y_{k+1,i} \sin \theta_i = y_{1,i} \lambda_i^{\frac{k}{2}} \sin[(t+1)\theta_i] + \lambda_i \sum_{s=1}^k \beta_{s,i} \lambda_i^{\frac{k-s}{2}} \sin[(k+1-s)\theta_i] + \sum_{s=1}^k r_{s,i} \lambda_i^{\frac{k-s}{2}} \sin[(k+1-s)\theta_i]$$

By taking norm, we get

$$\begin{aligned}
\sum_{i=2}^n \|y_{k+1,i}\| |\sin \theta_i| &= \sum_{i=2}^n \|y_{1,i}\| \lambda_i^{\frac{k}{2}} |\sin[(t+1)\theta_i]| + \sum_{i=2}^n \lambda_i \sum_{s=1}^k \|\beta_{s,i}\| \lambda_i^{\frac{k-s}{2}} |\sin[(k+1-s)\theta_i]| \\
&\quad + \sum_{i=2}^n \sum_{s=1}^k \|r_{s,i}\| \lambda_i^{\frac{k-s}{2}} |\sin[(k+1-s)\theta_i]| \\
&\leq \sum_{i=2}^n \|y_{1,i}\| \lambda_2^{\frac{k}{2}} + 2\alpha n B \lambda_2 \sum_{s=1}^{\infty} \lambda_2^{\frac{s}{2}} + 2n\omega\theta \sum_{s=1}^{\infty} \lambda_2^{\frac{s}{2}} \\
&\leq \alpha n B \sqrt{\lambda_2} + \frac{2\alpha n B \lambda_2 + 2n\omega\theta}{\sqrt{1 - \lambda_2}}
\end{aligned}$$

Since  $|\sin \theta_i| \geq \sqrt{1 - \lambda_2}$ , putting it back, we get

$$\sum_{i=2}^n \|y_{k+1,i}\| \leq \alpha n B \sqrt{\frac{\lambda_2}{1 - \lambda_2}} + \frac{2\alpha n B \lambda_2 + 2n\omega\theta}{1 - \lambda_2}$$

So there exists  $C_5, C_6$

$$\begin{aligned}
C_5 &= \max \left\{ |v_n| + \frac{2|\lambda_n|}{1 - |v_n|}, \sqrt{\frac{\lambda_2}{1 - \lambda_2}} + \frac{2\lambda_2}{1 - \lambda_2} \right\} \\
C_6 &= \max \left\{ \frac{2}{1 - |v_n|}, \frac{2}{\sqrt{1 - \lambda_2}} \right\}
\end{aligned}$$

such that

$$\sum_{i=2}^n \|y_{k+1,i}\| \leq C_5 \alpha n B + C_6 n \omega \theta$$

Putting it back we have  $\forall i, j$

$$\|X_{k+1}(e_i - e_j)\| \leq 2 \sum_{i=2}^n \|y_{k+1,i}\| \leq 2(C_5 \alpha n B + C_6 n \omega \theta) \leq \frac{2nC_5 \alpha B}{1 - 2nC_6 \omega}$$

As a result

$$\begin{aligned}
&\left\| X_{k+\frac{1}{2}}(e_i - e_j) \right\| \\
&= \left\| (2X_k - X_{k-1} - \alpha \tilde{G}_k + \alpha \tilde{G}_{k-1})(e_i - e_j) \right\| \\
&\leq 2 \|X_k(e_i - e_j)\| + \|X_{k-1}(e_i - e_j)\| + \alpha \left\| \tilde{G}_k \right\|_{2 \leftarrow 1} \|e_i - e_j\|_1 + \alpha \left\| \tilde{G}_{k-1} \right\|_{2 \leftarrow 1} \|e_i - e_j\|_1
\end{aligned}$$

$$\begin{aligned}
&\leq \frac{6nC_5}{1-2nC_6\omega} \alpha B + 4\alpha B \\
&\leq (12nC_5 + 4)\alpha B
\end{aligned}$$

The last step is because  $\omega = \frac{1}{4nC_6}$

That completes the proof.

**Lemma 10**

$$\begin{aligned}
&(1 - 12C_2\alpha^2 L^2) \sum_{i=1}^n \sum_{k=1}^K \mathbb{E} \|\bar{X}_k - x_{k,i}\|^2 \\
&\leq 3C_1\alpha^2 n\sigma^2 + 3C_1\alpha^2 n\zeta_0^2 + 3C_1\alpha^2 n\mathbb{E} \|\nabla f(0)\| + 6C_2\alpha^2 n\sigma^2 K + 3C_2\alpha^4 \sigma^2 L^2 K \\
&+ 3C_2\alpha^4 nL^2 \sum_{k=1}^{K-1} \mathbb{E} \|\bar{G}_k\|^2 + C_3 \sum_{k=1}^{K-1} \mathbb{E} \|\Omega_k\|_F^2
\end{aligned}$$

**Proof**

$$\begin{aligned}
\sum_{i=1}^n \|\bar{X}_k - x_{k,i}\|^2 &= \sum_{i=1}^n \left\| X_k \left( e_i - \frac{\mathbb{1}_n}{n} \right) \right\|^2 \\
&= \left\| X_k \left( I - \frac{\mathbb{1}_n \mathbb{1}_n^\top}{n} \right) \right\|_F^2 \\
&= \|X_k P P^\top - X_k v_1 v_1^\top\|_F^2 \\
&\stackrel{\text{Lemma 12}}{=} \left\| X_k P \begin{bmatrix} 0 & 0 & 0 & \dots & 0 \\ 0 & 1 & 0 & \dots & 0 \\ 0 & 0 & 1 & \dots & 0 \\ \vdots & \vdots & \vdots & \ddots & \vdots \\ 0 & 0 & 0 & \dots & 1 \end{bmatrix} \right\|_F^2 \\
&= \sum_{i=2}^n \|y_{k,i}\|^2
\end{aligned}$$

From the update rule, we obtain,

$$y_{k+1,i} = \lambda_i(2y_{k,i} - y_{k-1,i} - \alpha h_{k,i} + \alpha h_{k-1,i}) + r_{k,i} = \lambda_i(2y_{k,i} - y_{k-1,i}) + \lambda_i \beta_{k,i} + r_{k,i}$$

where  $\beta_{k,i} = -\alpha h_{k,i} + \alpha h_{k-1,i}$ , for all  $y_i$  with  $-\frac{1}{3} < \lambda_i < 0$ , from Lemma 11 we have

$$y_{k+1,i} = y_{1,i} \left( \frac{u_i^{k+1} - v_i^{k+1}}{u_i - v_i} \right) + \sum_{s=1}^k (\lambda_i \beta_{s,i} + r_{k,i}) \frac{u_i^{k-s+1} - v_i^{k-s+1}}{u_i - v_i}$$

where  $u_i = \lambda_i + \sqrt{\lambda_i^2 - \lambda_i}$  and  $v_i = \lambda_i - \sqrt{\lambda_i^2 - \lambda_i}$ , we obtain

$$\begin{aligned}
\|y_{k+1,i}\|^2 &\leq 3 \|y_{1,i}\|^2 \left( \frac{u_i^{k+1} - v_i^{k+1}}{u_i - v_i} \right)^2 + 3\lambda_i^2 \left( \sum_{s=1}^k \|\beta_{s,i}\| \left| \frac{u_i^{k-s+1} - v_i^{k-s+1}}{u_i - v_i} \right| \right)^2 \\
&+ 3 \left( \sum_{s=1}^k \|r_{s,i}\| \left| \frac{u_i^{k-s+1} - v_i^{k-s+1}}{u_i - v_i} \right| \right)^2
\end{aligned}$$

Since

$$\left| \frac{u_i^{n+1} - v_i^{n+1}}{u_i - v_i} \right| \leq |v_i|^n \left| \frac{u_i \left( \frac{u_i}{v_i} \right)^n - v_i}{u_i - v_i} \right| \leq |v_i|^n$$

We obtain

$$\|y_{k+1,i}\|^2 \leq 3 \|y_{1,i}\|^2 |v_i|^{2t} + 3\lambda_i^2 \left( \sum_{s=1}^k \|\beta_{s,i}\| |v_i|^{k-s} \right)^2 + 3 \left( \sum_{s=1}^k \|r_{s,i}\| |v_i|^{k-s} \right)^2$$

Summing over from  $k = 0$  to  $t = K - 1$ , we obtain

$$\begin{aligned}
\sum_{k=0}^{K-1} \|y_{k+1,i}\|^2 &= \sum_{k=1}^K \|y_{k,i}\|^2 \\
&\leq 3 \|y_{1,i}\|^2 \sum_{k=0}^{K-1} |v_i|^{2k} + 3\lambda_i^2 \sum_{k=1}^{K-1} \left( \sum_{s=1}^k \|\beta_{s,i}\| |v_i|^{k-s} \right)^2 + 3 \sum_{k=1}^{K-1} \left( \sum_{s=1}^k \|r_{s,i}\| |v_i|^{k-s} \right)^2 \\
&\leq \frac{3 \|y_{1,i}\|^2}{1 - |v_i|^2} + \frac{3\lambda_i^2}{(1 - |v_i|)^2} \sum_{k=1}^{K-1} \|\beta_{k,i}\|^2 + \frac{3}{(1 - |v_i|)^2} \sum_{k=1}^{K-1} \|r_{k,i}\|^2 \\
&\leq \frac{3 \|y_{1,i}\|^2}{1 - |v_n|^2} + \frac{3\lambda_n^2}{(1 - |v_n|)^2} \sum_{k=1}^{K-1} \|\beta_{k,i}\|^2 + \frac{3}{(1 - |v_n|)^2} \sum_{k=1}^{K-1} \|r_{k,i}\|^2
\end{aligned}$$

where  $v_n = \lambda_n - \sqrt{\lambda_n^2 - \lambda_n}$ .

On the other hand, when  $0 \leq \lambda_i < 1$ , from Lemma 11 we have

$$y_{k+1,i} \sin \theta_i = y_{1,i} \lambda_i^{\frac{k}{2}} \sin[(t+1)\theta_i] + \lambda_i \sum_{s=1}^k \beta_{s,i} \lambda_i^{\frac{k-s}{2}} \sin[(k+1-s)\theta_i] + \sum_{s=1}^k r_{s,i} \lambda_i^{\frac{k-s}{2}} \sin[(k+1-s)\theta_i]$$

And we have

$$\begin{aligned}
\|y_{k+1,i}\|^2 \sin^2 \theta_i &\leq 3 \|y_{1,i}\|^2 \lambda_i^k \sin^2[(t+1)\theta_i] + 3\lambda_i^2 \left( \sum_{s=1}^k \beta_{s,i} \lambda_i^{\frac{k-s}{2}} \sin[(k+1-s)\theta_i] \right)^2 \\
&\quad + 3 \left( \sum_{s=1}^k r_{s,i} \lambda_i^{\frac{k-s}{2}} \sin[(k+1-s)\theta_i] \right)^2 \\
&\leq 3 \|y_{1,i}\|^2 \lambda_i^k + 3\lambda_i^2 \left( \sum_{s=1}^k \beta_{s,i} \lambda_i^{\frac{k-s}{2}} \right)^2 + 3 \left( \sum_{s=1}^k r_{s,i} \lambda_i^{\frac{k-s}{2}} \right)^2
\end{aligned}$$

Summing from  $k = 0$  to  $K - 1$ , we have

$$\begin{aligned}
\sum_{k=0}^{K-1} \|y_{k+1,i}\|^2 \sin^2 \theta_i &= \sum_{k=1}^K \|y_{k,i}\|^2 \sin^2 \theta_i \\
&\leq 3 \|y_{1,i}\|^2 \sum_{k=0}^{K-1} \lambda_i^k + 3\lambda_i^2 \sum_{k=1}^{K-1} \left( \sum_{s=1}^k \|\beta_{s,i}\| \lambda_i^{\frac{k-s}{2}} \right)^2 + 3 \sum_{k=1}^{K-1} \left( \sum_{s=1}^k r_{s,i} \lambda_i^{\frac{k-s}{2}} \right)^2 \\
&\leq \frac{3 \|y_{1,i}\|^2}{1 - \lambda_i} + \frac{3\lambda_i^2}{(1 - \sqrt{\lambda_i})^2} \sum_{k=1}^{K-1} \|\beta_{k,i}\|^2 + \frac{3}{(1 - \sqrt{\lambda_i})^2} \sum_{k=1}^{K-1} \|r_{k,i}\|^2
\end{aligned}$$

Since  $\sin^2 \theta_i = 1 - \lambda_i$ , we have

$$\begin{aligned}
\sum_{k=1}^K \|y_{k,i}\|^2 &\leq \frac{3 \|y_{1,i}\|^2}{(1 - \lambda_i)^2} + \frac{3\lambda_i^2}{(1 - \sqrt{\lambda_i})^2(1 - \lambda_i)} \sum_{k=1}^{K-1} \|\beta_{k,i}\|^2 + \frac{3}{(1 - \sqrt{\lambda_i})^2(1 - \lambda_i)} \sum_{k=1}^{K-1} \|r_{k,i}\|^2 \\
&\leq \frac{3 \|y_{1,i}\|^2}{(1 - \lambda_2)^2} + \frac{3\lambda_2^2}{(1 - \sqrt{\lambda_2})^2(1 - \lambda_2)} \sum_{k=1}^{K-1} \|\beta_{k,i}\|^2 + \frac{3}{(1 - \sqrt{\lambda_2})^2(1 - \lambda_2)} \sum_{k=1}^{K-1} \|r_{k,i}\|^2
\end{aligned}$$

So there exists  $C_1, C_2, C_3$

$$C_1 = \max \left\{ \frac{3}{1 - |v_n|^2}, \frac{3}{(1 - \lambda_2)^2} \right\}$$

$$C_2 = \max \left\{ \frac{3\lambda_n^2}{(1-|v_n|)^2}, \frac{3\lambda_2^2}{(1-\sqrt{\lambda_2})^2(1-\lambda_2)} \right\}$$

$$C_3 = \max \left\{ \frac{3}{(1-|v_n|)^2}, \frac{3}{(1-\sqrt{\lambda_2})^2(1-\lambda_2)} \right\}$$

$$\sum_{k=1}^K \|y_{k,i}\|^2 \leq C_1 \|y_{1,i}\|^2 + C_2 \sum_{k=1}^{K-1} \|\beta_{k,i}\|^2 + C_3 \sum_{k=1}^{K-1} \|r_{k,i}\|^2$$

By taking expectation we have

$$\sum_{k=1}^K \mathbb{E} \|y_{k,i}\|^2 \leq C_1 \mathbb{E} \|y_{1,i}\|^2 + C_2 \sum_{k=1}^{K-1} \mathbb{E} \|\beta_{k,i}\|^2 + C_3 \sum_{k=1}^{K-1} \mathbb{E} \|r_{k,i}\|^2$$

We next analyze  $\beta_{k,i}$ :

$$\begin{aligned} & \sum_{i=2}^n \mathbb{E} \|\beta_{k,i}\|^2 \\ &= \alpha^2 \sum_{i=2}^n \mathbb{E} \|h_{k,i} - h_{k-1,i}\|^2 \\ &= \alpha^2 \sum_{i=2}^n \mathbb{E} \left\| \tilde{G}_k P e_i - \tilde{G}_{k-1} P e_i \right\|^2 \\ &\leq \alpha^2 \sum_{i=1}^n \mathbb{E} \left\| \tilde{G}_k P e_i - \tilde{G}_{k-1} P e_i \right\|^2 \\ &\leq \alpha^2 \mathbb{E} \left\| \tilde{G}_k P - \tilde{G}_{k-1} P \right\|_F^2 \\ &\stackrel{\text{Lemma 12}}{\leq} \alpha^2 \mathbb{E} \left\| \tilde{G}_k - \tilde{G}_{k-1} \right\|_F^2 \\ &= \alpha^2 \sum_{i=1}^n \mathbb{E} \left\| \tilde{G}_k e_i - \tilde{G}_{k-1} e_i \right\|^2 \\ &\leq 3\alpha^2 \sum_{i=1}^n \mathbb{E} \left\| \tilde{G}_k e_i - G_k e_i \right\|^2 + 3\alpha^2 \sum_{i=1}^n \mathbb{E} \left\| \tilde{G}_{k-1} e_i - G_{k-1} e_i \right\|^2 \\ &\quad + 3\alpha^2 \sum_{i=1}^n \mathbb{E} \|G_k e_i - G_{k-1} e_i\|^2 \\ &\leq 6\alpha^2 n \sigma^2 + 3\alpha^2 \sum_{i=1}^n \mathbb{E} \|G_k e_i - G_{k-1} e_i\|^2 \\ &\leq 6\alpha^2 n \sigma^2 + 3\alpha^2 L^2 \sum_{i=1}^n \mathbb{E} \|x_{k,i} - x_{k-1,i}\|^2 \\ &\leq 6\alpha^2 n \sigma^2 + 3\alpha^2 L^2 \sum_{i=1}^n \mathbb{E} \|Y_k P^\top e_i - Y_{k-1} P^\top e_i\|^2 \\ &\leq 6\alpha^2 n \sigma^2 + 3\alpha^2 L^2 \mathbb{E} \|Y_k P^\top - Y_{k-1} P^\top\|_F^2 \\ &\stackrel{\text{Lemma 12}}{\leq} 6\alpha^2 n \sigma^2 + 3\alpha^2 L^2 \mathbb{E} \|Y_k - Y_{k-1}\|_F^2 \\ &\leq 6\alpha^2 n \sigma^2 + 3\alpha^2 L^2 \sum_{i=1}^n \mathbb{E} \|y_{k,i} - y_{k-1,i}\|^2 \end{aligned}$$

And Putting it back, we have

$$\begin{aligned}
& \sum_{i=2}^n \sum_{k=1}^K \mathbb{E} \|y_{k,i}\|^2 \\
& \leq C_1 \mathbb{E} \|Y_1\|_F^2 + C_2 \sum_{i=2}^n \sum_{k=1}^{K-1} \mathbb{E} \|\beta_{k,i}\|^2 + C_3 \sum_{k=1}^{K-1} \sum_{i=2}^n \mathbb{E} \|r_{k,i}\|^2 \\
& \leq C_1 \mathbb{E} \|Y_1\|_F^2 + C_2 \sum_{k=1}^{K-1} \left( 6\alpha^2 n \sigma^2 + 3\alpha^2 L^2 \sum_{i=1}^n \mathbb{E} \|y_{k,i} - y_{k-1,i}\|^2 \right) + C_3 \sum_{k=1}^{K-1} \sum_{i=2}^n \mathbb{E} \|r_{k,i}\|^2 \\
& \stackrel{\text{Lemma 12}}{\leq} C_1 \mathbb{E} \|Y_1\|_F^2 + 6C_2 \alpha^2 n \sigma^2 K + 3C_2 \alpha^2 L^2 \sum_{k=1}^{K-1} \sum_{i=1}^n \mathbb{E} \|y_{k,i} - y_{k-1,i}\|^2 + C_3 \sum_{k=1}^{K-1} \mathbb{E} \|\Omega_k\|_F^2
\end{aligned}$$

Since

$$\begin{aligned}
& \mathbb{E} \|y_{k,1} - y_{k-1,1}\|^2 \\
& = \mathbb{E} \|X_k P e_1 - X_{k-1} P e_1\|^2 \\
& = \mathbb{E} \|X_k v_1 - X_{k-1} v_1\|^2 \\
& = \mathbb{E} \left\| X_k \frac{1}{\sqrt{n}} \mathbb{1}_n - X_{k-1} \frac{1}{\sqrt{n}} \mathbb{1}_n \right\|^2 \\
& = n \mathbb{E} \|\bar{X}_k - \bar{X}_{k-1}\|^2 \\
& = n \alpha^2 \mathbb{E} \|\widetilde{G}_k\|^2 \\
& \leq n \alpha^2 \mathbb{E} \|\widetilde{G}_k - \bar{G}_k\|^2 + n \alpha^2 \mathbb{E} \|\bar{G}_k\|^2 \\
& \leq n \alpha^2 \frac{\sigma^2}{n} + n \alpha^2 \mathbb{E} \|\bar{G}_k\|^2 \\
& = \alpha^2 \sigma^2 + n \alpha^2 \mathbb{E} \|\bar{G}_k\|^2
\end{aligned}$$

Putting it back, and we obtain

$$\begin{aligned}
& \sum_{i=2}^n \sum_{k=1}^K \mathbb{E} \|y_{k,i}\|^2 \\
& \leq C_1 \mathbb{E} \|Y_1\|_F^2 + 6C_2 \alpha^2 n \sigma^2 K + 3C_2 \alpha^4 \sigma^2 L^2 K + 3C_2 \alpha^4 n L^2 \sum_{k=1}^{K-1} \mathbb{E} \|\bar{G}_k\|^2 \\
& \quad + 3C_2 \alpha^2 L^2 \sum_{k=1}^{K-1} \sum_{i=2}^n \mathbb{E} \|y_{k,i} - y_{k-1,i}\|^2 + C_3 \sum_{k=1}^{K-1} \mathbb{E} \|\Omega_k\|_F^2 \\
& \leq C_1 \mathbb{E} \|Y_1\|_F^2 + 6C_2 \alpha^2 n \sigma^2 K + 3C_2 \alpha^4 \sigma^2 L^2 K + 3C_2 \alpha^4 n L^2 \sum_{k=1}^{K-1} \mathbb{E} \|\bar{G}_k\|^2 \\
& \quad + 6C_2 \alpha^2 L^2 \sum_{k=1}^{K-1} \sum_{i=2}^n \mathbb{E} (\|y_{k,i}\|^2 + \|y_{k-1,i}\|^2) + C_3 \sum_{k=1}^{K-1} \mathbb{E} \|\Omega_k\|_F^2 \\
& \leq C_1 \mathbb{E} \|Y_1\|_F^2 + 6C_2 \alpha^2 n \sigma^2 K + 3C_2 \alpha^4 \sigma^2 L^2 K + 3C_2 \alpha^4 n L^2 \sum_{k=1}^{K-1} \mathbb{E} \|\bar{G}_k\|^2 \\
& \quad + 12C_2 \alpha^2 L^2 \sum_{k=1}^{K-1} \sum_{i=2}^n \mathbb{E} \|y_{k,i}\|^2 + C_3 \sum_{k=1}^{K-1} \mathbb{E} \|\Omega_k\|_F^2
\end{aligned}$$

Rearrange the terms, we get

$$\begin{aligned}
& (1 - 12C_2\alpha^2L^2) \sum_{i=2}^n \sum_{k=1}^K \mathbb{E} \|y_{k,i}\|^2 \\
& \leq C_1 \mathbb{E} \|Y_1\|_F^2 + 6C_2\alpha^2n\sigma^2K + 3C_2\alpha^4\sigma^2L^2K + 3C_2\alpha^4nL^2 \sum_{k=1}^{K-1} \mathbb{E} \|\bar{G}_k\|^2 + C_3 \sum_{k=1}^{K-1} \mathbb{E} \|\Omega_k\|_F^2 \\
& \leq C_1 \mathbb{E} \|X_1\|_F^2 + 6C_2\alpha^2n\sigma^2K + 3C_2\alpha^4\sigma^2L^2K + 3C_2\alpha^4nL^2 \sum_{k=1}^{K-1} \mathbb{E} \|\bar{G}_k\|^2 + C_3 \sum_{k=1}^{K-1} \mathbb{E} \|\Omega_k\|_F^2
\end{aligned}$$

Considering

$$\begin{aligned}
\mathbb{E} \|X_1\|_F^2 &= \alpha^2 \mathbb{E} \left\| \tilde{G}_0 \right\|_F^2 \\
&= \alpha^2 \sum_{i=1}^n \mathbb{E} \left\| \tilde{G}_{0,i} - G_{0,i} + G_{0,i} - \nabla f(0) + \nabla f(0) \right\|^2 \\
&\leq 3\alpha^2 \sum_{i=1}^n \mathbb{E} \left\| \tilde{G}_{0,i} - G_{0,i} \right\|^2 + 3\alpha^2 \sum_{i=1}^n \mathbb{E} \|G_{0,i} - \nabla f(0)\|^2 + 3\alpha^2 \sum_{i=1}^n \mathbb{E} \|\nabla f(0)\|^2 \\
&\leq 3\alpha^2n\sigma^2 + 3\alpha^2n\varsigma_0^2 + 3\alpha^2n\mathbb{E} \|\nabla f(0)\|
\end{aligned}$$

We finally get

$$\begin{aligned}
& (1 - 12C_2\alpha^2L^2) \sum_{i=2}^n \sum_{k=1}^K \mathbb{E} \|y_{k,i}\|^2 \\
&= (1 - 12C_2\alpha^2L^2) \sum_{i=1}^n \sum_{k=1}^K \mathbb{E} \|\bar{X}_k - x_{k,i}\|^2 \\
&\leq 3C_1\alpha^2n\sigma^2 + 3C_1\alpha^2n\varsigma_0^2 + 3C_1\alpha^2n\mathbb{E} \|\nabla f(0)\| + 6C_2\alpha^2n\sigma^2K + 3C_2\alpha^4\sigma^2L^2K \\
&+ 3C_2\alpha^4nL^2 \sum_{k=1}^{K-1} \mathbb{E} \|\bar{G}_k\|^2 + C_3 \sum_{k=1}^{K-1} \mathbb{E} \|\Omega_k\|_F^2
\end{aligned}$$

**Lemma 11** Given  $\rho \in (-\frac{1}{3}, 0) \cup (0, 1)$ , for any two sequence  $\{a_t\}_{t=1}^\infty$ ,  $\{b_t\}_{t=1}^\infty$  and  $\{c_t\}_{t=1}^\infty$  that satisfying

$$\begin{aligned}
a_0 &= b_0 = 0, \\
a_1 &= b_1 + C_5, \\
a_{t+1} &= \rho(2a_t - a_{t-1}) + b_t - b_{t-1} + c_t, \forall t \geq 1
\end{aligned}$$

we have

$$a_{t+1} = a_1 \left( \frac{u^{t+1} - v^{t+1}}{u - v} \right) + \sum_{s=1}^t (b_s - b_{s-1} + c_s) \left( \frac{u^{t-s+1} - v^{t-s+1}}{u - v} \right), \forall t \geq 0$$

where

$$u = \rho + \sqrt{\rho^2 - \rho}, v = \rho - \sqrt{\rho^2 - \rho}$$

Moreover, if  $0 < \rho < 1$ , we have

$$a_{t+1} = a_1 \rho^{\frac{t}{2}} \frac{\sin[(t+1)\theta]}{\sin \theta} + \sum_{s=1}^t (b_s - b_{s-1} + c_s) \rho^{\frac{t-s}{2}} \frac{\sin[(t-s+1)\theta]}{\sin \theta}$$

where

$$\theta = \arccos(\sqrt{\rho})$$

**Proof** when  $t \geq 1$ , we have

$$a_{t+1} = 2\rho a_t - \rho a_{t-1} + b_t - b_{t-1} + c_t$$

since,

$$u = \rho + \sqrt{\rho^2 - \rho}, v = \rho - \sqrt{\rho^2 - \rho}$$

we obtain

$$a_{t+1} - ua_t = (a_t - ua_{t-1})v + b_t - b_{t-1} + c_t$$

Recursively we have

$$\begin{aligned} a_{t+1} - ua_t &= (a_t - ua_{t-1})v + b_t - b_{t-1} + c_t \\ &= (a_{t-1} - ua_{t-2})v^2 + (b_{t-1} - b_{t-2} + c_{t-1})v + b_t - b_{t-1} + c_t \\ &= (a_1 - ua_0)v^t + \sum_{s=1}^t (b_s - b_{s-1} + c_s)v^{t-s} \\ &= a_1v^t + \sum_{s=1}^t (b_s - b_{s-1} + c_s)v^{t-s} \end{aligned}$$

Dividing both sides by  $u^{t+1}$ , we have

$$\begin{aligned} \frac{a_{t+1}}{u^{t+1}} &= \frac{a_t}{u^t} + u^{-(t+1)} \left( a_1v^t + \sum_{s=1}^t (b_s - b_{s-1} + c_s)v^{t-s} \right) \\ &= \frac{a_{t-1}}{u^{t-1}} + u^{-t} \left( a_1v^{t-1} + \sum_{s=1}^{t-1} (b_s - b_{s-1} + c_s)v^{t-1-s} \right) + u^{-(t+1)} \left( a_1v^t + \sum_{s=1}^t (b_s - b_{s-1} + c_s)v^{t-s} \right) \\ &= \frac{a_1}{u} + \sum_{k=1}^t u^{-k-1} \left( a_1v^k + \sum_{s=1}^k (b_s - b_{s-1} + c_s)v^{k-s} \right) \end{aligned}$$

Multiplying both sides by  $u^{t+1}$

$$\begin{aligned} a_{t+1} &= a_1u^t + \sum_{k=1}^t u^{t-k} \left( a_1v^k + \sum_{s=1}^k (b_s - b_{s-1} + c_s)v^{k-s} \right) \\ &= a_1u^t \left( 1 + \sum_{k=1}^t \left( \frac{v}{u} \right)^k \right) + u^t \sum_{k=1}^t \sum_{s=1}^k (b_s - b_{s-1} + c_s)v^{-s} \left( \frac{v}{u} \right)^k \\ &= a_1u^t \sum_{k=0}^t \left( \frac{v}{u} \right)^k + u^t \sum_{s=1}^t \sum_{k=s}^t (b_s - b_{s-1} + c_s)v^{-s} \left( \frac{v}{u} \right)^k \\ &= a_1u^t \left( \frac{1 - \left( \frac{v}{u} \right)^{t+1}}{1 - \frac{v}{u}} \right) + u^t \sum_{s=1}^t (b_s - b_{s-1} + c_s)v^{-s} \left( \frac{v}{u} \right)^s \frac{1 - \left( \frac{v}{u} \right)^{t-s+1}}{1 - \frac{v}{u}} \\ &= a_1 \left( \frac{u^{t+1} - v^{t+1}}{u - v} \right) + \sum_{s=1}^t (b_s - b_{s-1} + c_s) \frac{u^{t-s+1} - v^{t-s+1}}{u - v} \end{aligned}$$

Note that when  $0 < \rho < 1$ , both  $u$  and  $v$  are complex numbers, we have

$$u = \sqrt{\rho}e^{i\theta}, v = \sqrt{\rho}e^{-i\theta}$$

where  $\theta = \arccos \sqrt{\rho}$ . And under this context, we have

$$a_{t+1} = a_1\rho^{\frac{t}{2}} \frac{\sin[(t+1)\theta]}{\sin \theta} + \sum_{s=1}^t (b_s - b_{s-1} + c_s)\rho^{\frac{t-s}{2}} \frac{\sin[(t-s+1)\theta]}{\sin \theta}$$

That completes the proof.

**Lemma 12** For any matrix  $X \in \mathbb{R}^{N \times n}$ , we have

$$\begin{aligned} \sum_{i=2}^n \|Xv_i\|^2 &\leq \sum_{i=1}^n \|Xv_i\|^2 = \|X\|_F^2 \\ \sum_{i=1}^n \|XP^\top e_i\|^2 &= \|XP^\top\|_F^2 = \|X\|_F^2 \end{aligned}$$

**Proof**

$$\sum_{i=2}^n \|X_t v_i\|^2 \leq \sum_{i=1}^n \|X_t v_i\|^2 = \|X_t P\|_F^2 = \text{Tr}(X_t P P^\top X_t^\top) = \text{Tr}(X_t X_t^\top) = \|X_t\|_F^2$$

And similarly,

$$\sum_{i=1}^n \|X P^\top e_i\|^2 = \|X P^\top\|_F^2 = \text{Tr}(X_t P^\top P X_t^\top) = \text{Tr}(X_t X_t^\top) = \|X_t\|_F^2$$

That completes the proof.

**Lemma 13** If we run Algorithm 2 for  $K$  iterations the following inequality holds:

$$\begin{aligned} &\left(1 - \frac{3C_1\alpha^2 L^2}{C_4}\right) \mathbb{E} \|\nabla f(0)\| + \left(1 - \alpha L - 3\frac{C_2}{C_4}\alpha^4 L^4\right) \frac{1}{K} \sum_{k=1}^{K-1} \mathbb{E} \|\bar{G}_k\|^2 + \frac{1}{K} \sum_{k=0}^{K-1} \mathbb{E} \|\nabla f(\bar{X}_k)\|^2 \\ &\leq \frac{2(f(0) - f^*)}{\alpha K} + \frac{\alpha L}{n} \sigma^2 + \frac{3C_1\alpha^2 L^2(\sigma^2 + \varsigma_0^2)}{C_4 K} + 6\frac{C_2}{C_4}\alpha^2 \sigma^2 L^2 + 3\frac{C_2}{nC_4}\alpha^4 \sigma^2 L^4 + \frac{C_3 L^2}{C_4} \left(\frac{12C_5 + 4}{2C_6}\right)^2 \alpha^2 B^2 \end{aligned}$$

where

$$\begin{aligned} C_1 &= \max \left\{ \frac{3}{1 - |v_n|^2}, \frac{3}{(1 - \lambda_2)^2} \right\} \\ C_2 &= \max \left\{ \frac{3\lambda_n^2}{(1 - |v_n|)^2}, \frac{3\lambda_2^2}{(1 - \sqrt{\lambda_2})^2(1 - \lambda_2)} \right\} \\ C_3 &= \max \left\{ \frac{3}{(1 - |v_n|)^2}, \frac{3}{(1 - \sqrt{\lambda_2})^2(1 - \lambda_2)} \right\} \\ C_4 &= 1 - 12C_2\alpha^2 L^2 \\ \Omega_k e_i &= \sum_{j=1}^n \left( (q_{k,j} - x_{k+\frac{1}{2},j}) - (q_{k,i} - x_{k+\frac{1}{2},i}) \right) W_{ji} \end{aligned}$$

**Proof** Since

$$\begin{aligned} \bar{X}_{k+1} &= (2X_k - X_{k-1} - \alpha\tilde{G}_k + \alpha\tilde{G}_{k-1})W \frac{\mathbb{1}_n}{n} + (Q_k - X_{k+\frac{1}{2}})(W - I) \frac{\mathbb{1}_n}{n} \\ &= 2\bar{X}_k - \bar{X}_{k-1} - \alpha\bar{\tilde{G}}_k + \alpha\bar{\tilde{G}}_{k-1} \end{aligned}$$

and we have

$$\begin{aligned} \bar{X}_{k+1} - \bar{X}_k &= \bar{X}_k - \bar{X}_{k-1} - \alpha\bar{\tilde{G}}_k + \alpha\bar{\tilde{G}}_{k-1} \\ &= \bar{X}_1 - \bar{X}_0 - \alpha \sum_{t=1}^k (\bar{\tilde{G}}_t - \bar{\tilde{G}}_{t-1}) \\ &= -\alpha\bar{\tilde{G}}_k \end{aligned}$$

As a result, we can reuse Lemma 6 from D-PSGD, thus we have

$$\frac{1 - \alpha L}{K} \sum_{k=0}^{K-1} \mathbb{E} \|\bar{G}_k\|^2 + \frac{1}{K} \sum_{k=0}^{K-1} \mathbb{E} \|\nabla f(\bar{X}_k)\|^2 \leq \frac{2(f(0) - f^*)}{\alpha K} + \frac{\alpha L}{n} \sigma^2 + \frac{L^2}{nK} \sum_{k=0}^{K-1} \sum_{i=1}^n \mathbb{E} \|\bar{X}_k - x_{k,i}\|^2$$

From Lemma 10 we obtain

$$\begin{aligned}
& \frac{1-\alpha L}{K} \sum_{k=0}^{K-1} \mathbb{E} \|\bar{G}_k\|^2 + \frac{1}{K} \sum_{k=0}^{K-1} \mathbb{E} \|\nabla f(\bar{X}_k)\|^2 \\
& \leq \frac{2(f(0) - f^*)}{\alpha K} + \frac{\alpha L}{n} \sigma^2 + \frac{3C_1 \alpha^2 L^2 (\sigma^2 + \varsigma_0^2 + \mathbb{E} \|\nabla f(0)\|)}{C_4 K} + 6 \frac{C_2}{C_4} \alpha^2 \sigma^2 L^2 + 3 \frac{C_2}{nC_4} \alpha^4 \sigma^2 L^4 \\
& + 3 \frac{C_2}{C_4} \alpha^4 L^4 \frac{1}{K} \sum_{k=1}^{K-1} \mathbb{E} \|\bar{G}_k\|^2 + \frac{C_3 L^2}{C_4 n K} \sum_{k=1}^{K-1} \mathbb{E} \|\Omega_k\|_F^2
\end{aligned}$$

Rearrange the terms, we get

$$\begin{aligned}
& \left(1 - \frac{3C_1 \alpha^2 L^2}{C_4}\right) \mathbb{E} \|\nabla f(0)\| + \left(1 - \alpha L - 3 \frac{C_2}{C_4} \alpha^4 L^4\right) \frac{1}{K} \sum_{k=1}^{K-1} \mathbb{E} \|\bar{G}_k\|^2 + \frac{1}{K} \sum_{k=0}^{K-1} \mathbb{E} \|\nabla f(\bar{X}_k)\|^2 \\
& \leq \frac{2(f(0) - f^*)}{\alpha K} + \frac{\alpha L}{n} \sigma^2 + \frac{3C_1 \alpha^2 L^2 (\sigma^2 + \varsigma_0^2)}{C_4 K} + 6 \frac{C_2}{C_4} \alpha^2 \sigma^2 L^2 + 3 \frac{C_2}{nC_4} \alpha^4 \sigma^2 L^4 + \frac{C_3 L^2}{C_4 n K} \sum_{k=1}^{K-1} \mathbb{E} \|\Omega_k\|_F^2 \\
& \stackrel{\text{Lemma 14}}{\leq} \frac{2(f(0) - f^*)}{\alpha K} + \frac{\alpha L}{n} \sigma^2 + \frac{3C_1 \alpha^2 L^2 (\sigma^2 + \varsigma_0^2)}{C_4 K} + 6 \frac{C_2}{C_4} \alpha^2 \sigma^2 L^2 + 3 \frac{C_2}{nC_4} \alpha^4 \sigma^2 L^4 + \frac{C_3 L^2}{C_4} \left(\frac{12C_5 + 4}{2C_6}\right)^2 \alpha^2 B^2
\end{aligned}$$

That completes the proof

**Lemma 14**

$$\sum_{k=0}^{K-1} \mathbb{E} \|\Omega_k\|_F^2 \leq \left(\frac{12C_5 + 4}{2C_6}\right)^2 \alpha^2 B^2 n K$$

**Proof** Similar to the case in D-PSGD, we have

$$\begin{aligned}
& \sum_{k=0}^{K-1} \mathbb{E} \|\Omega_k\|_F^2 \\
& = \sum_{k=0}^{K-1} \sum_{i=1}^n \mathbb{E} \|\Omega_k e_i\|^2 \\
& \leq \sum_{k=0}^{K-1} \sum_{i=1}^n \mathbb{E} \left\| \sum_{j=1}^n \left( (q_{k,j} - x_{k+\frac{1}{2},j}) - (q_{k,i} - x_{k+\frac{1}{2},i}) \right) W_{ji} \right\|^2 \\
& \stackrel{\text{Jensen}}{\leq} \sum_{k=0}^{K-1} \sum_{i=1}^n \sum_{j=1}^n W_{ji} \mathbb{E} \left\| \left( (q_{k,j} - x_{k+\frac{1}{2},j}) - (q_{k,i} - x_{k+\frac{1}{2},i}) \right) \right\|^2 \\
& = \sum_{k=0}^{K-1} \sum_{i=1}^n \sum_{j=1}^n W_{ji} \left( \mathbb{E} \left\| \theta \mathcal{Q} \left( \frac{x_{k+\frac{1}{2},j}}{\theta} \mod 1 \right) - \theta \mathcal{Q} \left( \frac{x_{k+\frac{1}{2},i}}{\theta} \mod 1 \right) - (x_{k+\frac{1}{2},j} - x_{k+\frac{1}{2},i}) \right\|^2 \right) \\
& \leq \sum_{k=0}^{K-1} \sum_{i=1}^n \sum_{j=1}^n W_{ji} \left( \mathbb{E} \left\| \theta \mathcal{Q} \left( \frac{x_{k+\frac{1}{2},j}}{\theta} \mod 1 \right) - \theta \mathcal{Q} \left( \frac{x_{k+\frac{1}{2},i}}{\theta} \mod 1 \right) - \theta \left( \frac{x_{k+\frac{1}{2},j} - x_{k+\frac{1}{2},i}}{\theta} \mod 1 \right) \right\|^2 \right) \\
& \leq 2 \sum_{k=0}^{K-1} \sum_{i=1}^n \sum_{j=1}^n W_{ji} \mathbb{E} \left\| \theta \mathcal{Q} \left( \frac{x_{k+\frac{1}{2},j}}{\theta} \mod 1 \right) - \theta \left( \frac{x_{k+\frac{1}{2},j}}{\theta} \mod 1 \right) \right\|^2 \\
& + 2 \sum_{k=0}^{K-1} \sum_{i=1}^n \sum_{j=1}^n W_{ji} \mathbb{E} \left\| \theta \mathcal{Q} \left( \frac{x_{k+\frac{1}{2},i}}{\theta} \mod 1 \right) - \theta \left( \frac{x_{k+\frac{1}{2},i}}{\theta} \mod 1 \right) \right\|^2 \\
& \leq 4 \sum_{k=0}^{K-1} \sum_{i=1}^n \mathbb{E} \left\| \theta \mathcal{Q} \left( \frac{x_{k+\frac{1}{2},i}}{\theta} \mod 1 \right) - \theta \left( \frac{x_{k+\frac{1}{2},i}}{\theta} \mod 1 \right) \right\|^2
\end{aligned}$$

$$\begin{aligned}
&\leq 4 \sum_{k=0}^{K-1} \sum_{i=1}^n \omega^2 \theta^2 \\
&\leq \left( \frac{12C_5 + 4}{2C_6} \right)^2 \alpha^2 B^2 n K
\end{aligned}$$

## H Moniqua on AD-PSGD (Proof to Theorem 4)

### H.1 Definition and Notation

In the original analysis of AD-PSGD, to better capture the nature of workers computing at different speed, the objective function is expressed as

$$f(x) = \sum_{i=1}^n p_i f_i(x)$$

where  $p_i$  is a parameter denoting the speed of  $i$ -th worker gradient updates. In the rest of the proof, we denote  $p = \max_i \{p_i\}$

For simplicity, we also define the following terms

$$\begin{aligned}
\nabla F(X_k) &= n [p_1 g_{k,1}, \dots, p_n g_{k,n}] \in \mathbb{R}^{d \times n} \\
\nabla \tilde{F}(X_k) &= n [p_1 \tilde{g}_{k,1}, \dots, p_n \tilde{g}_{k,n}] \in \mathbb{R}^{d \times n} \\
\tilde{G}_k &= [\dots, \tilde{g}_{k,i_k}, \dots] \\
G_k &= [\dots, g_{k,i_k}, \dots] \\
\Lambda_a^b &= \frac{\mathbb{1}_n \mathbb{1}_n^\top}{n} - \prod_{q=a}^b W_q
\end{aligned}$$

### H.2 Assumption

We makes the following assumptions:

1. **Lipschitzian Gradient:** All the function  $f_i$  have L-Lipschitzian gradients.
2. **Communication Matrix**<sup>7</sup>: The communication matrix  $W_k$  is doubly stochastic for any  $k \geq 0$  and for any  $b \geq a \geq 0$ , there exists  $t_{\text{mix}}$  such that

$$\left\| \prod_{q=a}^b W_q \left( I - \frac{\mathbb{1}_n \mathbb{1}_n^\top}{n} \right) \right\|_1 \leq 2 \cdot 2^{-\lfloor \frac{b-a+1}{t_{\text{mix}}} \rfloor}$$

3. **Bounded Variance:**

$$\begin{aligned}
\mathbb{E}_{\xi \sim \mathcal{D}_i} \left\| \nabla \tilde{f}_i(x; \xi_i) - \nabla f_i(x) \right\|^2 &\leq \sigma^2, \forall i \\
\mathbb{E}_{i \sim \mathcal{I}} \left\| \nabla f_i(x) - \nabla f(x) \right\|^2 &\leq \varsigma^2, \forall i
\end{aligned}$$

where  $\nabla \tilde{f}_i(x; \xi_i)$  denotes gradient sample on worker  $i$  computed via data sample  $\xi_i$ .

4. **Bounded Staleness:** There exists  $T$  such that  $\tau_k \leq T, \forall k$
5. **Gradient magnitude:** The norm of a sampled gradient is bounded by  $\|\tilde{g}_{k,i}\| \leq B$  for some constant  $B$ .

---

<sup>7</sup>Please refer to Section E for more details

### H.3 Algorithm

---

**Algorithm 3** Asynchronous Algorithm on a single Worker

---

**Input:** initial point  $x_{0,i} = x_0$ , step size  $\alpha$ , number of iterations  $K$ , quantization function  $\mathcal{Q}$ , initial random seed

- 1: **for**  $k = 0, 1, 2, \dots, K - 1$  **do**
- 2:   worker  $i_k$  is updating the gradient while during this iteration the global communication behaviour is written in the form of  $W_k$ .
- 3:   Compute a local stochastic gradient:  $\tilde{g}_{k-\tau_k, i_k}$
- 4:   Randomly select one of the neighbors  $j_k$  and average local weights with remote weights while subtracting the biased term:

$$x_{k+\frac{1}{2}, i_k} \leftarrow x_{k, i_k} + \frac{1}{2}q_{k, j_k} - \frac{1}{2}b_{k, i_k}$$

- 5:   Update the local weight with local gradient:  $x_{k+1, i_k} \leftarrow x_{k, i_k} - \alpha \tilde{g}_{k-\tau_k, i_k}$
- 6: **end for**

**Output:**  $\bar{X}_K = \frac{1}{n} \sum_{i=1}^n x_{K, i}$

---

Note that the gradient updated to the local model has a delay, or staleness  $\tau_k$  since between the time gradient is computed and updated, the model can be averaged by other local models. This setting is aligned with AD-PSGD.

### H.4 Theorems

We highlight all the theorems there:

**Theorem 3** If we apply quantizer  $\mathcal{Q}_\omega$  on the communication, by setting hyperparameters<sup>8</sup> to

$$\theta = 16t_{\text{mix}}\alpha B, \quad \omega = \frac{1}{32t_{\text{mix}}}, \quad \text{and} \quad \alpha = \frac{n}{2L + \sqrt{K(\sigma^2 + 6\zeta^2)}},$$

applying Moniqua on AD-PSGD has the following asymptotic convergence rate:

$$\frac{1}{K} \sum_{k=0}^{K-1} \mathbb{E} \|\nabla f(\bar{X}_k)\|^2 \lesssim \frac{1}{K} + \frac{\sqrt{\sigma^2 + 6\zeta^2}}{\sqrt{K}} + \frac{(\sigma^2 + 6\zeta^2)t_{\text{mix}}^2 n^2}{(\sigma^2 + 6\zeta^2)K + 1} + \frac{n^2 t_{\text{mix}}^2 B^2}{(\sigma^2 + 6\zeta^2)K + 1}$$

**Corollary 4** If we use a linear quantizer with quantization step  $\delta$  as  $\mathcal{Q}_\omega$  in Theorem 3, the number of bits  $\mathcal{B}$  required per dimension per iteration is upper bounded by  $\mathcal{B} \leq \log(32t_{\text{mix}}\sqrt{d})$ .

### H.5 Proof

We start from

$$\begin{aligned} & \frac{1}{K} \sum_{k=0}^{K-1} \mathbb{E} \|\nabla f(\bar{X}_k)\|^2 + \left(1 - \frac{2\alpha L}{n}\right) \frac{1}{K} \sum_{k=0}^{K-1} \mathbb{E} \|\nabla \bar{F}(X_{k-\tau_k})\|^2 \\ & \stackrel{\text{Lemma 18}}{\leq} \frac{2n(f(0) - f^*)}{\alpha K} + \frac{(\sigma^2 + 6\zeta^2)\alpha L}{n} + \left(2L^2 + \frac{12\alpha L^3}{n}\right) \frac{1}{K} \sum_{k=0}^{K-1} \sum_{i=1}^n p_i \mathbb{E} \left\| X_{k-\tau_k} \left( \frac{\mathbb{1}_n}{n} - e_i \right) \right\|^2 \\ & \quad + \frac{2L^2}{K} \sum_{k=0}^{K-1} \mathbb{E} \left\| \frac{(X_k - X_{k-\tau_k}) \mathbb{1}_n}{n} \right\|^2 \\ & \stackrel{\text{Lemma 19}}{\leq} \frac{2n(f(0) - f^*)}{\alpha K} + \frac{(\sigma^2 + 6\zeta^2)\alpha L}{n} + \frac{2\alpha^2 T^2 (\sigma^2 + 6\zeta^2) L^2}{n^2} + \frac{4\alpha^2 T^2 L^2}{n^2 K} \sum_{k=0}^{K-1} \mathbb{E} \left\| \sum_{i=1}^n p_i g_{k-\tau_k, i} \right\|^2 \end{aligned}$$

---

<sup>8</sup>Please refer to Section E for details about definition of  $t_{\text{mix}}$

$$\begin{aligned}
& + \left( 2L^2 + \frac{12\alpha L^3}{n} + \frac{24L^4\alpha^2 T^2}{n^2} \right) \frac{1}{K} \sum_{k=0}^{K-1} \sum_{i=1}^n p_i \mathbb{E} \left\| X_{k-\tau_k} \left( \frac{\mathbb{1}_n}{n} - e_i \right) \right\|^2 \\
& \stackrel{\text{Lemma 17}}{\leq} \frac{2n(f(0) - f^*)}{\alpha K} + \frac{(\sigma^2 + 6\varsigma^2)\alpha L}{n} + \frac{2\alpha^2 T^2(\sigma^2 + 6\varsigma^2)L^2}{n^2} + \frac{4\alpha^2 T^2 L^2}{n^2 K} \sum_{k=0}^{K-1} \mathbb{E} \left\| \sum_{i=1}^n p_i g_{k-\tau_k, i} \right\|^2 \\
& + \frac{128\alpha^2 t_{\text{mix}}^2 L^2}{A_1} \left( (\sigma^2 + 6\varsigma^2)p + \frac{2p}{K} \sum_{k=0}^{K-1} \mathbb{E} \left\| \sum_{i=1}^n p_i g_{k-\tau_k, i} \right\|^2 + B^2 \right)
\end{aligned}$$

where  $A_1 = 1 - 192p\alpha^2 t_{\text{mix}}^2 L^2$  as defined in Lemma 17.

Rearrange the terms, we get

$$\begin{aligned}
\frac{1}{K} \sum_{k=0}^{K-1} \mathbb{E} \left\| \nabla f(\bar{X}_k) \right\|^2 & \leq \frac{2n(f(0) - f^*)}{\alpha K} + \frac{(\sigma^2 + 6\varsigma^2)\alpha L}{n} + \frac{2\alpha^2 T^2(\sigma^2 + 6\varsigma^2)L^2}{n^2} \\
& + \frac{128p\alpha^2 t_{\text{mix}}^2 L^2}{A_1} (\sigma^2 + 6\varsigma^2) + \frac{128\alpha^2 t_{\text{mix}}^2 L^2}{A_1} B^2
\end{aligned}$$

By setting  $\alpha = \frac{n}{2L + \sqrt{K(\sigma^2 + 6\varsigma^2)}}$

$$\begin{aligned}
\frac{1}{K} \sum_{k=0}^{K-1} \mathbb{E} \left\| \nabla f(\bar{X}_k) \right\|^2 & \lesssim \frac{1}{K} + \frac{\sqrt{\sigma^2 + 6\varsigma^2}}{\sqrt{K}} + \frac{pt_{\text{mix}}^2(\sigma^2 + 6\varsigma^2)n^2}{(\sigma^2 + 6\varsigma^2)K + 4L^2} + \frac{n^2 t_{\text{mix}}^2 B^2}{(\sigma^2 + 6\varsigma^2)K + 4L^2} \\
& \lesssim \frac{1}{K} + \frac{\sqrt{\sigma^2 + 6\varsigma^2}}{\sqrt{K}} + \frac{(\sigma^2 + 6\varsigma^2)t_{\text{mix}}^2 n^2}{(\sigma^2 + 6\varsigma^2)K + 1} + \frac{n^2 t_{\text{mix}}^2 B^2}{(\sigma^2 + 6\varsigma^2)K + 1}
\end{aligned}$$

## H.6 Proof to Corollary

### Proof to Corollary 4

**Proof** The number of bits used in the communication per iteration per dimension can be written as  $\log\left(\frac{1}{\delta}\right)$ , note that for linear quantizer,  $\omega = \delta\sqrt{d}$ , so we have number of bits is upper bounded by  $\log\left(\frac{1}{\delta}\right) = \log\left(\frac{\sqrt{d}}{\omega}\right) = \log\left(32t_{\text{mix}}\sqrt{d}\right)$

## H.7 Lemma for Moniqua on AD-PSGD

### Lemma 15

$$\mathbb{E} \left\| \tilde{G}_{k-\tau_k} \frac{\mathbb{1}_n}{n} \right\|^2 \leq \frac{\sigma^2}{n^2} + \frac{1}{n^2} \sum_{i=1}^n p_i \mathbb{E} \|g_{k-\tau_k, i}\|^2, \forall k \geq 0.$$

**Proof**

$$\begin{aligned}
\mathbb{E} \left\| \tilde{G}_{k-\tau_k} \frac{\mathbb{1}_n}{n} \right\|^2 & \leq \sum_{i=1}^n p_i \mathbb{E} \left\| \frac{\tilde{g}_{k-\tau_k, i}}{n} \right\|^2 \\
& = \sum_{i=1}^n p_i \mathbb{E} \left\| \frac{\tilde{g}_{k-\tau_k, i} - g_{k-\tau_k, i}}{n} \right\|^2 + \sum_{i=1}^n p_i \mathbb{E} \left\| \frac{g_{k-\tau_k, i}}{n} \right\|^2 \\
& \leq \frac{\sigma^2}{n^2} + \frac{1}{n^2} \sum_{i=1}^n p_i \mathbb{E} \|g_{k-\tau_k, i}\|^2
\end{aligned}$$

### Lemma 16

$$\sum_{i=1}^n p_i \mathbb{E} \|g_{k-\tau_k, i}\|^2 \leq 12L^2 \sum_{i=1}^n p_i \mathbb{E} \left\| X_{k-\tau_k} \left( \frac{\mathbb{1}_n}{n} - e_i \right) \right\|^2 + 6\varsigma^2 + 2\mathbb{E} \left\| \sum_{i=1}^n p_i g_{k-\tau_k, i} \right\|^2, \forall k \geq 0.$$

**Proof**

$$\begin{aligned}
\sum_{i=1}^n p_i \mathbb{E} \|g_{k-\tau_k, i}\|^2 &= \sum_{i=1}^n p_i \mathbb{E} \left\| g_{k-\tau_k, i} - \sum_{i=1}^n p_i g_{k-\tau_k, i} + \sum_{i=1}^n p_i g_{k-\tau_k, i} \right\|^2 \\
&\leq 2 \sum_{i=1}^n p_i \mathbb{E} \left\| g_{k-\tau_k, i} - \sum_{i=1}^n p_i g_{k-\tau_k, i} \right\|^2 + 2 \sum_{i=1}^n p_i \mathbb{E} \left\| \sum_{i=1}^n p_i g_{k-\tau_k, i} \right\|^2 \\
&= 2 \sum_{i=1}^n p_i \mathbb{E} \left\| g_{k-\tau_k, i} - \sum_{i=1}^n p_i g_{k-\tau_k, i} \right\|^2 + 2 \mathbb{E} \left\| \sum_{i=1}^n p_i g_{k-\tau_k, i} \right\|^2
\end{aligned}$$

*And*

$$\begin{aligned}
&\sum_{i=1}^n p_i \mathbb{E} \left\| g_{k-\tau_k, i} - \sum_{i=1}^n p_i g_{k-\tau_k, i} \right\|^2 \\
&\leq 3 \sum_{i=1}^n p_i \mathbb{E} \|g_{k-\tau_k, i} - \nabla f_i(\bar{X}_{k-\tau_k})\|^2 + 3 \sum_{i=1}^n p_i \mathbb{E} \left\| \nabla f_i(\bar{X}_{k-\tau_k}) - \sum_{j=1}^n p_j \nabla f_j(\bar{X}_{k-\tau_k}) \right\|^2 \\
&+ 3 \sum_{i=1}^n p_i \mathbb{E} \left\| \sum_{i=1}^n p_i g_{k-\tau_k, i} - \sum_{j=1}^n p_j \nabla f_j(\bar{X}_{k-\tau_k}) \right\|^2 \\
&\leq 3L^2 \sum_{i=1}^n p_i \mathbb{E} \|x_{k-\tau_k, i} - \bar{X}_{k-\tau_k}\|^2 + 3 \sum_{i=1}^n p_i \mathbb{E} \left\| \nabla f_i(\bar{X}_{k-\tau_k}) - \sum_{j=1}^n p_j \nabla f_j(\bar{X}_{k-\tau_k}) \right\|^2 \\
&+ 3 \mathbb{E} \left\| \sum_{i=1}^n p_i g_{k-\tau_k, i} - \sum_{j=1}^n p_j \nabla f_j(\bar{X}_{k-\tau_k}) \right\|^2 \\
&\leq 3L^2 \sum_{i=1}^n p_i \mathbb{E} \left\| X_{k-\tau_k} \left( \frac{\mathbb{1}_n}{n} - e_i \right) \right\|^2 + 3 \sum_{i=1}^n p_i \mathbb{E} \left\| \nabla f_i(\bar{X}_{k-\tau_k}) - \nabla f(\bar{X}_{k-\tau_k}) \right\|^2 + 3 \sum_{j=1}^n p_j \mathbb{E} \|g_{k-\tau_k, j} - \nabla f_j(\bar{X}_{k-\tau_k})\|^2 \\
&\leq 6L^2 \sum_{i=1}^n p_i \mathbb{E} \left\| X_{k-\tau_k} \left( \frac{\mathbb{1}_n}{n} - e_i \right) \right\|^2 + 3\varsigma^2
\end{aligned}$$

*That completes the proof.*

**Lemma 17** Let  $A_1 = 1 - 192p\alpha^2 t_{\text{mix}}^2 L^2$ ,

$$\sum_{k=0}^{K-1} \sum_{i=1}^n p_i \mathbb{E} \left\| X_{k-\tau_k} \left( \frac{\mathbb{1}_n}{n} - e_i \right) \right\|^2 \leq \frac{32\alpha^2 t_{\text{mix}}^2}{A_1} \left( (\sigma^2 + 6\varsigma^2)pK + 2p \sum_{k=0}^{K-1} \mathbb{E} \left\| \sum_{i=1}^n p_i g_{k-\tau_k, i} \right\|^2 + B^2 K \right)$$

**Proof**

$$\begin{aligned}
&\sum_{i=1}^n p_i \mathbb{E} \left\| X_k \left( \frac{\mathbb{1}_n}{n} - e_i \right) \right\|^2 \\
&= \sum_{i=1}^n p_i \mathbb{E} \left\| \left( X_{k-1} W_{k-1} - \alpha \tilde{G}_{k-1-\tau_{k-1}} + \Omega_{k-1} \right) \left( \frac{\mathbb{1}_n}{n} - e_i \right) \right\|^2 \\
&\stackrel{X_0=0}{=} \sum_{i=1}^n p_i \mathbb{E} \left\| \sum_{t=0}^{k-1} \left( -\alpha \tilde{G}_{t-\tau_t} + \Omega_t \right) \Lambda_{t+1}^{k-1} e_i \right\|^2 \\
&\leq 2 \sum_{i=1}^n p_i \mathbb{E} \left\| \sum_{t=0}^{k-1} \alpha \tilde{G}_{t-\tau_t} \Lambda_{t+1}^{k-1} e_i \right\|^2 + 2 \sum_{i=1}^n p_i \mathbb{E} \left\| \sum_{t=0}^{k-1} \Omega_t \Lambda_{t+1}^{k-1} e_i \right\|^2
\end{aligned}$$

Now for the first term, we have

$$\begin{aligned}
2 \sum_{i=1}^n p_i \mathbb{E} \left\| \sum_{t=0}^{k-1} \alpha \tilde{G}_{t-\tau_t} \Lambda_{t+1}^{k-1} e_i \right\|^2 &\leq 2p\alpha^2 \mathbb{E} \left\| \sum_{t=0}^{k-1} \tilde{G}_{t-\tau_t} \Lambda_{t+1}^{k-1} \right\|_F^2 \\
&\leq 2p\alpha^2 \mathbb{E} \left( \sum_{t=0}^{k-1} \left\| \tilde{G}_{t-\tau_t} \right\|_F \left\| \Lambda_{t+1}^{k-1} \right\| \right)^2 \\
&\leq 2p\alpha^2 \mathbb{E} \left( \sum_{t=0}^{k-1} \left\| \tilde{G}_{t-\tau_t} \right\|_F \left\| \Lambda_{t+1}^{k-1} \right\|_1 \right)^2 \\
&\leq 8p\alpha^2 \mathbb{E} \left( \sum_{t=0}^{k-1} \left\| \tilde{G}_{t-\tau_t} \right\|_F 2^{-\lfloor \frac{k-t-1}{t_{\text{mix}}} \rfloor} \right)^2
\end{aligned}$$

Now we replace  $k$  with  $k - \tau_k$ , that is

$$\begin{aligned}
&\sum_{i=1}^n p_i \mathbb{E} \left\| X_{k-\tau_k} \left( \frac{\mathbb{1}_n}{n} - e_i \right) \right\|^2 \\
&\leq 8p\alpha^2 \mathbb{E} \left( \sum_{t=0}^{k-\tau_k-1} \left\| \tilde{G}_{t-\tau_t} \right\|_F 2^{-\lfloor \frac{k-\tau_k-t-1}{t_{\text{mix}}} \rfloor} \right)^2 + 2 \sum_{i=1}^n p_i \mathbb{E} \left\| \sum_{t=0}^{k-\tau_k-1} \Omega_t \Lambda_{t+1}^{k-\tau_k-1} e_i \right\|^2
\end{aligned}$$

Summing from  $k = 0$  to  $K - 1$  on both sides, we obtain

$$\begin{aligned}
&\sum_{k=0}^{K-1} \sum_{i=1}^n p_i \mathbb{E} \left\| X_{k-\tau_k} \left( \frac{\mathbb{1}_n}{n} - e_i \right) \right\|^2 \\
&\leq 8p\alpha^2 \sum_{k=0}^{K-1} \mathbb{E} \left( \sum_{t=0}^{k-\tau_k-1} \left\| \tilde{G}_{t-\tau_t} \right\|_F 2^{-\lfloor \frac{k-\tau_k-t-1}{t_{\text{mix}}} \rfloor} \right)^2 + 2 \sum_{i=1}^n p_i \sum_{k=0}^{K-1} \mathbb{E} \left\| \sum_{t=0}^{k-\tau_k-1} \Omega_t \Lambda_{t+1}^{k-\tau_k-1} e_i \right\|^2 \\
&\leq 8p\alpha^2 \sum_{k=0}^{K-1} \mathbb{E} \left( \sum_{t=0}^{k-\tau_k-1} \left\| \tilde{G}_{t-\tau_t} \right\|_F 2^{-\lfloor \frac{k-\tau_k-t-1}{t_{\text{mix}}} \rfloor} \right)^2 + 2 \sum_{i=1}^n p_i \sum_{k=0}^{K-1} \mathbb{E} \left( \sum_{t=0}^{k-\tau_k-1} \left\| \Omega_t \right\|_{2 \leftarrow 1} \left\| \Lambda_{t+1}^{k-\tau_k-1} \right\|_1 \left\| e_i \right\|_1 \right)^2 \\
&\leq 8p\alpha^2 \sum_{k=0}^{K-1} \mathbb{E} \left( \sum_{t=0}^{k-\tau_k-1} \left\| \tilde{G}_{t-\tau_t} \right\|_F 2^{-\lfloor \frac{k-\tau_k-t-1}{t_{\text{mix}}} \rfloor} \right)^2 + 8 \sum_{i=1}^n p_i \sum_{k=0}^{K-1} \mathbb{E} \left( \sum_{t=0}^{k-\tau_k-1} \left\| \Omega_t \right\|_{2 \leftarrow 1} 2^{-\lfloor \frac{k-\tau_k-t-1}{t_{\text{mix}}} \rfloor} \right)^2 \\
&\stackrel{\text{Lemma 20}}{\leq} 8p\alpha^2 \sum_{k=0}^{K-1} \mathbb{E} \left( \sum_{t=0}^{k-\tau_k-1} \left\| \tilde{G}_{t-\tau_t} \right\|_F 2^{-\lfloor \frac{k-\tau_k-t-1}{t_{\text{mix}}} \rfloor} \right)^2 + 32t_{\text{mix}}^2 \sum_{i=1}^n p_i \sum_{k=0}^{K-1} \mathbb{E} \left\| \Omega_k \right\|_{2 \leftarrow 1}^2 \\
&\leq 8p\alpha^2 \sum_{k=0}^{K-1} \mathbb{E} \left( \sum_{t=0}^{k-\tau_k-1} \left\| \tilde{G}_{t-\tau_t} \right\|_F 2^{-\lfloor \frac{k-\tau_k-t-1}{t_{\text{mix}}} \rfloor} \right)^2 + 128\omega^2 \theta^2 t_{\text{mix}}^2 K \\
&\stackrel{\text{Lemma 20}}{\leq} 32p\alpha^2 t_{\text{mix}}^2 \sum_{k=0}^{K-1} \mathbb{E} \left\| \tilde{G}_{k-\tau_k} \right\|_F^2 + 128\omega^2 \theta^2 t_{\text{mix}}^2 K
\end{aligned}$$

Note that for the first term, we have

$$\begin{aligned}
&\sum_{k=0}^{K-1} \mathbb{E} \left\| \tilde{G}_{k-\tau_k} \right\|_F^2 \\
&= \sum_{k=0}^{K-1} \mathbb{E} \left\| \tilde{g}_{k-\tau_k, i_k} \right\|^2
\end{aligned}$$

$$\begin{aligned}
&= \sum_{k=0}^{K-1} \mathbb{E} \|\tilde{g}_{k-\tau_k, i_k} - g_{k-\tau_k, i_k}\|^2 + \sum_{k=0}^{K-1} \mathbb{E} \|g_{k-\tau_k, i_k}\|^2 \\
&\leq \sigma^2 K + \sum_{k=0}^{K-1} \sum_{i=1}^n p_i \mathbb{E} \|g_{t-\tau_t, i}\|^2 \\
&\leq (\sigma^2 + 6\varsigma^2)K + 12L^2 \sum_{k=0}^{K-1} \sum_{i=1}^n p_i \mathbb{E} \left\| X_{k-\tau_k} \left( \frac{\mathbb{1}_n}{n} - e_i \right) \right\|^2 + 2 \sum_{k=0}^{K-1} \mathbb{E} \left\| \sum_{i=1}^n p_i g_{k-\tau_k, i} \right\|^2
\end{aligned}$$

Putting these two terms back, we obtain

$$\begin{aligned}
&\sum_{k=0}^{K-1} \sum_{i=1}^n p_i \mathbb{E} \left\| X_{k-\tau_k} \left( \frac{\mathbb{1}_n}{n} - e_i \right) \right\|^2 \\
&\leq 32p\alpha^2 t_{\text{mix}}^2 \left( (\sigma^2 + 6\varsigma^2)K + 12L^2 \sum_{k=0}^{K-1} \sum_{i=1}^n p_i \mathbb{E} \left\| X_{k-\tau_k} \left( \frac{\mathbb{1}_n}{n} - e_i \right) \right\|^2 + 2 \sum_{k=0}^{K-1} \mathbb{E} \left\| \sum_{i=1}^n p_i g_{k-\tau_k, i} \right\|^2 \right) \\
&+ 128\omega^2 \theta^2 t_{\text{mix}}^2 K
\end{aligned}$$

Rearrange the terms, we obtain

$$\begin{aligned}
&(1 - 192p\alpha^2 t_{\text{mix}}^2 L^2) \sum_{k=0}^{K-1} \sum_{i=1}^n p_i \mathbb{E} \left\| X_{k-\tau_k} \left( \frac{\mathbb{1}_n}{n} - e_i \right) \right\|^2 \\
&\leq 32p\alpha^2 t_{\text{mix}}^2 \left( (\sigma^2 + 6\varsigma^2)K + 2 \sum_{k=0}^{K-1} \mathbb{E} \left\| \sum_{i=1}^n p_i g_{k-\tau_k, i} \right\|^2 \right) + 128\omega^2 \theta^2 t_{\text{mix}}^2 K \\
&\stackrel{\text{Lemma 21}}{\leq} 32\alpha^2 t_{\text{mix}}^2 \left( (\sigma^2 + 6\varsigma^2)pK + 2p \sum_{k=0}^{K-1} \mathbb{E} \left\| \sum_{i=1}^n p_i g_{k-\tau_k, i} \right\|^2 + B^2 K \right)
\end{aligned}$$

Let  $A_1 = 1 - 192p\alpha^2 t_{\text{mix}}^2 L^2$ , we obtain

$$\sum_{k=0}^{K-1} \sum_{i=1}^n p_i \mathbb{E} \left\| X_{k-\tau_k} \left( \frac{\mathbb{1}_n}{n} - e_i \right) \right\|^2 \leq \frac{32\alpha^2 t_{\text{mix}}^2}{A_1} \left( (\sigma^2 + 6\varsigma^2)pK + 2p \sum_{k=0}^{K-1} \mathbb{E} \left\| \sum_{i=1}^n p_i g_{k-\tau_k, i} \right\|^2 + B^2 K \right)$$

**Lemma 18**

$$\begin{aligned}
&\frac{1}{K} \sum_{k=0}^{K-1} \mathbb{E} \|\nabla f(\bar{X}_k)\|^2 + \left(1 - \frac{2\alpha L}{n}\right) \frac{1}{K} \sum_{k=0}^{K-1} \mathbb{E} \|\nabla \bar{F}(X_{k-\tau_k})\|^2 \\
&\leq \frac{2n(f(0) - f^*)}{\alpha K} + \frac{2L^2}{K} \sum_{k=0}^{K-1} \mathbb{E} \left\| \frac{(X_k - X_{k-\tau_k})\mathbb{1}_n}{n} \right\|^2 + \left(2L^2 + \frac{12\alpha L^3}{n}\right) \frac{1}{K} \sum_{k=0}^{K-1} \sum_{i=1}^n p_i \mathbb{E} \left\| X_{k-\tau_k} \left( \frac{\mathbb{1}_n}{n} - e_i \right) \right\|^2 \\
&+ \frac{(\sigma^2 + 6\varsigma^2)\alpha L}{n}
\end{aligned}$$

**Proof** We start from  $f(\bar{X}_{k+1})$  Since

$$\bar{X}_{k+1} = X_k W_k \frac{\mathbb{1}_n}{n} + (Q_k - X_k)(W_k - I) \frac{\mathbb{1}_n}{n} - \alpha \bar{\bar{G}}_{k-\tau_k} = \bar{X}_k - \alpha \bar{\bar{G}}_{k-\tau_k}$$

Then from Taylor Expansion, we have

$$\begin{aligned}
&\mathbb{E} f(\bar{X}_{k+1}) \\
&= \mathbb{E} f\left(\bar{X}_k - \alpha \bar{\bar{G}}_{k-\tau_k}\right) \\
&\leq \mathbb{E} f(\bar{X}_k) - \alpha \mathbb{E} \langle \nabla f(\bar{X}_k), \bar{\bar{G}}_{k-\tau_k} \rangle + \frac{\alpha^2 L}{2} \mathbb{E} \left\| \bar{\bar{G}}_{k-\tau_k} \right\|^2
\end{aligned}$$

$$\begin{aligned}
&= \mathbb{E}f(\bar{X}_k) - \alpha \mathbb{E} \langle \nabla f(\bar{X}_k), \bar{G}_{k-\tau_k} \rangle - \alpha \mathbb{E} \langle \nabla f(\bar{X}_k), \bar{\tilde{G}}_{k-\tau_k} - \bar{G}_{k-\tau_k} \rangle + \frac{\alpha^2 L}{2} \mathbb{E} \left\| \bar{\tilde{G}}_{k-\tau_k} \right\|^2 \\
&= \mathbb{E}f(\bar{X}_k) - \frac{\alpha}{n} \mathbb{E} \langle \nabla f(\bar{X}_k), \nabla \bar{F}(X_{k-\tau_k}) \rangle + \frac{\alpha^2 L}{2} \mathbb{E} \left\| \frac{\tilde{g}_{k-\tau_k, i_k}}{n} \right\|^2 \\
&\leq \mathbb{E}f(\bar{X}_k) - \frac{\alpha}{n} \mathbb{E} \langle \nabla f(\bar{X}_k), \nabla \bar{F}(X_{k-\tau_k}) \rangle + \frac{\alpha^2 L}{2} \sum_{i=1}^n p_i \mathbb{E} \left\| \frac{\tilde{g}_{k-\tau_k, i_k} - g_{k-\tau_k, i_k}}{n} \right\|^2 + \frac{\alpha^2 L}{2} \sum_{i=1}^n p_i \mathbb{E} \left\| \frac{g_{k-\tau_k, i}}{n} \right\|^2 \\
&\leq \mathbb{E}f(\bar{X}_k) - \frac{\alpha}{n} \mathbb{E} \langle \nabla f(\bar{X}_k), \nabla \bar{F}(X_{k-\tau_k}) \rangle + \frac{\alpha^2 L \sigma^2}{2n^2} + \frac{\alpha^2 L}{2n^2} \sum_{i=1}^n p_i \mathbb{E} \|g_{k-\tau_k, i}\|^2 \\
&= \mathbb{E}f(\bar{X}_k) + \frac{\alpha}{2n} \mathbb{E} \left\| \nabla f(\bar{X}_k) - \nabla \bar{F}(X_{k-\tau_k}) \right\|^2 - \frac{\alpha}{2n} \mathbb{E} \left\| \nabla f(\bar{X}_k) \right\|^2 - \frac{\alpha}{2n} \mathbb{E} \left\| \nabla \bar{F}(X_{k-\tau_k}) \right\|^2 \\
&\quad + \frac{\alpha^2 L \sigma^2}{2n^2} + \frac{\alpha^2 L}{2n^2} \sum_{i=1}^n p_i \mathbb{E} \|g_{k-\tau_k, i}\|^2
\end{aligned}$$

Rearrange these terms, we can get

$$\begin{aligned}
&\frac{\alpha}{2n} \mathbb{E} \left\| \nabla f(\bar{X}_k) \right\|^2 + \frac{\alpha}{2n} \mathbb{E} \left\| \nabla \bar{F}(X_{k-\tau_k}) \right\|^2 \\
&\leq \mathbb{E}f(\bar{X}_k) - \mathbb{E}f(\bar{X}_{k+1}) + \frac{\alpha}{2n} \mathbb{E} \left\| \nabla f(\bar{X}_k) - \nabla \bar{F}(X_{k-\tau_k}) \right\|^2 + \frac{\alpha^2 L \sigma^2}{2n^2} + \frac{\alpha^2 L}{2n^2} \sum_{i=1}^n p_i \mathbb{E} \|g_{k-\tau_k, i}\|^2
\end{aligned}$$

Summing over  $k = 0$  to  $K - 1$  on both sides, we can get

$$\begin{aligned}
&\frac{1}{K} \sum_{k=0}^{K-1} \mathbb{E} \left\| \nabla f(\bar{X}_k) \right\|^2 + \frac{1}{K} \sum_{k=0}^{K-1} \mathbb{E} \left\| \nabla \bar{F}(X_{k-\tau_k}) \right\|^2 \\
&\leq \frac{2n(f(0) - f^*)}{\alpha K} + \frac{1}{K} \sum_{k=0}^{K-1} \mathbb{E} \left\| \nabla f(\bar{X}_k) - \nabla \bar{F}(X_{k-\tau_k}) \right\|^2 + \frac{\alpha L \sigma^2}{n} + \frac{\alpha L}{nK} \sum_{k=0}^{K-1} \sum_{i=1}^n p_i \mathbb{E} \|g_{k-\tau_k, i}\|^2
\end{aligned}$$

For  $\sum_{k=0}^{K-1} \mathbb{E} \left\| \nabla f(\bar{X}_k) - \nabla \bar{F}(X_{k-\tau_k}) \right\|^2$ , we have

$$\begin{aligned}
&\sum_{k=0}^{K-1} \mathbb{E} \left\| \nabla f(\bar{X}_k) - \nabla \bar{F}(X_{k-\tau_k}) \right\|^2 \\
&\leq 2 \sum_{k=0}^{K-1} \mathbb{E} \left\| \nabla f(\bar{X}_k) - \nabla f(\bar{X}_{k-\tau_k}) \right\|^2 + 2 \sum_{k=0}^{K-1} \mathbb{E} \left\| \nabla f(\bar{X}_{k-\tau_k}) - \nabla \bar{F}(X_{k-\tau_k}) \right\|^2 \\
&= 2 \sum_{k=0}^{K-1} \mathbb{E} \left\| \nabla f(\bar{X}_k) - \nabla f(\bar{X}_{k-\tau_k}) \right\|^2 + 2 \sum_{k=0}^{K-1} \mathbb{E} \left\| \sum_{i=1}^n p_i (\nabla f_i(\bar{X}_{k-\tau_k}) - g_{k-\tau_k, i}) \right\|^2 \\
&\leq 2 \sum_{k=0}^{K-1} \mathbb{E} \left\| \nabla f(\bar{X}_k) - \nabla f(\bar{X}_{k-\tau_k}) \right\|^2 + 2 \sum_{k=0}^{K-1} \mathbb{E} \sum_{i=1}^n p_i \left\| \nabla f_i(\bar{X}_{k-\tau_k}) - g_{k-\tau_k, i} \right\|^2 \\
&\leq 2L^2 \sum_{k=0}^{K-1} \mathbb{E} \left\| \frac{(X_k - X_{k-\tau_k}) \mathbb{1}_n}{n} \right\|^2 + 2L^2 \sum_{k=0}^{K-1} \sum_{i=1}^n p_i \mathbb{E} \left\| X_{k-\tau_k} \left( \frac{\mathbb{1}_n}{n} - e_i \right) \right\|^2
\end{aligned}$$

Putting it back, we have

$$\begin{aligned}
&\frac{1}{K} \sum_{k=0}^{K-1} \mathbb{E} \left\| \nabla f(\bar{X}_k) \right\|^2 + \frac{1}{K} \sum_{k=0}^{K-1} \mathbb{E} \left\| \nabla \bar{F}(X_{k-\tau_k}) \right\|^2 \\
&\leq \frac{2n(f(0) - f^*)}{\alpha K} + \frac{2L^2}{K} \sum_{k=0}^{K-1} \mathbb{E} \left\| \frac{(X_k - X_{k-\tau_k}) \mathbb{1}_n}{n} \right\|^2 + \frac{2L^2}{K} \sum_{k=0}^{K-1} \sum_{i=1}^n p_i \mathbb{E} \left\| X_{k-\tau_k} \left( \frac{\mathbb{1}_n}{n} - e_i \right) \right\|^2
\end{aligned}$$

$$\begin{aligned}
& + \frac{\alpha L \sigma^2}{n} + \frac{\alpha L}{nK} \sum_{k=0}^{K-1} \sum_{i=1}^n p_i \mathbb{E} \|g_{k-\tau_k, i}\|^2 \\
& \stackrel{\text{Lemma 16}}{\leq} \frac{2n(f(0) - f^*)}{\alpha K} + \frac{2L^2}{K} \sum_{k=0}^{K-1} \mathbb{E} \left\| \frac{(X_k - X_{k-\tau_k}) \mathbb{1}_n}{n} \right\|^2 + \frac{2L^2}{K} \sum_{k=0}^{K-1} \sum_{i=1}^n p_i \mathbb{E} \left\| X_{k-\tau_k} \left( \frac{\mathbb{1}_n}{n} - e_i \right) \right\|^2 \\
& + \frac{\alpha L \sigma^2}{n} + \frac{\alpha L}{nK} \sum_{k=0}^{K-1} \left( 12L^2 \sum_{i=1}^n p_i \mathbb{E} \left\| X_{k-\tau_k} \left( \frac{\mathbb{1}_n}{n} - e_i \right) \right\|^2 + 6\zeta^2 + 2\mathbb{E} \left\| \sum_{i=1}^n p_i g_{k-\tau_k, i} \right\|^2 \right) \\
& = \frac{2n(f(0) - f^*)}{\alpha K} + \frac{2L^2}{K} \sum_{k=0}^{K-1} \mathbb{E} \left\| \frac{(X_k - X_{k-\tau_k}) \mathbb{1}_n}{n} \right\|^2 + \left( 2L^2 + \frac{12\alpha L^3}{n} \right) \frac{1}{K} \sum_{k=0}^{K-1} \sum_{i=1}^n p_i \mathbb{E} \left\| X_{k-\tau_k} \left( \frac{\mathbb{1}_n}{n} - e_i \right) \right\|^2 \\
& + \frac{(\sigma^2 + 6\zeta^2)\alpha L}{n} + \frac{2\alpha L}{nK} \sum_{k=0}^{K-1} \mathbb{E} \left\| \sum_{i=1}^n p_i g_{k-\tau_k, i} \right\|^2
\end{aligned}$$

Note that

$$\mathbb{E} \left\| \sum_{i=1}^n p_i g_{k-\tau_k, i} \right\|^2 = \mathbb{E} \|\nabla \bar{F}(X_{k-\tau_k})\|^2$$

Moving it to the left side, we finally get

$$\begin{aligned}
& \frac{1}{K} \sum_{k=0}^{K-1} \mathbb{E} \|\nabla f(\bar{X}_k)\|^2 + \left( 1 - \frac{2\alpha L}{n} \right) \frac{1}{K} \sum_{k=0}^{K-1} \mathbb{E} \|\nabla \bar{F}(X_{k-\tau_k})\|^2 \\
& \leq \frac{2n(f(0) - f^*)}{\alpha K} + \frac{2L^2}{K} \sum_{k=0}^{K-1} \mathbb{E} \left\| \frac{(X_k - X_{k-\tau_k}) \mathbb{1}_n}{n} \right\|^2 + \left( 2L^2 + \frac{12\alpha L^3}{n} \right) \frac{1}{K} \sum_{k=0}^{K-1} \sum_{i=1}^n p_i \mathbb{E} \left\| X_{k-\tau_k} \left( \frac{\mathbb{1}_n}{n} - e_i \right) \right\|^2 \\
& + \frac{(\sigma^2 + 6\zeta^2)\alpha L}{n}
\end{aligned}$$

That completes the proof.

**Lemma 19** For all  $k \geq 0$ , we have

$$\begin{aligned}
& \frac{2L^2}{K} \sum_{k=0}^{K-1} \mathbb{E} \left\| (X_k - X_{k-\tau_k}) \frac{\mathbb{1}_n}{n} \right\|^2 \\
& \leq \frac{2\alpha^2 T^2 (\sigma^2 + 6\zeta^2) L^2}{n^2} + \frac{24L^4 \alpha^2 T^2}{n^2 K} \sum_{k=0}^{K-1} \sum_{i=1}^n p_i \mathbb{E} \left\| X_{k-\tau_k} \left( \frac{\mathbb{1}_n}{n} - e_i \right) \right\|^2 + \frac{4\alpha^2 T^2 L^2}{n^2 K} \sum_{k=0}^{K-1} \mathbb{E} \left\| \sum_{i=1}^n p_i g_{k-\tau_k, i} \right\|^2
\end{aligned}$$

**Proof** From Lemma 18, we know the fact

$$\bar{X}_{k+1} = X_k W_k \frac{\mathbb{1}_n}{n} + (Q_k - X_k)(W_k - I) \frac{\mathbb{1}_n}{n} - \alpha \widetilde{G}_{k-\tau_k} = \bar{X}_k - \alpha \widetilde{G}_{k-\tau_k}$$

As a result

$$\begin{aligned}
& \sum_{k=0}^{K-1} \mathbb{E} \left\| (X_k - X_{k-\tau_k}) \frac{\mathbb{1}_n}{n} \right\|^2 \\
& = \sum_{k=0}^{K-1} \mathbb{E} \left\| \sum_{t=1}^{\tau_k} \alpha \widetilde{G}_{k-t} \frac{\mathbb{1}_n}{n} \right\|^2 \\
& \leq \alpha^2 \sum_{k=0}^{K-1} \sum_{t=1}^{\tau_k} \mathbb{E} \left\| \widetilde{G}_{k-t} \frac{\mathbb{1}_n}{n} \right\|^2 \\
& \leq \alpha^2 \sum_{k=0}^{K-1} \sum_{t=1}^{\tau_k} \left( \frac{\sigma^2}{n^2} + \frac{1}{n^2} \sum_{i=1}^n p_i \mathbb{E} \|g_{k-t, i}\|^2 \right)
\end{aligned}$$

$$\begin{aligned}
&\leq \frac{\alpha^2 T^2 \sigma^2 K}{n^2} + \frac{\alpha^2 T}{n^2} \sum_{k=0}^{K-1} \sum_{t=1}^{\tau_k} \sum_{i=1}^n p_i \mathbb{E} \|g_{k-t,i}\|^2 \\
&\leq \frac{\alpha^2 T^2 \sigma^2 K}{n^2} + \frac{\alpha^2 T}{n^2} \sum_{k=0}^{K-1} \sum_{t=1}^{\tau_k} \left( 12L^2 \sum_{i=1}^n p_i \mathbb{E} \left\| X_{k-t} \left( \frac{\mathbb{1}_n}{n} - e_i \right) \right\|^2 + 6\varsigma^2 + 2\mathbb{E} \left\| \sum_{i=1}^n p_i g_{k-t,i} \right\|^2 \right) \\
&\leq \frac{\alpha^2 T^2 \sigma^2 K}{n^2} + \frac{\alpha^2 T^2}{n^2} \sum_{k=0}^{K-1} \left( 12L^2 \sum_{i=1}^n p_i \mathbb{E} \left\| X_{k-\tau_k} \left( \frac{\mathbb{1}_n}{n} - e_i \right) \right\|^2 + 6\varsigma^2 + 2\mathbb{E} \left\| \sum_{i=1}^n p_i g_{k-\tau_k,i} \right\|^2 \right) \\
&= \frac{\alpha^2 T^2 (\sigma^2 + 6\varsigma^2) K}{n^2} + \frac{12L^2 \alpha^2 T^2}{n^2} \sum_{k=0}^{K-1} \sum_{i=1}^n p_i \mathbb{E} \left\| X_{k-\tau_k} \left( \frac{\mathbb{1}_n}{n} - e_i \right) \right\|^2 + \frac{2\alpha^2 T^2}{n^2} \sum_{k=0}^{K-1} \mathbb{E} \left\| \sum_{i=1}^n p_i g_{k-\tau_k,i} \right\|^2
\end{aligned}$$

And we get

$$\begin{aligned}
&\frac{2L^2}{K} \sum_{k=0}^{K-1} \mathbb{E} \left\| (X_k - X_{k-\tau_k}) \frac{\mathbb{1}_n}{n} \right\|^2 \\
&\leq \frac{2\alpha^2 T^2 (\sigma^2 + 6\varsigma^2) L^2}{n^2} + \frac{24L^4 \alpha^2 T^2}{n^2 K} \sum_{k=0}^{K-1} \sum_{i=1}^n p_i \mathbb{E} \left\| X_{k-\tau_k} \left( \frac{\mathbb{1}_n}{n} - e_i \right) \right\|^2 + \frac{4\alpha^2 T^2 L^2}{n^2 K} \sum_{k=0}^{K-1} \mathbb{E} \left\| \sum_{i=1}^n p_i g_{k-\tau_k,i} \right\|^2
\end{aligned}$$

That completes the proof.

**Lemma 20** Given non-negative sequences  $\{a_t\}_{t=1}^\infty$ ,  $\{b_t\}_{t=1}^\infty$  and  $\{\tau_t\}_{t=1}^\infty$  and a positive number  $T$  that satisfying

$$a_t = \sum_{s=1}^{t-\tau_t} \rho^{\lfloor \frac{t-\tau_t-s}{T} \rfloor} b_s$$

with  $0 \leq \rho < 1$ , we have

$$\begin{aligned}
S_k &= \sum_{t=1}^k a_t \leq \frac{(2-\rho)T}{1-\rho} \sum_{s=1}^k b_s \\
D_k &= \sum_{t=1}^k a_t^2 \leq \frac{(2-\rho)T^2}{(1-\rho)^2} \sum_{s=1}^k b_s^2
\end{aligned}$$

**Proof**

$$\begin{aligned}
S_k &= \sum_{t=1}^k a_t = \sum_{t=1}^k \sum_{s=1}^{t-\tau_t} \rho^{\lfloor \frac{t-\tau_t-s}{T} \rfloor} b_s \leq \sum_{t=1}^k \sum_{s=1}^t \rho^{\max(\lfloor \frac{t-\tau_t-s}{T} \rfloor, 0)} b_s = \sum_{s=1}^k \sum_{t=s}^k \rho^{\max(\lfloor \frac{t-\tau_t-s}{T} \rfloor, 0)} b_s \\
&= \sum_{s=1}^k \sum_{t=0}^{k-\tau_k-s} \rho^{\lfloor \frac{t}{T} \rfloor} b_s + \sum_{s=1}^k \sum_{t=1}^{\tau_k} \rho^0 b_s \leq \sum_{s=1}^k \left( \sum_{t=0}^{T-1} \sum_{m=0}^{\infty} \rho^m \right) b_s + \tau_k \sum_{s=1}^k b_s \leq \left( T + \frac{T}{1-\rho} \right) \sum_{s=1}^k b_s \\
D_k &= \sum_{t=1}^k a_t^2 = \sum_{t=1}^k \sum_{s=1}^{t-\tau_t} \rho^{\lfloor \frac{t-\tau_t-s}{T} \rfloor} b_s \sum_{r=1}^{t-\tau_t} \rho^{\lfloor \frac{t-\tau_t-r}{T} \rfloor} b_r = \sum_{t=1}^k \sum_{s=1}^{t-\tau_t} \sum_{r=1}^{t-\tau_t} \rho^{\lfloor \frac{t-\tau_t-s}{T} \rfloor + \lfloor \frac{t-\tau_t-r}{T} \rfloor} b_s b_r \\
&\leq \sum_{t=1}^k \sum_{s=1}^{t-\tau_t} \sum_{r=1}^{t-\tau_t} \rho^{\lfloor \frac{t-\tau_t-s}{T} \rfloor + \lfloor \frac{t-\tau_t-r}{T} \rfloor} \frac{b_s^2 + b_r^2}{2} = \sum_{t=1}^k \sum_{s=1}^{t-\tau_t} \sum_{r=1}^{t-\tau_t} \rho^{\lfloor \frac{t-\tau_t-s}{T} \rfloor + \lfloor \frac{t-\tau_t-r}{T} \rfloor} b_s^2 \\
&\leq \sum_{t=1}^k \sum_{s=1}^{t-\tau_t} b_s^2 \rho^{\lfloor \frac{t-\tau_t-s}{T} \rfloor} \sum_{r=1}^{t-\tau_t} \rho^{\lfloor \frac{t-\tau_t-r}{T} \rfloor} \leq \sum_{t=1}^k \sum_{s=1}^{t-\tau_t} b_s^2 \rho^{\lfloor \frac{t-\tau_t-s}{T} \rfloor} \sum_{r=0}^{T-1} \sum_{m=0}^{\infty} \rho^m \\
&\leq \frac{T}{1-\rho} \sum_{t=1}^k \sum_{s=1}^{t-\tau_t} \rho^{\lfloor \frac{t-\tau_t-s}{T} \rfloor} b_s^2 \stackrel{Using S_k}{\leq} \frac{(2-\rho)T^2}{(1-\rho)^2} \sum_{s=1}^k b_s^2
\end{aligned}$$

**Lemma 21** for  $\forall i, j$  and  $\forall k \geq 0$ , we have <sup>9</sup>

$$\|X_k(e_i - e_j)\|_2 \leq \theta = 16t_{\text{mix}}\alpha B$$

**Proof** Similar to Section F and Section G, we use mathematical induction to prove this lemma.

First, for  $k = 0$ , we have

$$\|X_k(e_i - e_j)\|_2 = 0 \leq \theta = 16t_{\text{mix}}\alpha B$$

Now, suppose for  $k \geq 0$ , we have  $\|X_k(e_i - e_j)\|_2 \leq \theta = 16t_{\text{mix}}\alpha B$ , we now prove the case for  $k + 1$ :

$$\begin{aligned} & \|X_{k+1}(e_i - e_j)\|_2 \\ & \leq \left\| X_{k+1} \left( \frac{\mathbb{1}_n}{n} - e_i \right) \right\|_2 + \left\| X_{k+1} \left( \frac{\mathbb{1}_n}{n} - e_j \right) \right\|_2 \\ & \leq \left\| X_{k+1} \left( I - \frac{\mathbb{1}_n \mathbb{1}_n^\top}{n} \right) \right\|_{2 \leftarrow 1} \|e_i\|_1 + \left\| X_{k+1} \left( I - \frac{\mathbb{1}_n \mathbb{1}_n^\top}{n} \right) \right\|_{2 \leftarrow 1} \|e_j\|_1 \\ & = 2 \left\| X_{k+1} \left( I - \frac{\mathbb{1}_n \mathbb{1}_n^\top}{n} \right) \right\|_{2 \leftarrow 1} \\ & \leq 2 \left\| \left( X_k W_k - \alpha \tilde{G}_{k-\tau_k} + \Omega_k \right) \left( \frac{\mathbb{1}_n}{n} - e_i \right) \right\|_{2 \leftarrow 1} \\ & = 2 \left\| \sum_{t=0}^k \left( -\alpha \tilde{G}_{t-\tau_t} + \Omega_t \right) \left( \prod_{q=t+1}^k W_q - \frac{\mathbb{1}_n \mathbb{1}_n^\top}{n} \right) \right\|_{2 \leftarrow 1} \\ & \leq 2 \sum_{t=0}^k \left\| \left( -\alpha \tilde{G}_{t-\tau_t} + \Omega_t \right) \left( \prod_{q=t+1}^k W_q - \frac{\mathbb{1}_n \mathbb{1}_n^\top}{n} \right) \right\|_{2 \leftarrow 1} \\ & \leq 2 \sum_{t=0}^k \left\| -\alpha \tilde{G}_{t-\tau_t} + \Omega_t \right\|_{2 \leftarrow 1} \left\| \prod_{q=t+1}^k W_q - \frac{\mathbb{1}_n \mathbb{1}_n^\top}{n} \right\|_1 \\ & \leq 4(\alpha B + 2\omega\theta) \sum_{t=0}^k 2^{-\lfloor (k-t)/t_{\text{mix}} \rfloor} \\ & \leq 4(\alpha B + 2\omega\theta) \sum_{t=0}^{t_{\text{mix}}-1} \sum_{r=0}^{\infty} 2^{-r} \\ & \leq 8(\alpha B + 2\omega\theta) t_{\text{mix}} \end{aligned}$$

Put in  $\omega = \frac{1}{32t_{\text{mix}}}$ , we obtain

$$\|X_{k+1}(e_i - e_j)\|_2 \leq 8(\alpha B + 2\omega\theta) t_{\text{mix}} = 8t_{\text{mix}}\alpha B + 8t_{\text{mix}}\alpha B = 16t_{\text{mix}}\alpha B$$

And that completes the proof.

---

<sup>9</sup>Since  $\|X_k(e_i - e_j)\|_\infty \leq \|X_k(e_i - e_j)\|_2$  and  $\|X_k(e_i - e_j)\|_2$  is easier to analyze, so we prove  $\|X_k(e_i - e_j)\|_2 \leq \theta$  that will automatically hold for  $\|X_k(e_i - e_j)\|_\infty \leq \theta$ .
