# Supplementary material for: Moniqua: Modulo Quantized Communication in Decentralized SGD
Source: arXiv:2002.11787 source file (2020-06-30)
Supplement: Supplementary file 4 [file backup.tex]

\begin{comment}
\begin{lemma}\label{Async_lemma1}
	\begin{displaymath}
	\mathbb{E}\left\|\frac{\mathbbm{1}_n}{n} - \prod_{k=1}^{K}W_ke_i\right\|^2 \leq \frac{n-1}{n}\rho^K, \forall K \geq 0.
	\end{displaymath}
\end{lemma}\label{Async_lemma1}
\begin{proof}
	Let $y_K = \frac{\mathbbm{1}_n}{n} - \prod\nolimits_{k=1}^{K}W_ke_i$, we have
	\begin{displaymath}
		\begin{split}
		\mathbb{E}\left\|y_{K+1}\right\|^2 & = \mathbb{E}\left\|W_{K+1}y_K\right\|^2\\
		& = \mathbb{E}\langle W_{K+1}y_K, W_{K+1}y_K\rangle\\
		& = \mathbb{E}\langle y_K, W_{K+1}^\top W_{K+1}y_K\rangle\\
		& = \mathbb{E}\langle y_K, \mathbb{E}(W_{K+1}^\top W_{K+1})y_K\rangle
		\end{split}
	\end{displaymath}
	Note that $\mathbb{E}(W_{K+1}^\top W_{K+1})$ is symmetric and doubly stochastic and $\mathbbm{1}_n$ is an eigenvector of $\mathbb{E}(W_{K+1}^\top W_{K+1})$ with eigenvalue 1. Starting from $\mathbbm{1}_n$ we construct a basis of $\mathbb{R}^n$ composed by the eigenvectors of $\mathbb{E}(W_{K+1}^\top W_{K+1})$, which is guaranteed to exist by the spectral theorem of Hermitian matrices. The magnitude of all other eigenvectors' associated eigenvalues should be smaller or equal to $\rho$. Noting $y_K$ is orthogonal to $\mathbbm{1}_n$, we decompose $y_K$ using this constructed basis and it follows that
	\begin{displaymath}
	\mathbb{E}\left\|y_{K+1}\right\|^2 \leq \rho \mathbb{E}\left\|y_{K+1}\right\|^2
	\end{displaymath}
	Note that $\left\|y_0\right\|^2 = \left\|\frac{\mathbbm{1}_n}{n} - e_i\right\|^2 = \frac{(n-1)^2}{n^2} + \sum_{i=1}^{n-1}\frac{1}{n^2} = \frac{n^2 - 2n + 1 + n - 1}{n^2} = \frac{n-1}{n}$
	That completes the proof.
\end{proof}
\end{comment}

\begin{comment}
\begin{lemma}\label{Async_lemma4}
\begin{align*}
    & (1 - 48 L^2\alpha^2\left(T + \bar{\rho}\right))\sum_{k=0}^{K-1}\sum_{i=1}^{n}p_i\mathbb{E}\left\|X_{k-\tau_k}\left(\frac{\mathbbm{1}_n}{n} - e_i\right)\right\|^2\\
    \leq & 4\alpha^2(M\sigma^2 + 6 \varsigma^2)\bar{\rho}K + \frac{4n\alpha\sqrt{d}M\delta \eta\nu}{(1-\sqrt{\rho})^2}\sum_{k=1}^{K-1} \mathbb{E}\left\|\partial\overline{f}(X_{k-\tau_k})\right\| + 8 \alpha^2\left(T + \bar{\rho}\right)\sum_{k=0}^{K-1}\mathbb{E}\left\|\sum_{i=1}^{n}p_ig_{t-\tau_t,i}\right\|^2
    \end{align*}
\end{lemma}
\begin{proof}
\begin{align*}
    & \sum_{k=0}^{K-1}\sum_{i=1}^{n}p_i\mathbb{E}\left\|X_{k-\tau_k}\left(\frac{\mathbbm{1}_n}{n} - e_i\right)\right\|^2\\
    & \overset{Lemma~\ref{Async_lemma5}}{\leq} 4\alpha^2(M\sigma^2 + 6 \varsigma^2)\bar{\rho}K + \frac{4n\alpha\sqrt{d}M\delta \eta\nu}{(1-\sqrt{\rho})^2}\sum_{k=1}^{K-1} \mathbb{E}\left\|\partial\overline{f}(X_{k-\tau_k})\right\|\\
    & + 4 \alpha^2\sum_{k=0}^{K-1}\sum_{t=0}^{k-\tau_k-1}\left(12L^2\sum_{i=1}^{n}p_i\mathbb{E}\left\|X_{t-\tau_t}\left(\frac{\mathbbm{1}_n}{n} - e_i\right)\right\|^2 + 2\mathbb{E}\left\|\sum_{h=1}^{n}p_h\nabla f_h(x^s_{t,h})\right\|^2\right)\left(\rho^{k-\tau_k-t-1} + 2(k-\tau_k-t-1)\rho^{\frac{k-\tau_k-t-1}{2}}\right)\\
    & \leq 4\alpha^2(M\sigma^2 + 6 \varsigma^2)\bar{\rho}K + \frac{4n\alpha\sqrt{d}M\delta \eta\nu}{(1-\sqrt{\rho})^2}\sum_{k=1}^{K-1} \mathbb{E}\left\|\partial\overline{f}(X_{k-\tau_k})\right\|\\
    & + 4 \alpha^2\sum_{k=0}^{K-1}\sum_{t=0}^{k-\tau_k-1}\\
    & \left(12L^2\sum_{i=1}^{n}p_i\mathbb{E}\left\|X_{t-\tau_t}\left(\frac{\mathbbm{1}_n}{n} - e_i\right)\right\|^2 + 2\mathbb{E}\left\|\sum_{h=1}^{n}p_h\nabla f_h(x^s_{t,h})\right\|^2\right)\left(\rho^{\max\{k-\tau_k-t-1, 0\}} + 2(\max\{k-\tau_k-t-1, 0\})\rho^{\frac{\max\{k-\tau_k-t-1, 0\}}{2}}\right)\\
    & \leq 4\alpha^2(M\sigma^2 + 6 \varsigma^2)\bar{\rho}K + \frac{4n\alpha\sqrt{d}M\delta \eta\nu}{(1-\sqrt{\rho})^2}\sum_{k=1}^{K-1} \mathbb{E}\left\|\partial\overline{f}(X_{k-\tau_k})\right\|\\
    & + 4 \alpha^2\sum_{t=0}^{K-1}\\
    & \left(12L^2\sum_{i=1}^{n}p_i\mathbb{E}\left\|X_{t-\tau_t}\left(\frac{\mathbbm{1}_n}{n} - e_i\right)\right\|^2 + 2\mathbb{E}\left\|\sum_{h=1}^{n}p_h\nabla f_h(x^s_{t,h})\right\|^2\right)\sum_{k=t+1}^{\infty}\left(\rho^{\max\{k-\tau_k-t-1, 0\}} + 2(\max\{k-\tau_k-t-1, 0\})\rho^{\frac{\max\{k-\tau_k-t-1, 0\}}{2}}\right)\\
    & \leq 4\alpha^2(M\sigma^2 + 6 \varsigma^2)\bar{\rho}K + \frac{4n\alpha\sqrt{d}M\delta \eta\nu}{(1-\sqrt{\rho})^2}\sum_{k=1}^{K-1} \mathbb{E}\left\|\partial\overline{f}(X_{k-\tau_k})\right\|\\
    & + 2 \alpha^2\sum_{t=0}^{K-1}\left(12L^2\sum_{i=1}^{n}p_i\mathbb{E}\left\|X_{t-\tau_t}\left(\frac{\mathbbm{1}_n}{n} - e_i\right)\right\|^2 + 2\mathbb{E}\left\|\sum_{h=1}^{n}p_h\nabla f_h(x^s_{t,h})\right\|^2\right)\left(T + \sum_{h=0}^{\infty}(\rho^h + 2h\rho^{\frac{h}{2}})\right)\\
    & \leq 4\alpha^2(M\sigma^2 + 6 \varsigma^2)\bar{\rho}K + \frac{4n\alpha\sqrt{d}M\delta \eta\nu}{(1-\sqrt{\rho})^2}\sum_{k=1}^{K-1} \mathbb{E}\left\|\partial\overline{f}(X_{k-\tau_k})\right\|\\
    & + 4 \alpha^2\left(T + \bar{\rho}\right)\sum_{t=0}^{K-1}\left(12L^2\sum_{i=1}^{n}p_i\mathbb{E}\left\|X_{t-\tau_t}\left(\frac{\mathbbm{1}_n}{n} - e_i\right)\right\|^2 + 2\mathbb{E}\left\|\sum_{h=1}^{n}p_h\nabla f_h(x^s_{t,h})\right\|^2\right)\\
    & \leq 4\alpha^2(M\sigma^2 + 6 \varsigma^2)\bar{\rho}K + \frac{4n\alpha\sqrt{d}M\delta \eta\nu}{(1-\sqrt{\rho})^2}\sum_{k=1}^{K-1} \mathbb{E}\left\|\partial\overline{f}(X_{k-\tau_k})\right\|\\
    & + 48 L^2\alpha^2\left(T + \bar{\rho}\right)\sum_{k=0}^{K-1}\mathbb{E}M^s_k + 8 \alpha^2\left(T + \bar{\rho}\right)\sum_{k=0}^{K-1}\mathbb{E}\left\|\sum_{i=1}^{n}p_ig_{t-\tau_t,i}\right\|^2\\
\end{align*}
And we finally have
\begin{displaymath}
\begin{split}
& (1 - 48 L^2\alpha^2\left(T + \bar{\rho}\right))\sum_{k=0}^{K-1}\sum_{i=1}^{n}p_i\mathbb{E}\left\|X_{k-\tau_k}\left(\frac{\mathbbm{1}_n}{n} - e_i\right)\right\|^2\\
\leq & 4\alpha^2(M\sigma^2 + 6 \varsigma^2)\bar{\rho}K + \frac{4n\alpha\sqrt{d}M\delta \eta\nu}{(1-\sqrt{\rho})^2}\sum_{k=1}^{K-1} \mathbb{E}\left\|\partial\overline{f}(X_{k-\tau_k})\right\| + 8 \alpha^2\left(T + \bar{\rho}\right)\sum_{k=0}^{K-1}\mathbb{E}\left\|\sum_{i=1}^{n}p_ig_{t-\tau_t,i}\right\|^2
\end{split}
\end{displaymath}
That completes the proof.
\end{proof}
\end{comment}

\begin{comment}
\begin{lemma}\label{Async_lemma6}
\begin{align*}
    & \alpha^2\mathbb{E}\left\|\sum_{t=0}^{k-1}\widetilde{G}_{t-\tau_t}\Lambda_{t+1}^{k-1}e_i\right\|^2\\
    \leq & 2\alpha^2(M\sigma^2 + 6 \varsigma^2)\bar{\rho} + 2 \alpha^2\sum_{t=0}^{k-1}\left(12L^2\sum_{i=1}^{n}p_i\mathbb{E}\left\|X_{t-\tau_t}\left(\frac{\mathbbm{1}_n}{n} - e_i\right)\right\|^2 + 2\mathbb{E}\left\|\sum_{h=1}^{n}p_h\nabla f_h(x^s_{t,h})\right\|^2\right)\left(\rho^{k-t-1} + 2(k-t-1)\rho^{\frac{k-t-1}{2}}\right)
    \end{align*}
\end{lemma}
\begin{proof}
Note that
\begin{align*}
    &\mathbb{E}\left\|\sum_{t=0}^{k-1}\widetilde{G}_{t-\tau_t}\Lambda_{t+1}^{k-1}e_i\right\|^2\\
    = &\mathbb{E}\left\|\sum_{t=0}^{k-1}\left(\widetilde{G}_{t-\tau_t} - G_{t-\tau_t}\right)\Lambda_{t+1}^{k-1}e_i\right\|^2 + \mathbb{E}\left\|\sum_{t=0}^{k-1}G_{t-\tau_t}\Lambda_{t+1}^{k-1}e_i\right\|^2
    \end{align*}
Let $A_1$ denote the first term and $A_2$ denote the second term. And now let $\Lambda_{a}^{b} = \frac{\mathbbm{1}_n\mathbbm{1}_n^\top}{n} - \prod_{q=a}^{b}W_q$, we first analyze $A_1$:
\begin{align*}
    &\mathbb{E}\left\|\sum_{t=0}^{k-1}\left(\widetilde{G}_{t-\tau_t} - G_{t-\tau_t}\right)\Lambda_{t+1}^{k-1}e_i\right\|^2\\
    = &\sum_{t=0}^{k-1}\mathbb{E}\left\|\left(\widetilde{G}_{t-\tau_t} - G_{t-\tau_t}\right)\Lambda_{t+1}^{k-1}e_i\right\|^2 + \sum_{k\geq t>t^{'}\geq 0}\left\langle\left(\widetilde{G}_{t-\tau_t} - G_{t-\tau_t}\right)\Lambda_{t+1}^{k-1}e_i, \widetilde{G}_{s(t^{'})} - G_{s(t^{'})}\Lambda_{t^{'}+1}^{k-1}e_i\right\rangle\\
    \leq & \sum_{t=0}^{k-1}\mathbb{E}\left\|\left(\widetilde{G}_{t-\tau_t} - G_{t-\tau_t}\right)\Lambda_{t+1}^{k-1}\right\|^2 + \sum_{k\geq t>t^{'}\geq 0}\mathbb{E}\left\|\widetilde{G}_{t-\tau_t} - G_{t-\tau_t}\right\|\left\|\Lambda_{t+1}^{k-1}e_i\right\|\left\|\widetilde{G}_{s(t^{'})} - G_{s(t^{'})}\right\|\left\|\Lambda_{t^{'}+1}^{k-1}e_i\right\|\\
    \leq & \sum_{t=0}^{k-1}\mathbb{E}\left\|\widetilde{G}_{t-\tau_t} - G_{t-\tau_t}\right\|^2\left\|\Lambda_{t+1}^{k-1}\right\|^2 + \sum_{k\geq t>t^{'}\geq 0}\mathbb{E}\left(\frac{\left\|\Lambda_{t+1}^{k-1}e_i\right\|^2\left\|\Lambda_{t^{'}+1}^{k-1}e_i\right\|^2}{2\gamma_{t,t^{'}}} + \frac{\left\|\widetilde{G}_{t-\tau_t} - G_{t-\tau_t}\right\|^2\left\|\widetilde{G}_{s(t^{'})} - G_{s(t^{'})}\right\|^2}{2/\gamma_{t,t^{'}}}\right)\\
    \leq & \sum_{t=0}^{k-1}\mathbb{E}\left\|\widetilde{G}_{t-\tau_t} - G_{t-\tau_t}\right\|^2\rho^{k-t} + \sum_{k\geq t>t^{'}\geq 0}\mathbb{E}\left(\frac{\left\|\Lambda_{t^{'}+1}^{k-1}e_i\right\|^2}{2\gamma_{t,t^{'}}} + \frac{\sigma^4}{2/\gamma_{t,t^{'}}}\right)\\
    \leq & \sigma^2\sum_{t=0}^{k-1}\rho^{k-t} + \sum_{k\geq t>t^{'}\geq 0}\mathbb{E}\left(\frac{\rho^{k-t^{'}-1}}{2\gamma_{t,t^{'}}} + \frac{\sigma^4}{2/\gamma_{t,t^{'}}}\right)\\
    \leq & \frac{\sigma^2}{1-\rho} + \sum^k_{k\geq t>t^{'}\geq 0}\rho^{\frac{k-t^{'}-1}{2}}\sigma^2\\
    \leq & \left(\frac{1}{1-\rho} + \frac{2\sqrt{\rho}}{(1-\sqrt{\rho})^2}\right)\sigma^2\\
    \leq & \sigma^2\bar{\rho}
    \end{align*}
For $A_2$, we have
\begin{align*}
    &\mathbb{E}\left\|\sum_{t=0}^{k-1}G_{t-\tau_t}\Lambda_{t+1}^{k-1}e_i\right\|^2\\
    = & \sum_{t=0}^{k-1}\mathbb{E}\left\|G_{t-\tau_t}\Lambda_{t+1}^{k-1}e_i\right\|^2 + 2\mathbb{E}\sum_{t=0}^{k-1}\sum_{t^{'}=t+1}^{k-1}\left\langle G_{t-\tau_t}\Lambda_{t+1}^{k-1}e_i, G_{s(t^{'})}\Lambda_{t^{'}+1}^{k-1}e_i\right\rangle\\
    \leq & \sum_{t=0}^{k-1}\mathbb{E}\left(\sum_{i=1}^{n}p_i\left\|g_{t-\tau_t,i}\right\|^2\right)\rho^{k-t-1} + 2\mathbb{E}\sum_{t=0}^{k-1}\sum_{t^{'}=t+1}^{k-1}\left\|G_{t-\tau_t}\right\|\left\|\Lambda_{t+1}^{k-1}e_i\right\|\left\|G_{s(t^{'})}\right\|\left\|\Lambda_{t^{'}+1}^{k-1}e_i\right\|
\end{align*}
For the second term, we have
\begin{align*}
    & \mathbb{E}\sum_{t=0}^{k-1}\sum_{t^{'}=t+1}^{k-1}\left\|G_{t-\tau_t}\right\|\left\|\Lambda_{t+1}^{k-1}e_i\right\|\left\|G_{s(t^{'})}\right\|\left\|\Lambda_{t^{'}+1}^{k-1}e_i\right\|\\
    \leq & \mathbb{E}\sum_{t=0}^{k-1}\sum_{t^{'}=t+1}^{k-1}\left(\frac{\left\|G_{t-\tau_t}\right\|^2\left\|G_{s(t^{'})}\right\|^2}{2\gamma_{t,t^{'}}} + \frac{\left\|\Lambda_{t+1}^{k-1}e_i\right\|^2\left\|\Lambda_{t^{'}+1}^{k-1}e_i\right\|^2}{2/\gamma_{t,t^{'}}}\right)\\
    \leq & \frac{1}{2}\mathbb{E}\sum_{t\neq t^{'}}^{k-1}\left(\frac{\left\|G_{t-\tau_t}\right\|^2\left\|G_{s(t^{'})}\right\|^2}{2\gamma_{t,t^{'}}} + \frac{\rho^{k-\min\{t,t^{'}\}-1}}{2/\gamma_{t,t^{'}}}\right)\\
    \leq & \frac{1}{2}\mathbb{E}\sum_{t\neq t^{'}}^{k-1}\left(\left\|G_{t-\tau_t}\right\|\left\|G_{s(t^{'})}\right\|\rho^{\frac{k-\min\{t,t^{'}\}-1}{2}}\right)\\
    \leq & \frac{1}{2}\mathbb{E}\sum_{t\neq t^{'}}^{k-1}\left(\frac{\left\|G_{t-\tau_t}\right\|^2 + \left\|G_{s(t^{'})}\right\|^2}{2}\rho^{\frac{k-\min\{t,t^{'}\}-1}{2}}\right)\\
    = & \frac{1}{2}\mathbb{E}\sum_{t\neq t^{'}}^{k-1}\left(\left\|G_{t-\tau_t}\right\|^2\rho^{\frac{k-\min\{t,t^{'}\}-1}{2}}\right)\\
    = & \sum_{t=0}^{k-1}\sum_{t^{'}=t+1}^{k-1}\left(\mathbb{E}\left\|G_{t-\tau_t}\right\|^2\rho^{\frac{k-t-1}{2}}\right)\\
    = & \sum_{t=0}^{k-1}\left(\sum_{i=1}^{n}p_i\mathbb{E}\left\|g_{t-\tau_t,i}\right\|^2\right)(k-t-1)\rho^{\frac{k-t-1}{2}}
    \end{align*}
Putting it back to $A_2$, we obtain
\begin{align*}
    A_2 & = \sum_{t=0}^{k-1}\left(\sum_{i=1}^{n}p_i\mathbb{E}\left\|g_{t-\tau_t,i}\right\|^2\right)\left(\rho^{k-t-1} + 2(k-t-1)\rho^{\frac{k-t-2}{2}}\right)\\
    & \leq \sum_{t=0}^{k-1}\left(12L^2\sum_{i=1}^{n}p_i\mathbb{E}\left\|X_{t-\tau_t}\left(\frac{\mathbbm{1}_n}{n} - e_i\right)\right\|^2 + 6\varsigma^2 + 2\mathbb{E}\left\|\sum_{h=1}^{n}p_h\nabla f_h(x^s_{t,h})\right\|^2\right)\left(\rho^{k-t-1} + 2(k-t-1)\rho^{\frac{k-t-1}{2}}\right)\\
    & \leq \sum_{t=0}^{k-1}\left(12L^2\sum_{i=1}^{n}p_i\mathbb{E}\left\|X_{t-\tau_t}\left(\frac{\mathbbm{1}_n}{n} - e_i\right)\right\|^2 + 2\mathbb{E}\left\|\sum_{h=1}^{n}p_h\nabla f_h(x^s_{t,h})\right\|^2\right)\left(\rho^{k-t-1} + 2(k-t-1)\rho^{\frac{k-t-1}{2}}\right) + 6\varsigma^2\bar{\rho}
    \end{align*}
Putting it back, we have
\begin{align*}
    & \alpha^2\mathbb{E}\left\|\sum_{t=0}^{k-1}\widetilde{G}_{t-\tau_t}\Lambda_{t+1}^{k-1}e_i\right\|^2\\
    = & \alpha^2A_1 + \alpha^2A_2\\
    \leq & \alpha^2(\sigma^2 + 6\varsigma^2)\bar{\rho} + \alpha^2\sum_{t=0}^{k-1}\left(12L^2\sum_{i=1}^{n}p_i\mathbb{E}\left\|X_{t-\tau_t}\left(\frac{\mathbbm{1}_n}{n} - e_i\right)\right\|^2 + 2\mathbb{E}\left\|\sum_{h=1}^{n}p_h\nabla f_h(x^s_{t,h})\right\|^2\right)\\
    \times & \left(\rho^{k-t-1} + 2(k-t-1)\rho^{\frac{k-t-1}{2}}\right)
\end{align*}
As a result
\begin{align*}
    & 2\alpha^2\sum_{k=1}^{K-1}\sum_{i=1}^{n}p_i\mathbb{E}\left\|\sum_{t=0}^{k-1}\widetilde{G}_{t-\tau_t}\Lambda_{t+1}^{k-1}e_i\right\|^2\\
    \leq & 2\alpha^2(\sigma^2 + 6\varsigma^2)\bar{\rho}K + \alpha^2\sum_{t=0}^{k-1}\left(12L^2\sum_{i=1}^{n}p_i\mathbb{E}\left\|X_{t-\tau_t}\left(\frac{\mathbbm{1}_n}{n} - e_i\right)\right\|^2 + 2\mathbb{E}\left\|\sum_{h=1}^{n}p_h\nabla f_h(x^s_{t,h})\right\|^2\right)\\
    \times & \left(\rho^{k-t-1} + 2(k-t-1)\rho^{\frac{k-t-1}{2}}\right)
\end{align*}
\end{proof}
\end{comment}
