# Supplementary material for: Moniqua: Modulo Quantized Communication in Decentralized SGD
Source: arXiv:2002.11787 source file (2020-06-30)
Supplement: Supplementary file 5 [file experiments.tex]

\section{More Experimental Results}\label{experiments}
\iffalse
\subsection{Compute Number of Bits}
In Experiment of \emph{Efficient Moniqua}, we calculate the number of bits in the following way: First, we calculate the total number of bits each worker send out, sum them up and divided by number of epochs, and we get the average bandwidth consumption $\overline{BW}$ of the whole system in each epoch. Then we compute the number of bits required for each number in the following way (note that every worker has 2 neighbors in a ring topology):
\begin{align*}
\#bits=\frac{\overline{BW}}{\text{\#neighbors}\cdot\text{\#workers}\cdot\text{\#params of model}}
\end{align*}
In our experiments, \text{\#neighbors}=2, \text{\#workers}=8. For VGG16, \text{\#params of model}= 15,245,130 while for ResNet110, \text{\#params of model}=1,146,842. We formalize the results in Table~\ref{exp Quantization step} \footnote{Note that we only put results that's 'close to the limit of Moniqua' here}.

\begin{table}[h]
\label{exp time}
\caption{Wall Clock Time consumption (Seconds)/Epoch in average under different network in Experiment of Evaluation of Moniqua.}
\begin{center}
\begin{tabular}{c|c|c|c|c}
\toprule
& 100mbps/0.15ms &  20mbps/0.15ms & 100mbps/10ms & Extra Memory\\
\midrule
Centralized & $38.92$ & $206.14$ & $343.28$ & N/A \\
\midrule
D-PSGD      & $36.25$ & $189.48$ & $310.98$ & N/A \\
\midrule
DCD-PSGD    & $32.99$ & $105.40$ & $202.42$ & $20.4$ MB \\
\midrule
ECD-PSGD    & $31.96$ & $105.26$ & $202.04$ & $20.4$ MB \\
\midrule
ChocoSGD    & $32.03$ & $105.18$ & $201.18$ & $20.4$ MB \\
\midrule
DeepSqueeze & $30.01$ & $103.67$ & $193.92$ & $13.6$ MB \\
\midrule
Moniqua     & \textbf{$22.42$} & \textbf{$95.08$}  & \textbf{$184.86$} & $0$ B\\
\bottomrule
\end{tabular}
\end{center}
\end{table}

\begin{table}[t]
\label{exp Quantization step}
\caption{Bandwidth consumption under different $\theta$ and $\delta$ when applying linear quantizer in Moniqua}
\begin{center}
\begin{small}
\begin{sc}
\begin{tabular}{c|c|c|c|c}
\toprule
Model  & Mod Param $\theta$ & Quant Step & Bytes/Epoch & Avg Bits\\
\midrule
\multirow{3}{*}{VGG16} 
& None   & None   & 45594MB  & 32   \\ 
& $1.0$  & $0.01$ & 5206MB   & 3.65 \\
& $0.08$  & $0.01$ & 5192MB   & 3.64 \\
\midrule
\multirow{3}{*}{ResNet110} 
& None   & None   & 3430MB  & 32    \\  
& $2.0$  & $0.01$ & 609MB   & 5.67  \\
& $1.3$  & $0.01$ & 608MB   & 5.67  \\
\bottomrule
\end{tabular}
\end{sc}
\end{small}
\end{center}
\end{table}
\fi

\subsection{Various Quantizers}
In this section, we will verify Moniqua is applicable to other quantizers aside from linear quantizer as shown in the paper. We test it on two more quantizers:
\begin{enumerate}
    \item \textbf{Nearest Rounding (Biased)}
    \begin{align*}
    \mathcal{Q}(x) = \delta\left\lfloor\frac{x}{\delta} + 0.5\right\rfloor
    \end{align*}
    where $\delta$ is the quantization step as defined in the linear quantizer. In this experiment, we set $\delta=0.01$, the same value as we used in the paper with stochastic rounding.
    \item \textbf{Randomized Gossip (Non-linear)}
    \begin{align*}
    \mathcal{Q}(x)= & \begin{cases} x, &\text{with probability}\hspace{1em}p \cr  0, &\text{with probability}\hspace{1em} 1-p\end{cases}
    \end{align*}
    In this experiment, we set $p=0.7$.
\end{enumerate}

We train ResNet110 on CIFAR10, and plot the results in Figure~\ref{expquantizer}. We can see that the training curves of using three quantizers are all aligned with D-PSGD with full-precision communication. Note that in the paper we show that previous work cannot perserve the aligned curve even with stochastic rounding (unbiased), thus we are not comparing them here.

\subsection{More results on different hyperparameters}
In this experiment, we plot more result of training ResNet110 and VGG16 on CIFAR10 under different $\delta$ and $\theta$ in the experiment of aggressive quantization. And we plot the results in Figure~\ref{expmoreVGG} and Figure~\ref{expmoreResNet}.


\begin{figure}[h!]
\subfigure[Performance of Moniqua on VGG16 under different $\theta$ and $\delta$]{
    \includegraphics[width=0.3\textwidth]{./section/appendix/Figures/more_VGG.pdf}
    \label{expmoreVGG}
    }
\subfigure[Performance of Moniqua on ResNet110 under different $\theta$ and $\delta$]{
    \includegraphics[width=0.3\textwidth]{./section/appendix/Figures/more_ResNet.pdf}
    \label{expmoreResNet}
    }
\subfigure[Performance of algorithms under different quantizer]{
    \includegraphics[width=0.3\textwidth]{./section/appendix/Figures/biased_quantizer.pdf}
    \label{expquantizer}
    }
\end{figure}
